# Supplementary material for: Comprehensive Empirical Evaluation of Deep Learning Approaches for Session-based Recommendation in E-Commerce
Source: arXiv:2010.12540 source file (2020-10-17)
Supplement: Supplementary file 1 [file tab1.tex]

\begin{table*}[!h]
\centering
\caption{RQ1: training using long sessions of Length \textgreater = 10}
\resizebox{0.9\textwidth}{!}{\begin{tabular}{|c|ccccc|ccccc|}
\hline
\cellcolor[HTML]{333333}{\color[HTML]{FFFFFF} } &
  \multicolumn{5}{c|}{\textbf{HR@}} &
  \multicolumn{5}{c|}{\textbf{MRR@}} \\ \cline{2-11} 
\multirow{-2}{*}{\cellcolor[HTML]{333333}{\color[HTML]{FFFFFF} \textbf{RECSYS}}} &
  \textbf{1} &
  \textbf{3} &
  \textbf{5} &
  \textbf{10} &
  \textbf{20} &
  \textbf{1} &
  \textbf{3} &
  \textbf{5} &
  \textbf{10} &
  \textbf{20} \\ \hline
\textbf{S-POP} &
  0.0352 &
  0.09716 &
  0.12179 &
  0.14178 &
  0.15211 &
  0.0352 &
  0.06234 &
  0.068 &
  0.07079 &
  0.07155 \\
\textbf{AR} &
  0.10075 &
  0.20169 &
  0.26112 &
  0.32715 &
  0.32753 &
  0.10075 &
  0.14431 &
  0.15784 &
  0.16723 &
  0.16726 \\
\textbf{SR} &
  0.10515 &
  0.20555 &
  0.26726 &
  0.35955 &
  0.45141 &
  0.10515 &
  0.1487 &
  0.16272 &
  0.17501 &
  0.18138 \\
\textbf{VSKNN} &
  0.10519 & 0.19934 & 0.24868 & 0.32591 & 0.40670 & 0.10519 & 0.14624 & 0.15752 & 0.16771 & 0.17332 \\
\textbf{SMF} &
  0.06302 &
  0.19325 &
  0.27855 &
  0.40556 &
  0.53415 &
  0.06302 &
  0.11895 &
  0.13823 &
  0.15515 &
  0.16412 \\
\textbf{Item2Vec} &
  0.07978 &
  0.16408 &
  0.21602 &
  0.30968 &
  0.40933 &
  0.07978 &
  0.1162 &
  0.12798 &
  0.14036 &
  0.14723 \\
\textbf{GRU4Rec+} &
  0.07194 &
  0.18834 &
  0.26708 &
  0.39639 &
  0.5294 &
  0.07194 &
  0.12141 &
  0.13923 &
  0.1564 &
  0.1657 \\
\textbf{NARM} &
  0.08484 &
  0.19574 &
  0.25034 &
  0.40034 &
  0.59822 &
  0.08484 &
  0.13275 &
  0.15833 &
  0.16492 &
  0.17078 \\
\textbf{STAMP} &
  0.11954 &
  0.24778 &
  0.32518 &
  0.44541 &
  0.5667 &
  0.11954 &
  0.17488 &
  0.19246 &
  0.2085 &
  0.21698 \\
\textbf{NextItNet} &
  0.16772 &
  0.32224 &
  0.40444 &
  0.51027 &
  0.61013 &
  0.16772 &
  0.2342 &
  0.25296 &
  0.26713 &
  0.27412 \\
\textbf{SRGNN} &
  0.12919 &
  0.26245 &
  0.34709 &
  0.46792 &
  0.59104 &
  0.12919 &
  0.18675 &
  0.20599 &
  0.22207 &
  0.2307 \\
\textbf{CSRM} &
  0.1512 &
  0.29975 &
  0.38993 &
  0.53247 &
  0.66373 &
  0.1512 &
  0.21527 &
  0.23569 &
  0.25465 &
  0.26387 \\ \hline
\cellcolor[HTML]{333333}{\color[HTML]{FFFFFF} } &
  \multicolumn{5}{c|}{\textbf{HR@}} &
  \multicolumn{5}{c|}{\textbf{MRR@}} \\ \cline{2-11} 
\multirow{-2}{*}{\cellcolor[HTML]{333333}{\color[HTML]{FFFFFF} \textbf{CIKMCUP}}} &
  \textbf{1} &
  \textbf{3} &
  \textbf{5} &
  \textbf{10} &
  \textbf{20} &
  \textbf{1} &
  \textbf{3} &
  \textbf{5} &
  \textbf{10} &
  \textbf{20} \\ \hline
\textbf{S-POP} &
  0.03831 &
  0.09682 &
  0.11394 &
  0.1286 &
  0.13304 &
  0.03831 &
  0.06391 &
  0.06793 &
  0.07002 &
  0.07033 \\
\textbf{AR} &
  0.03695 &
  0.08795 &
  0.127 &
  0.1812 &
  0.18145 &
  0.03695 &
  0.05894 &
  0.06782 &
  0.07531 &
  0.07533 \\
\textbf{SR} &
  0.03227 &
  0.08303 &
  0.1169 &
  0.1679 &
  0.22838 &
  0.03227 &
  0.05408 &
  0.06181 &
  0.06862 &
  0.07291 \\
\textbf{VSKNN} &
  0.05640 & 0.11438 & 0.14978 & 0.21236 & 0.26854 & 0.05640 & 0.08157 & 0.08961 & 0.09790 & 0.10180 \\
\textbf{SMF} &
  0.03375 &
  0.08463 &
  0.1307 &
  0.212 &
  0.31523 &
  0.03375 &
  0.05475 &
  0.06515 &
  0.07588 &
  0.08293 \\
\textbf{Item2Vec} &
  0.01383 &
  0.03335 &
  0.04657 &
  0.0788 &
  0.12327 &
  0.01383 &
  0.02203 &
  0.02499 &
  0.02931 &
  0.0323 \\
\textbf{GRU4Rec+} &
  0.02169 &
  0.05538 &
  0.08062 &
  0.13698 &
  0.2111 &
  0.02169 &
  0.03598 &
  0.0417 &
  0.04918 &
  0.05421 \\
\textbf{NARM} &
  0.04436 &
  0.10479 &
  0.14416 &
  0.22199 &
  0.40159 &
  0.04436 &
  0.06993 &
  0.07892 &
  0.08922 &
  0.09945 \\
\textbf{STAMP} &
  0.02834 &
  0.07996 &
  0.12024 &
  0.20623 &
  0.31588 &
  0.02834 &
  0.05 &
  0.05912 &
  0.07044 &
  0.07793 \\
\textbf{NextItNet} &
  0.0142 &
  0.03456 &
  0.05682 &
  0.09138 &
  0.1392 &
  0.0142 &
  0.02281 &
  0.02778 &
  0.03224 &
  0.03552 \\
\textbf{SRGNN} &
  0.03845 &
  0.09863 &
  0.14709 &
  0.23669 &
  0.34167 &
  0.03845 &
  0.06396 &
  0.07491 &
  0.08688 &
  0.09413 \\
\textbf{CSRM} &
  0.03953 &
  0.09524 &
  0.14169 &
  0.21828 &
  0.32563 &
  0.03953 &
  0.06325 &
  0.07384 &
  0.08398 &
  0.09139 \\ \hline
\cellcolor[HTML]{333333}{\color[HTML]{FFFFFF} } &
  \multicolumn{5}{c|}{\textbf{HR@}} &
  \multicolumn{5}{c|}{\textbf{MRR@}} \\ \cline{2-11} 
\multirow{-2}{*}{\cellcolor[HTML]{333333}{\color[HTML]{FFFFFF} \textbf{TMALL}}} &
  \textbf{1} &
  \textbf{3} &
  \textbf{5} &
  \textbf{10} &
  \textbf{20} &
  \textbf{1} &
  \textbf{3} &
  \textbf{5} &
  \textbf{10} &
  \textbf{20} \\ \hline
\textbf{S-POP} &
  0.04398 &
  0.10146 &
  0.13027 &
  0.16264 &
  0.18323 &
  0.04398 &
  0.06891 &
  0.07551 &
  0.0799 &
  0.08139 \\
\textbf{AR} &
  0.01403 &
  0.02968 &
  0.04016 &
  0.05445 &
  0.05503 &
  0.01403 &
  0.02071 &
  0.02309 &
  0.02509 &
  0.02512 \\
\textbf{SR} &
  0.01397 &
  0.02838 &
  0.03799 &
  0.05288 &
  0.06929 &
  0.01397 &
  0.02013 &
  0.02231 &
  0.02429 &
  0.02544 \\
\textbf{VSKNN} &
  0.02439 & 0.03710 & 0.04448 & 0.05826 & 0.07304 & 0.02439 & 0.02974 & 0.03167 & 0.03325 & 0.03456 \\
\textbf{SMF} &
  0.01307 &
  0.03366 &
  0.03869 &
  0.06232 &
  0.0888 &
  0.01307 &
  0.02745 &
  0.02905 &
  0.04033 &
  0.04269 \\
\textbf{Item2Vec} &
  0.00256 &
  0.00567 &
  0.00769 &
  0.01227 &
  0.01974 &
  0.00256 &
  0.00386 &
  0.00431 &
  0.00491 &
  0.00541 \\
\textbf{GRU4Rec+} &
  0.03536 &
  0.06745 &
  0.08644 &
  0.11675 &
  0.14992 &
  0.03536 &
  0.04922 &
  0.05352 &
  0.05753 &
  0.05982 \\
\textbf{NARM} &
  0.05701 &
  0.10647 &
  0.12878 &
  0.16514 &
  0.25595 &
  0.05701 &
  0.07795 &
  0.08264 &
  0.08663 &
  0.09185 \\
\textbf{STAMP} &
  0.03286 &
  0.06537 &
  0.08406 &
  0.11384 &
  0.14941 &
  0.03286 &
  0.04688 &
  0.05112 &
  0.05509 &
  0.05755 \\
\textbf{NextItNet} &
  0.013 &
  0.035 &
  0.0542 &
  0.07143 &
  0.09966 &
  0.013 &
  0.03147 &
  0.03585 &
  0.03936 &
  0.04129 \\
\textbf{SRGNN} &
  0.03855 &
  0.0779 &
  0.09892 &
  0.13229 &
  0.16993 &
  0.03855 &
  0.05542 &
  0.0602 &
  0.06468 &
  0.06729 \\
\textbf{CSRM} &
  0.03716 &
  0.07753 &
  0.10122 &
  0.13871 &
  0.18382 &
  0.03716 &
  0.05448 &
  0.05988 &
  0.06484 &
  0.06796 \\ \hline
\cellcolor[HTML]{333333}{\color[HTML]{FFFFFF} } &
  \multicolumn{5}{c|}{\textbf{HR@}} &
  \multicolumn{5}{c|}{\textbf{MRR@}} \\ \cline{2-11} 
\multirow{-2}{*}{\cellcolor[HTML]{333333}{\color[HTML]{FFFFFF} \textbf{ROCKET}}} &
  \textbf{1} &
  \textbf{3} &
  \textbf{5} &
  \textbf{10} &
  \textbf{20} &
  \textbf{1} &
  \textbf{3} &
  \textbf{5} &
  \textbf{10} &
  \textbf{20} \\ \hline
\textbf{S-POP} &
  0.04006 &
  0.11733 &
  0.13085 &
  0.14672 &
  0.15271 &
  0.04006 &
  0.07514 &
  0.07821 &
  0.08041 &
  0.08082 \\
\textbf{AR} &
  0.0281 &
  0.06504 &
  0.08871 &
  0.12123 &
  0.12175 &
  0.0281 &
  0.04379 &
  0.04915 &
  0.0536 &
  0.05363 \\
\textbf{SR} &
  0.03122 &
  0.0705 &
  0.09365 &
  0.12643 &
  0.15557 &
  0.03122 &
  0.04782 &
  0.05296 &
  0.05742 &
  0.0594 \\
\textbf{VSKNN} &
  0.11666 & 0.17283 & 0.20050 & 0.24840 & 0.29155 & 0.11666 & 0.14123 & 0.14760 & 0.15396 & 0.15696 \\
\textbf{SMF} &
  0.0307 &
  0.0744 &
  0.10432 &
  0.15453 &
  0.20786 &
  0.0307 &
  0.04908 &
  0.05583 &
  0.06229 &
  0.06601 \\
\textbf{Item2Vec} &
  0.01788 &
  0.03344 &
  0.04536 &
  0.06791 &
  0.10394 &
  0.01788 &
  0.02467 &
  0.02738 &
  0.03035 &
  0.0328 \\
\textbf{GRU4Rec+} &
  0.02438 &
  0.04824 &
  0.06406 &
  0.09232 &
  0.11852 &
  0.02438 &
  0.03453 &
  0.03817 &
  0.04198 &
  0.04379 \\
\textbf{NARM} &
  0.08869 &
  0.17132 &
  0.2162 &
  0.27816 &
  0.38009 &
  0.08869 &
  0.12412 &
  0.13416 &
  0.14264 &
  0.14936 \\
\textbf{STAMP} &
  0.02381 &
  0.07561 &
  0.10178 &
  0.14887 &
  0.19519 &
  0.02381 &
  0.04622 &
  0.05202 &
  0.05833 &
  0.06148 \\
\textbf{NextItNet} &
  0.00305 &
  0.00762 &
  0.01296 &
  0.02058 &
  0.03125 &
  0.00305 &
  0.00495 &
  0.00614 &
  0.00717 &
  0.00791 \\
\textbf{SRGNN} &
  0.04688 &
  0.09879 &
  0.12954 &
  0.17364 &
  0.21976 &
  0.04688 &
  0.06901 &
  0.0759 &
  0.08195 &
  0.08511 \\
\textbf{CSRM} &
  0.0331 &
  0.09465 &
  0.13085 &
  0.19033 &
  0.25032 &
  0.0331 &
  0.05892 &
  0.06709 &
  0.07511 &
  0.07926 \\ \hline
\end{tabular}}
\label{tab:train-long}
\end{table*}
