# Supplementary material for: Comprehensive Empirical Evaluation of Deep Learning Approaches for Session-based Recommendation in E-Commerce
Source: arXiv:2010.12540 source file (2020-10-17)
Supplement: Supplementary file 2 [file tab10.tex]

\begin{table*}[!h]
\centering
\caption{RQ6: training using sessions of the most recent 2 days before the testing set.}
\resizebox{0.9\textwidth}{!}{\begin{tabular}{|c|ccccc|ccccc|}
\hline
\cellcolor[HTML]{333333}{\color[HTML]{FFFFFF} } &
  \multicolumn{5}{c|}{\textbf{HR@}} &
  \multicolumn{5}{c|}{\textbf{MRR@}} \\ \cline{2-11} 
\multirow{-2}{*}{\cellcolor[HTML]{333333}{\color[HTML]{FFFFFF} \textbf{RECSYS}}} &
  \textbf{1} &
  \textbf{3} &
  \textbf{5} &
  \textbf{10} &
  \textbf{20} &
  \textbf{1} &
  \textbf{3} &
  \textbf{5} &
  \textbf{10} &
  \textbf{20} \\ \hline
\textbf{S-POP} &
  0.03878 &
  0.10347 &
  0.13353 &
  0.16989 &
  0.19284 &
  0.03878 &
  0.06714 &
  0.07388 &
  0.07897 &
  0.08046 \\
\textbf{AR} &
  0.11896 &
  0.2291 &
  0.29183 &
  0.36038 &
  0.36248 &
  0.11896 &
  0.1665 &
  0.18077 &
  0.19054 &
  0.19069 \\
\textbf{SR} &
  0.03317 &
  0.07453 &
  0.10015 &
  0.1308 &
  0.15033 &
  0.03317 &
  0.05063 &
  0.05643 &
  0.06059 &
  0.06195 \\
\textbf{VSKNN} &
  0.11579 & 0.23588 & 0.30713 & 0.37928 & 0.45404 & 0.11337 & 0.16450 & 0.17618 & 0.18374 & 0.19069 \\
\textbf{SMF} &
  0.0802 &
  0.20197 &
  0.28808 &
  0.42532 &
  0.54642 &
  0.0802 &
  0.13205 &
  0.15163 &
  0.16995 &
  0.17844 \\
\textbf{Item2Vec} &
  0.07054 &
  0.13467 &
  0.1744 &
  0.24192 &
  0.32925 &
  0.07054 &
  0.09821 &
  0.10721 &
  0.11614 &
  0.1222 \\
\textbf{GRU4Rec+} &
  0.07242 &
  0.17118 &
  0.24186 &
  0.36148 &
  0.48687 &
  0.07242 &
  0.11438 &
  0.13034 &
  0.14618 &
  0.15493 \\
\textbf{NARM} &
  0.11652 &
  0.28302 &
  0.37549 &
  0.51916 &
  0.69631 &
  0.11652 &
  0.18848 &
  0.20959 &
  0.22868 &
  0.23966 \\
\textbf{STAMP} &
  0.12941 &
  0.26419 &
  0.34461 &
  0.46388 &
  0.59013 &
  0.12941 &
  0.18737 &
  0.20564 &
  0.2215 &
  0.23028 \\
\textbf{NextItNet} &
  0.16389 &
  0.3125 &
  0.38438 &
  0.48963 &
  0.59443 &
  0.16389 &
  0.22847 &
  0.24487 &
  0.25879 &
  0.2662 \\
\textbf{SRGNN} &
  0.135 &
  0.2769 &
  0.357 &
  0.4826 &
  0.60737 &
  0.135 &
  0.19609 &
  0.21429 &
  0.231 &
  0.23969 \\
\textbf{CSRM} &
  0.16314 &
  0.32207 &
  0.40702 &
  0.53426 &
  0.65601 &
  0.16314 &
  0.23188 &
  0.25111 &
  0.26802 &
  0.27656 \\ \hline
\cellcolor[HTML]{333333}{\color[HTML]{FFFFFF} } &
  \multicolumn{5}{c|}{\textbf{HR@}} &
  \multicolumn{5}{c|}{\textbf{MRR@}} \\ \cline{2-11} 
\multirow{-2}{*}{\cellcolor[HTML]{333333}{\color[HTML]{FFFFFF} \textbf{CIKMCUP}}} &
  \textbf{1} &
  \textbf{3} &
  \textbf{5} &
  \textbf{10} &
  \textbf{20} &
  \textbf{1} &
  \textbf{3} &
  \textbf{5} &
  \textbf{10} &
  \textbf{20} \\ \hline
\textbf{S-POP} &
  0.13222 &
  0.21957 &
  0.24145 &
  0.25193 &
  0.25947 &
  0.13222 &
  0.17102 &
  0.17616 &
  0.17773 &
  0.17824 \\
\textbf{AR} &
  0.04136 &
  0.09532 &
  0.13353 &
  0.17825 &
  0.17909 &
  0.04136 &
  0.06425 &
  0.07294 &
  0.07903 &
  0.07908 \\
\textbf{SR} &
  0.0388 &
  0.0876 &
  0.11615 &
  0.15129 &
  0.17472 &
  0.0388 &
  0.05922 &
  0.06567 &
  0.07045 &
  0.07209 \\
\textbf{VSKNN} &
  0.09084 & 0.18334 & 0.23906 & 0.32218 & 0.39371 & 0.09084 & 0.13065 & 0.14352 & 0.15478 & 0.15975 \\
\textbf{SMF} &
  0.0413 &
  0.10271 &
  0.14554 &
  0.22203 &
  0.32823 &
  0.0413 &
  0.06742 &
  0.07703 &
  0.08724 &
  0.0946 \\
\textbf{Item2Vec} &
  0.0174 &
  0.04294 &
  0.06232 &
  0.10064 &
  0.15041 &
  0.0174 &
  0.02837 &
  0.03264 &
  0.03775 &
  0.04113 \\
\textbf{GRU4Rec+} &
  0.02292 &
  0.04747 &
  0.06384 &
  0.08656 &
  0.11971 &
  0.02292 &
  0.03346 &
  0.03709 &
  0.04015 &
  0.04244 \\
\textbf{NARM} &
  0.03807 &
  0.08633 &
  0.12301 &
  0.18697 &
  0.3157 &
  0.03807 &
  0.05928 &
  0.06782 &
  0.07639 &
  0.08415 \\
\textbf{STAMP} &
  0.02667 &
  0.06825 &
  0.09408 &
  0.14595 &
  0.21273 &
  0.02667 &
  0.04424 &
  0.0501 &
  0.05699 &
  0.06155 \\
\textbf{NextItNet} &
  0.00195 &
  0.00521 &
  0.00586 &
  0.01042 &
  0.01497 &
  0.00195 &
  0.00336 &
  0.00353 &
  0.00409 &
  0.0044 \\
\textbf{SRGNN} &
  0.02549 &
  0.05757 &
  0.07751 &
  0.11061 &
  0.15132 &
  0.02549 &
  0.03958 &
  0.04411 &
  0.0486 &
  0.05142 \\
\textbf{CSRM} &
  0.04322 &
  0.10563 &
  0.15244 &
  0.22834 &
  0.31773 &
  0.04322 &
  0.06982 &
  0.08049 &
  0.0906 &
  0.09685 \\ \hline
\cellcolor[HTML]{333333}{\color[HTML]{FFFFFF} } &
  \multicolumn{5}{c|}{\textbf{HR@}} &
  \multicolumn{5}{c|}{\textbf{MRR@}} \\ \cline{2-11} 
\multirow{-2}{*}{\cellcolor[HTML]{333333}{\color[HTML]{FFFFFF} \textbf{TMALL}}} &
  \textbf{1} &
  \textbf{3} &
  \textbf{5} &
  \textbf{10} &
  \textbf{20} &
  \textbf{1} &
  \textbf{3} &
  \textbf{5} &
  \textbf{10} &
  \textbf{20} \\ \hline
\textbf{S-POP} &
  0.04876 &
  0.11326 &
  0.14327 &
  0.17518 &
  0.19311 &
  0.04876 &
  0.07681 &
  0.08368 &
  0.08805 &
  0.08935 \\
\textbf{AR} &
  0.01224 &
  0.02634 &
  0.03543 &
  0.04888 &
  0.0496 &
  0.01224 &
  0.0183 &
  0.02035 &
  0.02219 &
  0.02225 \\
\textbf{SR} &
  0.01158 &
  0.02374 &
  0.03091 &
  0.04263 &
  0.05459 &
  0.01158 &
  0.01673 &
  0.01836 &
  0.01991 &
  0.02075 \\
\textbf{VSKNN} &
  0.04172 & 0.06539 & 0.07883 & 0.08965 & 0.11669 & 0.04324 & 0.07608 & 0.06261 & 0.06358 & 0.05396 \\
\textbf{SMF} &
  0.0156 &
  0.03865 &
  0.05477 &
  0.08105 &
  0.11333 &
  0.0156 &
  0.02542 &
  0.02908 &
  0.03255 &
  0.03476 \\
\textbf{Item2Vec} &
  0.00267 &
  0.00636 &
  0.00908 &
  0.01403 &
  0.02143 &
  0.00267 &
  0.00423 &
  0.00485 &
  0.0055 &
  0.006 \\
\textbf{GRU4Rec+} &
  0.01576 &
  0.03594 &
  0.04943 &
  0.06961 &
  0.09027 &
  0.01576 &
  0.02437 &
  0.02743 &
  0.03014 &
  0.03157 \\
\textbf{NARM} &
  0.02143 &
  0.04888 &
  0.06912 &
  0.10585 &
  0.16867 &
  0.02143 &
  0.03342 &
  0.03813 &
  0.04295 &
  0.04676 \\
\textbf{STAMP} &
  0.03585 &
  0.07247 &
  0.09296 &
  0.122 &
  0.15468 &
  0.03585 &
  0.05171 &
  0.05638 &
  0.06027 &
  0.06253 \\
\textbf{NextItNet} &
  0.00696 &
  0.01357 &
  0.01779 &
  0.02737 &
  0.03752 &
  0.00696 &
  0.01002 &
  0.01092 &
  0.01219 &
  0.01287 \\
\textbf{SRGNN} &
  0.03022 &
  0.05978 &
  0.07548 &
  0.1011 &
  0.12883 &
  0.03022 &
  0.043 &
  0.04656 &
  0.04997 &
  0.05188 \\
\textbf{CSRM} &
  0.01894 &
  0.03963 &
  0.05328 &
  0.07492 &
  0.09991 &
  0.01894 &
  0.02788 &
  0.03097 &
  0.03386 &
  0.03559 \\ \hline
\cellcolor[HTML]{333333}{\color[HTML]{FFFFFF} } &
  \multicolumn{5}{c|}{\textbf{HR@}} &
  \multicolumn{5}{c|}{\textbf{MRR@}} \\ \cline{2-11} 
\multirow{-2}{*}{\cellcolor[HTML]{333333}{\color[HTML]{FFFFFF} \textbf{ROCKET}}} &
  \textbf{1} &
  \textbf{3} &
  \textbf{5} &
  \textbf{10} &
  \textbf{20} &
  \textbf{1} &
  \textbf{3} &
  \textbf{5} &
  \textbf{10} &
  \textbf{20} \\ \hline
\textbf{S-POP} &
  0.04844 &
  0.12409 &
  0.13537 &
  0.15328 &
  0.17651 &
  0.04844 &
  0.08328 &
  0.0859 &
  0.08835 &
  0.09003 \\
\textbf{AR} &
  0.06702 &
  0.13338 &
  0.16457 &
  0.19376 &
  0.19841 &
  0.06702 &
  0.09578 &
  0.10271 &
  0.10678 &
  0.10712 \\
\textbf{SR} &
  0.06038 &
  0.11015 &
  0.1294 &
  0.14333 &
  0.15461 &
  0.06038 &
  0.08129 &
  0.08567 &
  0.08772 &
  0.08849 \\
\textbf{VSKNN} &
  0.23916 & 0.39860 & 0.45548 & 0.51235 & 0.55058 & 0.23916 & 0.30901 & 0.32211 & 0.32983 & 0.33249 \\
\textbf{SMF} &
  0.0637 &
  0.12741 &
  0.17386 &
  0.22561 &
  0.26543 &
  0.0637 &
  0.09102 &
  0.102 &
  0.10881 &
  0.1115 \\
\textbf{Item2Vec} &
  0.0126 &
  0.03149 &
  0.03919 &
  0.04409 &
  0.05038 &
  0.0126 &
  0.02064 &
  0.02243 &
  0.0232 &
  0.02362 \\
\textbf{GRU4Rec+} &
  0.05177 &
  0.08965 &
  0.11427 &
  0.13826 &
  0.1654 &
  0.05177 &
  0.06839 &
  0.07417 &
  0.07738 &
  0.07937 \\
\textbf{NARM} &
  0.09251 &
  0.15928 &
  0.18371 &
  0.24605 &
  0.3066 &
  0.09251 &
  0.11974 &
  0.1256 &
  0.134 &
  0.13743 \\
\textbf{STAMP} &
  0.03874 &
  0.08818 &
  0.11957 &
  0.15431 &
  0.18504 &
  0.03874 &
  0.05979 &
  0.06733 &
  0.07196 &
  0.07419 \\
\textbf{NextItNet} &
  0.01875 &
  0.02969 &
  0.03438 &
  0.04844 &
  0.05781 &
  0.01875 &
  0.02318 &
  0.02419 &
  0.02628 &
  0.02687 \\
\textbf{SRGNN} &
  0.02669 &
  0.05273 &
  0.0625 &
  0.07422 &
  0.09115 &
  0.02669 &
  0.03754 &
  0.03972 &
  0.04125 &
  0.04237 \\
\textbf{CSRM} &
  0.08178 &
  0.16955 &
  0.20612 &
  0.25399 &
  0.30053 &
  0.08178 &
  0.11857 &
  0.12712 &
  0.13358 &
  0.1368 \\ \hline
\end{tabular}}

\label{tab:timespan-2}
\end{table*}
