# Supplementary material for: Comprehensive Empirical Evaluation of Deep Learning Approaches for Session-based Recommendation in E-Commerce
Source: arXiv:2010.12540 source file (2020-10-17)
Supplement: Supplementary file 3 [file tab11.tex]

\begin{table*}[!h]
\centering
\caption{RQ6: Training using the sessions of the most recent 7 days before the testing set.}
\resizebox{0.9\textwidth}{!}{\begin{tabular}{|c|ccccc|ccccc|}
\hline
\cellcolor[HTML]{333333}{\color[HTML]{FFFFFF} } &
  \multicolumn{5}{c|}{\textbf{HR@}} &
  \multicolumn{5}{c|}{\textbf{MRR@}} \\ \cline{2-11} 
\multirow{-2}{*}{\cellcolor[HTML]{333333}{\color[HTML]{FFFFFF} \textbf{RECSYS}}} &
  \textbf{1} &
  \textbf{3} &
  \textbf{5} &
  \textbf{10} &
  \textbf{20} &
  \textbf{1} &
  \textbf{3} &
  \textbf{5} &
  \textbf{10} &
  \textbf{20} \\ \hline
\textbf{S-POP} &
  0.03734 &
  0.10076 &
  0.12558 &
  0.14822 &
  0.16662 &
  0.03734 &
  0.06511 &
  0.07079 &
  0.07392 &
  0.07511 \\
\textbf{AR} &
  0.118 &
  0.22986 &
  0.29309 &
  0.36132 &
  0.36219 &
  0.118 &
  0.16625 &
  0.18059 &
  0.1903 &
  0.19035 \\
\textbf{SR} &
  0.0361 &
  0.08348 &
  0.11067 &
  0.15434 &
  0.18925 &
  0.0361 &
  0.0562 &
  0.06239 &
  0.06824 &
  0.07072 \\
\textbf{VSKNN} &
  0.09913 & 0.20987 & 0.26796 & 0.31952 & 0.39772 & 0.10499 & 0.14455 & 0.16437 & 0.17460 & 0.18091 \\
\textbf{SMF} &
  0.0772 &
  0.20517 &
  0.2933 &
  0.43169 &
  0.55566 &
  0.0772 &
  0.13179 &
  0.15178 &
  0.17026 &
  0.17896 \\
\textbf{Item2Vec} &
  0.07405 &
  0.14618 &
  0.19101 &
  0.26475 &
  0.3534 &
  0.07405 &
  0.10537 &
  0.11551 &
  0.12526 &
  0.13137 \\
\textbf{GRU4Rec+} &
  0.08516 &
  0.18774 &
  0.26189 &
  0.38997 &
  0.52056 &
  0.08516 &
  0.12883 &
  0.1456 &
  0.16257 &
  0.17168 \\
\textbf{NARM} &
  0.11816 &
  0.27464 &
  0.37502 &
  0.52189 &
  0.70713 &
  0.11816 &
  0.18602 &
  0.20882 &
  0.2284 &
  0.23976 \\
\textbf{STAMP} &
  0.14767 &
  0.13084 &
  0.26508 &
  0.34558 &
  0.46611 &
  0.13084 &
  0.18865 &
  0.20701 &
  0.22305 &
  0.23186 \\
\textbf{NextItNet} &
  0.18048 &
  0.33839 &
  0.41508 &
  0.52363 &
  0.62568 &
  0.18048 &
  0.2488 &
  0.26622 &
  0.28082 &
  0.28795 \\
\textbf{SRGNN} &
  0.13781 &
  0.28069 &
  0.36588 &
  0.49366 &
  0.61621 &
  0.13781 &
  0.19955 &
  0.2189 &
  0.23586 &
  0.24435 \\
\textbf{CSRM} &
  0.16685 &
  0.3255 &
  0.41197 &
  0.54531 &
  0.66892 &
  0.16685 &
  0.23571 &
  0.25543 &
  0.27326 &
  0.28193 \\ \hline
\cellcolor[HTML]{333333}{\color[HTML]{FFFFFF} } &
  \multicolumn{5}{c|}{\textbf{HR@}} &
  \multicolumn{5}{c|}{\textbf{MRR@}} \\ \cline{2-11} 
\multirow{-2}{*}{\cellcolor[HTML]{333333}{\color[HTML]{FFFFFF} \textbf{CIKMCUP}}} &
  \textbf{1} &
  \textbf{3} &
  \textbf{5} &
  \textbf{10} &
  \textbf{20} &
  \textbf{1} &
  \textbf{3} &
  \textbf{5} &
  \textbf{10} &
  \textbf{20} \\ \hline
\textbf{S-POP} &
  0.1072 &
  0.18874 &
  0.2112 &
  0.22497 &
  0.23045 &
  0.1072 &
  0.14359 &
  0.14873 &
  0.15075 &
  0.1511 \\
\textbf{AR} &
  0.04308 &
  0.09269 &
  0.13191 &
  0.17974 &
  0.18256 &
  0.04308 &
  0.06434 &
  0.07332 &
  0.08002 &
  0.08021 \\
\textbf{SR} &
  0.04201 &
  0.09688 &
  0.12723 &
  0.17695 &
  0.21742 &
  0.04201 &
  0.06527 &
  0.07218 &
  0.07885 &
  0.08174 \\
\textbf{VSKNN} &
  0.06603 & 0.13100 & 0.16883 & 0.22163 & 0.27536 & 0.06603 & 0.09422 & 0.10287 & 0.10982 & 0.11359 \\
\textbf{SMF} &
  0.04142 &
  0.09872 &
  0.14331 &
  0.22419 &
  0.33107 &
  0.04142 &
  0.06528 &
  0.07536 &
  0.08599 &
  0.09333 \\
\textbf{Item2Vec} &
  0.02183 &
  0.04957 &
  0.07352 &
  0.12445 &
  0.18903 &
  0.02183 &
  0.0334 &
  0.03883 &
  0.04557 &
  0.0499 \\
\textbf{GRU4Rec+} &
  0.02129 &
  0.05182 &
  0.0759 &
  0.11392 &
  0.16265 &
  0.02129 &
  0.03433 &
  0.03979 &
  0.04483 &
  0.04819 \\
\textbf{NARM} &
  0.04203 &
  0.1055 &
  0.15468 &
  0.24037 &
  0.37987 &
  0.04203 &
  0.06947 &
  0.08064 &
  0.09236 &
  0.1009 \\
\textbf{STAMP} &
  0.03476 &
  0.07993 &
  0.11142 &
  0.16907 &
  0.24083 &
  0.03476 &
  0.05378 &
  0.06093 &
  0.0686 &
  0.07361 \\
\textbf{NextItNet} &
  0.00781 &
  0.01823 &
  0.02396 &
  0.04323 &
  0.07604 &
  0.00781 &
  0.01215 &
  0.01348 &
  0.01593 &
  0.01811 \\
\textbf{SRGNN} &
  0.04113 &
  0.09906 &
  0.14726 &
  0.21742 &
  0.30218 &
  0.04113 &
  0.06535 &
  0.07632 &
  0.08552 &
  0.09139 \\
\textbf{CSRM} &
  0.04096 &
  0.10203 &
  0.14358 &
  0.21999 &
  0.30608 &
  0.04096 &
  0.0668 &
  0.07627 &
  0.0864 &
  0.0924 \\ \hline
\cellcolor[HTML]{333333}{\color[HTML]{FFFFFF} } &
  \multicolumn{5}{c|}{\textbf{HR@}} &
  \multicolumn{5}{c|}{\textbf{MRR@}} \\ \cline{2-11} 
\multirow{-2}{*}{\cellcolor[HTML]{333333}{\color[HTML]{FFFFFF} \textbf{TMALL}}} &
  \textbf{1} &
  \textbf{3} &
  \textbf{5} &
  \textbf{10} &
  \textbf{20} &
  \textbf{1} &
  \textbf{3} &
  \textbf{5} &
  \textbf{10} &
  \textbf{20} \\ \hline
\textbf{S-POP} &
  0.04641 &
  0.10609 &
  0.13483 &
  0.16695 &
  0.18707 &
  0.04641 &
  0.07226 &
  0.07883 &
  0.0832 &
  0.08465 \\
\textbf{AR} &
  0.0139 &
  0.02955 &
  0.03935 &
  0.05323 &
  0.05423 &
  0.0139 &
  0.02061 &
  0.02281 &
  0.02474 &
  0.0248 \\
\textbf{SR} &
  0.01337 &
  0.02719 &
  0.0353 &
  0.04836 &
  0.06257 &
  0.01337 &
  0.01935 &
  0.02119 &
  0.02295 &
  0.02393 \\
\textbf{VSKNN} &
  0.03786 & 0.05265 & 0.05627 & 0.07584 & 0.08770 & 0.02825 & 0.04194 & 0.04714 & 0.04479 & 0.04785 \\
\textbf{SMF} &
  0.01522 &
  0.04034 &
  0.05789 &
  0.08677 &
  0.12075 &
  0.01522 &
  0.02596 &
  0.02995 &
  0.03376 &
  0.03611 \\
\textbf{Item2Vec} &
  0.00213 &
  0.00521 &
  0.00738 &
  0.01172 &
  0.01842 &
  0.00213 &
  0.00343 &
  0.00392 &
  0.00448 &
  0.00493 \\
\textbf{GRU4Rec+} &
  0.02217 &
  0.05062 &
  0.06804 &
  0.09559 &
  0.12456 &
  0.02217 &
  0.03423 &
  0.03817 &
  0.04186 &
  0.04387 \\
\textbf{NARM} &
  0.03502 &
  0.08048 &
  0.10992 &
  0.15952 &
  0.23458 &
  0.03502 &
  0.05469 &
  0.06139 &
  0.06837 &
  0.07307 \\
\textbf{STAMP} &
  0.03141 &
  0.06188 &
  0.08084 &
  0.11039 &
  0.14463 &
  0.03141 &
  0.04442 &
  0.04875 &
  0.05269 &
  0.05506 \\
\textbf{NextItNet} &
  0.01858 &
  0.0389 &
  0.04797 &
  0.06469 &
  0.08053 &
  0.01858 &
  0.02721 &
  0.02927 &
  0.03149 &
  0.03256 \\
\textbf{SRGNN} &
  0.03533 &
  0.07152 &
  0.09185 &
  0.1228 &
  0.15816 &
  0.03533 &
  0.05099 &
  0.05561 &
  0.05973 &
  0.06218 \\
\textbf{CSRM} &
  0.0256 &
  0.05599 &
  0.07535 &
  0.10739 &
  0.14362 &
  0.0256 &
  0.03857 &
  0.04297 &
  0.04724 &
  0.04972 \\ \hline
\cellcolor[HTML]{333333}{\color[HTML]{FFFFFF} } &
  \multicolumn{5}{c|}{\textbf{HR@}} &
  \multicolumn{5}{c|}{\textbf{MRR@}} \\ \cline{2-11} 
\multirow{-2}{*}{\cellcolor[HTML]{333333}{\color[HTML]{FFFFFF} \textbf{ROCKET}}} &
  \textbf{1} &
  \textbf{3} &
  \textbf{5} &
  \textbf{10} &
  \textbf{20} &
  \textbf{1} &
  \textbf{3} &
  \textbf{5} &
  \textbf{10} &
  \textbf{20} \\ \hline
\textbf{S-POP} &
  0.03767 &
  0.12021 &
  0.13356 &
  0.14486 &
  0.16164 &
  0.03767 &
  0.07568 &
  0.0788 &
  0.08035 &
  0.08158 \\
\textbf{AR} &
  0.05445 &
  0.11336 &
  0.14144 &
  0.1637 &
  0.16473 &
  0.05445 &
  0.08014 &
  0.08651 &
  0.08962 &
  0.08971 \\
\textbf{SR} &
  0.04692 &
  0.08801 &
  0.11404 &
  0.13425 &
  0.14932 &
  0.04692 &
  0.06507 &
  0.07098 &
  0.07373 &
  0.0748 \\
\textbf{VSKNN} &
  0.16814 & 0.27190 & 0.30787 & 0.34619 & 0.37304 & 0.16814 & 0.21411 & 0.22249 & 0.22771 & 0.22959 \\
\textbf{SMF} &
  0.04282 &
  0.10346 &
  0.13601 &
  0.18979 &
  0.24837 &
  0.04282 &
  0.06909 &
  0.07642 &
  0.08378 &
  0.08782 \\
\textbf{Item2Vec} &
  0.0218 &
  0.04861 &
  0.06648 &
  0.08792 &
  0.10936 &
  0.0218 &
  0.03318 &
  0.03738 &
  0.04024 &
  0.04167 \\
\textbf{GRU4Rec+} &
  0.04317 &
  0.07892 &
  0.10118 &
  0.12951 &
  0.15312 &
  0.04317 &
  0.05863 &
  0.06367 &
  0.06741 &
  0.06902 \\
\textbf{NARM} &
  0.06404 &
  0.13902 &
  0.16607 &
  0.20748 &
  0.27297 &
  0.06404 &
  0.09449 &
  0.10077 &
  0.10633 &
  0.11019 \\
\textbf{STAMP} &
  0.05229 &
  0.09288 &
  0.12281 &
  0.15721 &
  0.19436 &
  0.05229 &
  0.07006 &
  0.07711 &
  0.08168 &
  0.08426 \\
\textbf{NextItNet} &
  0.01471 &
  0.02574 &
  0.03585 &
  0.05147 &
  0.06618 &
  0.01471 &
  0.01976 &
  0.02197 &
  0.02388 &
  0.02496 \\
\textbf{SRGNN} &
  0.02989 &
  0.05503 &
  0.07201 &
  0.09545 &
  0.11583 &
  0.02989 &
  0.04036 &
  0.04425 &
  0.04747 &
  0.0489 \\
\textbf{CSRM} &
  0.06587 &
  0.13276 &
  0.16894 &
  0.21843 &
  0.2628 &
  0.06587 &
  0.09431 &
  0.10264 &
  0.10928 &
  0.1123 \\ \hline
\end{tabular}}

\label{tab:timespan-7}
\end{table*}
