# Supplementary material for: Comprehensive Empirical Evaluation of Deep Learning Approaches for Session-based Recommendation in E-Commerce
Source: arXiv:2010.12540 source file (2020-10-17)
Supplement: Supplementary file 4 [file tab12.tex]

\begin{table*}[!h]
\centering
\caption{RQ6: training using the sessions of the most recent 14 days before the testing set.}
\resizebox{0.9\textwidth}{!}{\begin{tabular}{|c|ccccc|ccccc|}
\hline
\cellcolor[HTML]{333333}{\color[HTML]{FFFFFF} } &
  \multicolumn{5}{c|}{\textbf{HR@}} &
  \multicolumn{5}{c|}{\textbf{MRR@}} \\ \cline{2-11} 
\multirow{-2}{*}{\cellcolor[HTML]{333333}{\color[HTML]{FFFFFF} \textbf{RECSYS}}} &
  \textbf{1} &
  \textbf{3} &
  \textbf{5} &
  \textbf{10} &
  \textbf{20} &
  \textbf{1} &
  \textbf{3} &
  \textbf{5} &
  \textbf{10} &
  \textbf{20} \\ \hline
\textbf{S-POP} &
  0.03671 &
  0.10021 &
  0.12507 &
  0.14586 &
  0.1596 &
  0.03671 &
  0.06455 &
  0.07026 &
  0.07314 &
  0.07412 \\
\textbf{AR} &
  0.10322 &
  0.19791 &
  0.2579 &
  0.32011 &
  0.32024 &
  0.10322 &
  0.14393 &
  0.15759 &
  0.16643 &
  0.16643 \\
\textbf{SR} &
  0.03384 &
  0.08353 &
  0.11818 &
  0.1719 &
  0.22146 &
  0.03384 &
  0.05533 &
  0.06317 &
  0.07027 &
  0.0737 \\
\textbf{VSKNN} &
  0.09375 & 0.18943 & 0.23744 & 0.30791 & 0.36286 & 0.10491 & 0.14135 & 0.16055 & 0.16436 & 0.17399 \\
\textbf{SMF} &
  0.07265 &
  0.20339 &
  0.2893 &
  0.4306 &
  0.55955 &
  0.07265 &
  0.12789 &
  0.14742 &
  0.16628 &
  0.17527 \\
\textbf{Item2Vec} &
  0.07729 &
  0.15461 &
  0.19994 &
  0.27403 &
  0.36161 &
  0.07729 &
  0.11034 &
  0.1206 &
  0.13038 &
  0.13641 \\
\textbf{GRU4Rec+} &
  0.08554 &
  0.19469 &
  0.2738 &
  0.39686 &
  0.53192 &
  0.08554 &
  0.13179 &
  0.14972 &
  0.16604 &
  0.17543 \\
\textbf{NARM} &
  0.11018 &
  0.27523 &
  0.37441 &
  0.51956 &
  0.70541 &
  0.11018 &
  0.18072 &
  0.20331 &
  0.22279 &
  0.23414 \\
\textbf{STAMP} &
  0.13012 &
  0.27107 &
  0.35345 &
  0.47785 &
  0.60268 &
  0.13012 &
  0.19059 &
  0.20933 &
  0.2259 &
  0.2346 \\
\textbf{NextItNet} &
  0.18486 &
  0.3436 &
  0.42338 &
  0.52951 &
  0.63021 &
  0.18486 &
  0.25374 &
  0.27193 &
  0.28615 &
  0.29324 \\
\textbf{SRGNN} &
  0.14067 &
  0.28651 &
  0.37042 &
  0.49563 &
  0.61891 &
  0.14067 &
  0.20359 &
  0.22263 &
  0.23937 &
  0.24795 \\
\textbf{CSRM} &
  0.16803 &
  0.32619 &
  0.41463 &
  0.54749 &
  0.67328 &
  0.16803 &
  0.23642 &
  0.25653 &
  0.2742 &
  0.283 \\ \hline
\cellcolor[HTML]{333333}{\color[HTML]{FFFFFF} } &
  \multicolumn{5}{c|}{\textbf{HR@}} &
  \multicolumn{5}{c|}{\textbf{MRR@}} \\ \cline{2-11} 
\multirow{-2}{*}{\cellcolor[HTML]{333333}{\color[HTML]{FFFFFF} \textbf{CIKMCUP}}} &
  \textbf{1} &
  \textbf{3} &
  \textbf{5} &
  \textbf{10} &
  \textbf{20} &
  \textbf{1} &
  \textbf{3} &
  \textbf{5} &
  \textbf{10} &
  \textbf{20} \\ \hline
\textbf{S-POP} &
  0.03948 &
  0.10368 &
  0.12168 &
  0.13605 &
  0.14249 &
  0.03948 &
  0.06798 &
  0.07216 &
  0.07422 &
  0.07467 \\
\textbf{AR} &
  0.04472 &
  0.0971 &
  0.13511 &
  0.1856 &
  0.18815 &
  0.04472 &
  0.06713 &
  0.07576 &
  0.08289 &
  0.08305 \\
\textbf{SR} &
  0.03884 &
  0.09409 &
  0.13432 &
  0.19653 &
  0.25379 &
  0.03884 &
  0.06267 &
  0.07174 &
  0.07995 &
  0.08393 \\
\textbf{VSKNN} &
  0.05609 & 0.11352 & 0.14673 & 0.19382 & 0.24091 & 0.05609 & 0.08107 & 0.08866 & 0.09494 & 0.09828 \\
\textbf{SMF} &
  0.03817 &
  0.09739 &
  0.14086 &
  0.22616 &
  0.33537 &
  0.03817 &
  0.06316 &
  0.07296 &
  0.08419 &
  0.09162 \\
\textbf{Item2Vec} &
  0.02331 &
  0.05139 &
  0.06952 &
  0.11314 &
  0.17639 &
  0.02331 &
  0.03535 &
  0.03944 &
  0.04511 &
  0.04942 \\
\textbf{GRU4Rec+} &
  0.02147 &
  0.05682 &
  0.08589 &
  0.14097 &
  0.21059 &
  0.02147 &
  0.03628 &
  0.0429 &
  0.0502 &
  0.05502 \\
\textbf{NARM} &
  0.03873 &
  0.10812 &
  0.15912 &
  0.24586 &
  0.41707 &
  0.03873 &
  0.06869 &
  0.08039 &
  0.09184 &
  0.10185 \\
\textbf{STAMP} &
  0.03264 &
  0.07777 &
  0.11363 &
  0.18039 &
  0.26729 &
  0.03264 &
  0.05176 &
  0.05983 &
  0.0686 &
  0.07451 \\
\textbf{NextItNet} &
  0.01904 &
  0.03662 &
  0.05127 &
  0.07666 &
  0.1167 &
  0.01904 &
  0.02661 &
  0.02996 &
  0.03333 &
  0.036 \\
\textbf{SRGNN} &
  0.04145 &
  0.10501 &
  0.15678 &
  0.2406 &
  0.34587 &
  0.04145 &
  0.06837 &
  0.08005 &
  0.09117 &
  0.09846 \\
\textbf{CSRM} &
  0.04336 &
  0.10544 &
  0.1523 &
  0.23674 &
  0.34029 &
  0.04336 &
  0.0696 &
  0.0803 &
  0.09146 &
  0.09858 \\ \hline
\cellcolor[HTML]{333333}{\color[HTML]{FFFFFF} } &
  \multicolumn{5}{c|}{\textbf{HR@}} &
  \multicolumn{5}{c|}{\textbf{MRR@}} \\ \cline{2-11} 
\multirow{-2}{*}{\cellcolor[HTML]{333333}{\color[HTML]{FFFFFF} \textbf{TMALL}}} &
  \textbf{1} &
  \textbf{3} &
  \textbf{5} &
  \textbf{10} &
  \textbf{20} &
  \textbf{1} &
  \textbf{3} &
  \textbf{5} &
  \textbf{10} &
  \textbf{20} \\ \hline
\textbf{S-POP} &
  0.0454 &
  0.10433 &
  0.13224 &
  0.16499 &
  0.1853 &
  0.0454 &
  0.07086 &
  0.07723 &
  0.08168 &
  0.08313 \\
\textbf{AR} &
  0.01464 &
  0.0306 &
  0.04136 &
  0.05569 &
  0.05625 &
  0.01464 &
  0.02151 &
  0.02396 &
  0.02592 &
  0.02596 \\
\textbf{SR} &
  0.0145 &
  0.02965 &
  0.03906 &
  0.05354 &
  0.06861 &
  0.0145 &
  0.02099 &
  0.02312 &
  0.02505 &
  0.0261 \\
\textbf{VSKNN} &
  0.02897 & 0.04645 & 0.04589 & 0.05787 & 0.07395 & 0.03222 & 0.04274 & 0.04843 & 0.03824 & 0.03583 \\
\textbf{SMF} &
  0.01573 &
  0.0433 &
  0.06187 &
  0.0915 &
  0.12622 &
  0.01573 &
  0.02748 &
  0.0317 &
  0.03564 &
  0.03801 \\
\textbf{Item2Vec} &
  0.00204 &
  0.00501 &
  0.00717 &
  0.01159 &
  0.01863 &
  0.00204 &
  0.00328 &
  0.00376 &
  0.00434 &
  0.00482 \\
\textbf{GRU4Rec+} &
  0.02544 &
  0.05867 &
  0.07992 &
  0.11163 &
  0.14446 &
  0.02544 &
  0.03962 &
  0.04443 &
  0.04866 &
  0.05092 \\
\textbf{NARM} &
  0.03744 &
  0.0914 &
  0.12225 &
  0.16466 &
  0.2489 &
  0.03744 &
  0.06137 &
  0.06845 &
  0.0739 &
  0.0789 \\
\textbf{STAMP} &
  0.03218 &
  0.06457 &
  0.08592 &
  0.11847 &
  0.15537 &
  0.03218 &
  0.04605 &
  0.05089 &
  0.05523 &
  0.05778 \\
\textbf{NextItNet} &
  0.02543 &
  0.04989 &
  0.06563 &
  0.08879 &
  0.11336 &
  0.02543 &
  0.03615 &
  0.03974 &
  0.04283 &
  0.04447 \\
\textbf{SRGNN} &
  0.0382 &
  0.07667 &
  0.09919 &
  0.13454 &
  0.17489 &
  0.0382 &
  0.05479 &
  0.05991 &
  0.0646 &
  0.06739 \\
\textbf{CSRM} &
  0.03246 &
  0.0694 &
  0.0923 &
  0.12964 &
  0.17272 &
  0.03246 &
  0.04836 &
  0.05358 &
  0.05853 &
  0.0615 \\ \hline
\cellcolor[HTML]{333333}{\color[HTML]{FFFFFF} } &
  \multicolumn{5}{c|}{\textbf{HR@}} &
  \multicolumn{5}{c|}{\textbf{MRR@}} \\ \cline{2-11} 
\multirow{-2}{*}{\cellcolor[HTML]{333333}{\color[HTML]{FFFFFF} \textbf{ROCKET}}} &
  \textbf{1} &
  \textbf{3} &
  \textbf{5} &
  \textbf{10} &
  \textbf{20} &
  \textbf{1} &
  \textbf{3} &
  \textbf{5} &
  \textbf{10} &
  \textbf{20} \\ \hline
\textbf{S-POP} &
  0.03946 &
  0.11559 &
  0.13098 &
  0.14442 &
  0.15701 &
  0.03946 &
  0.07393 &
  0.07753 &
  0.07932 &
  0.08016 \\
\textbf{AR} &
  0.0557 &
  0.10747 &
  0.13154 &
  0.16093 &
  0.16177 &
  0.0557 &
  0.07841 &
  0.0838 &
  0.08794 &
  0.08799 \\
\textbf{SR} &
  0.04618 &
  0.0918 &
  0.11643 &
  0.13882 &
  0.15449 &
  0.04618 &
  0.06568 &
  0.07125 &
  0.07418 &
  0.07535 \\
\textbf{VSKNN} &
  0.13714 & 0.22234 & 0.25038 & 0.28342 & 0.30841 & 0.13714 & 0.17464 & 0.18107 & 0.18550 & 0.18721 \\
\textbf{SMF} &
  0.04002 &
  0.10411 &
  0.14442 &
  0.20347 &
  0.27064 &
  0.04002 &
  0.0674 &
  0.07664 &
  0.08449 &
  0.08924 \\
\textbf{Item2Vec} &
  0.02455 &
  0.05256 &
  0.07421 &
  0.09731 &
  0.13428 &
  0.02455 &
  0.03667 &
  0.04152 &
  0.0446 &
  0.04715 \\
\textbf{GRU4Rec+} &
  0.03727 &
  0.07789 &
  0.10097 &
  0.1338 &
  0.16606 &
  0.03727 &
  0.05457 &
  0.05977 &
  0.06418 &
  0.06638 \\
\textbf{NARM} &
  0.06628 &
  0.15536 &
  0.1933 &
  0.22802 &
  0.29868 &
  0.06628 &
  0.10561 &
  0.1144 &
  0.11905 &
  0.1232 \\
\textbf{STAMP} &
  0.04136 &
  0.09342 &
  0.12268 &
  0.1646 &
  0.20456 &
  0.04136 &
  0.06392 &
  0.07059 &
  0.07608 &
  0.07882 \\
\textbf{NextItNet} &
  0.0221 &
  0.0404 &
  0.05945 &
  0.07241 &
  0.09146 &
  0.0221 &
  0.02973 &
  0.03407 &
  0.03571 &
  0.03697 \\
\textbf{SRGNN} &
  0.03934 &
  0.08287 &
  0.10463 &
  0.13728 &
  0.16908 &
  0.03934 &
  0.05818 &
  0.06321 &
  0.06759 &
  0.06975 \\
\textbf{CSRM} &
  0.0665 &
  0.13578 &
  0.17307 &
  0.21953 &
  0.26322 &
  0.0665 &
  0.09655 &
  0.1052 &
  0.11153 &
  0.11465 \\ \hline
\end{tabular}}
\label{tab:timespan-14}
\end{table*}
