# Supplementary material for: Comprehensive Empirical Evaluation of Deep Learning Approaches for Session-based Recommendation in E-Commerce
Source: arXiv:2010.12540 source file (2020-10-17)
Supplement: Supplementary file 5 [file tab22.tex]

\begin{table*}[!h]
\centering
\caption{RQ3: performance of predictions on items whose frequency is very low in the training set \textless{}200 (\textless{}60) for RECSYS and TMALL (CIKMCUP and ROCKET).}
\resizebox{0.9\textwidth}{!}{\begin{tabular}{|c|ccccc|ccccc|}
\hline
\cellcolor[HTML]{333333}{\color[HTML]{FFFFFF} } &
  \multicolumn{5}{c|}{\textbf{HR@}} &
  \multicolumn{5}{c|}{\textbf{MRR@}} \\ \cline{2-11} 
\multirow{-2}{*}{\cellcolor[HTML]{333333}{\color[HTML]{FFFFFF} \textbf{RECSYS}}} &
  \textbf{1} &
  \textbf{3} &
  \textbf{5} &
  \textbf{10} &
  \textbf{20} &
  \textbf{1} &
  \textbf{3} &
  \textbf{5} &
  \textbf{10} &
  \textbf{20} \\ \hline
\textbf{S-POP} &
  0.03018 &
  0.08395 &
  0.10111 &
  0.11091 &
  0.11427 &
  0.03018 &
  0.05375 &
  0.0577 &
  0.05907 &
  0.05931 \\
\textbf{AR} &
  0.06246 &
  0.13009 &
  0.17659 &
  0.23162 &
  0.23176 &
  0.06246 &
  0.09182 &
  0.10249 &
  0.11023 &
  0.11024 \\
\textbf{SR} &
  0.06407 &
  0.13794 &
  0.18121 &
  0.24408 &
  0.30094 &
  0.06407 &
  0.09566 &
  0.10548 &
  0.114 &
  0.11801 \\
\textbf{VSKNN} &
  0.12117 & 0.18989 & 0.22025 & 0.26197 & 0.29738 & 0.12117 & 0.15101 & 0.15794 & 0.16359 & 0.16606 \\
\textbf{SMF} &
  0.07413 &
  0.19046 &
  0.26802 &
  0.37057 &
  0.47432 &
  0.07413 &
  0.12404 &
  0.14179 &
  0.15557 &
  0.16287 \\
\textbf{Item2Vec} &
  0.02549 &
  0.06103 &
  0.08578 &
  0.13675 &
  0.20463 &
  0.02549 &
  0.04057 &
  0.04619 &
  0.05298 &
  0.05763 \\
\textbf{GRU4Rec+} &
  0.06817 &
  0.1645 &
  0.23308 &
  0.33317 &
  0.43275 &
  0.06817 &
  0.10885 &
  0.12446 &
  0.13784 &
  0.14485 \\
\textbf{NARM} &
  0.07814 &
  0.23104 &
  0.33644 &
  0.48736 &
  0.67256 &
  0.07814 &
  0.14445 &
  0.16868 &
  0.1887 &
  0.2002 \\
\textbf{STAMP} &
  0.12252 &
  0.24897 &
  0.32509 &
  0.44361 &
  0.56432 &
  0.12252 &
  0.17693 &
  0.19428 &
  0.21015 &
  0.21857 \\
\textbf{NextItNet} &
  0.08404 &
  0.17438 &
  0.22674 &
  0.30629 &
  0.39236 &
  0.08404 &
  0.12285 &
  0.13481 &
  0.14543 &
  0.15138 \\
\textbf{SRGNN} &
  0.12789 &
  0.2608 &
  0.33917 &
  0.46395 &
  0.5824 &
  0.12789 &
  0.18458 &
  0.20246 &
  0.21905 &
  0.22734 \\
\textbf{CSRM} &
  0.151 &
  0.31124 &
  0.40604 &
  0.54675 &
  0.66949 &
  0.151 &
  0.21937 &
  0.24091 &
  0.25994 &
  0.26861 \\ \hline
\cellcolor[HTML]{333333}{\color[HTML]{FFFFFF} } &
  \multicolumn{5}{c|}{\textbf{HR@}} &
  \multicolumn{5}{c|}{\textbf{MRR@}} \\ \cline{2-11} 
\multirow{-2}{*}{\cellcolor[HTML]{333333}{\color[HTML]{FFFFFF} \textbf{CIKMCUP}}} &
  \textbf{1} &
  \textbf{3} &
  \textbf{5} &
  \textbf{10} &
  \textbf{20} &
  \textbf{1} &
  \textbf{3} &
  \textbf{5} &
  \textbf{10} &
  \textbf{20} \\ \hline
\textbf{S-POP} &
  0.0349 &
  0.09306 &
  0.1079 &
  0.11473 &
  0.11531 &
  0.0349 &
  0.06061 &
  0.06404 &
  0.06502 &
  0.06507 \\
\textbf{AR} &
  0.03301 &
  0.07896 &
  0.11444 &
  0.17086 &
  0.17115 &
  0.03301 &
  0.05235 &
  0.0604 &
  0.06817 &
  0.06819 \\
\textbf{SR} &
  0.03199 &
  0.07096 &
  0.09772 &
  0.15152 &
  0.20169 &
  0.03199 &
  0.04852 &
  0.05465 &
  0.06191 &
  0.06541 \\
\textbf{VSKNN} &
  0.05515 & 0.10205 & 0.13052 & 0.16862 & 0.20919 & 0.05515 & 0.07521 & 0.08164 & 0.08672 & 0.08952 \\
\textbf{SMF} &
  0.02974 &
  0.08171 &
  0.12816 &
  0.21417 &
  0.32117 &
  0.02974 &
  0.05118 &
  0.0617 &
  0.07305 &
  0.08034 \\
\textbf{Item2Vec} &
  0.02244 &
  0.04934 &
  0.07091 &
  0.11249 &
  0.17103 &
  0.02244 &
  0.03409 &
  0.03894 &
  0.04441 &
  0.04838 \\
\textbf{GRU4Rec+} &
  0.0233 &
  0.06028 &
  0.09095 &
  0.15168 &
  0.2258 &
  0.0233 &
  0.03884 &
  0.04584 &
  0.05385 &
  0.05892 \\
\textbf{NARM} &
  0.05693 &
  0.11397 &
  0.17865 &
  0.30007 &
  0.50559 &
  0.05693 &
  0.08104 &
  0.09518 &
  0.11143 &
  0.12318 \\
\textbf{STAMP} &
  0.04194 &
  0.11183 &
  0.17204 &
  0.27527 &
  0.40376 &
  0.04194 &
  0.07106 &
  0.08469 &
  0.09826 &
  0.10712 \\
\textbf{NextItNet} &
  0.02524 &
  0.051 &
  0.06904 &
  0.1051 &
  0.15301 &
  0.02524 &
  0.03649 &
  0.04069 &
  0.04533 &
  0.04855 \\
\textbf{SRGNN} &
  0.05599 &
  0.14453 &
  0.20573 &
  0.30859 &
  0.44401 &
  0.05599 &
  0.09321 &
  0.10727 &
  0.1212 &
  0.13071 \\
\textbf{CSRM} &
  0.05978 &
  0.13742 &
  0.18789 &
  0.29581 &
  0.42314 &
  0.05978 &
  0.09265 &
  0.10391 &
  0.11846 &
  0.12734 \\ \hline
\cellcolor[HTML]{333333}{\color[HTML]{FFFFFF} } &
  \multicolumn{5}{c|}{\textbf{HR@}} &
  \multicolumn{5}{c|}{\textbf{MRR@}} \\ \cline{2-11} 
\multirow{-2}{*}{\cellcolor[HTML]{333333}{\color[HTML]{FFFFFF} \textbf{TMALL}}} &
  \textbf{1} &
  \textbf{3} &
  \textbf{5} &
  \textbf{10} &
  \textbf{20} &
  \textbf{1} &
  \textbf{3} &
  \textbf{5} &
  \textbf{10} &
  \textbf{20} \\ \hline
\textbf{S-POP} &
  0.0471 &
  0.1102 &
  0.13952 &
  0.1703 &
  0.18683 &
  0.0471 &
  0.0471 &
  0.0471 &
  0.0471 &
  0.0471 \\
\textbf{AR} &
  0.01125 &
  0.02493 &
  0.03403 &
  0.04693 &
  0.04716 &
  0.01125 &
  0.01712 &
  0.01918 &
  0.02096 &
  0.02097 \\
\textbf{SR} &
  0.01068 &
  0.02235 &
  0.02944 &
  0.04068 &
  0.05219 &
  0.01068 &
  0.01561 &
  0.01721 &
  0.0187 &
  0.01951 \\
\textbf{VSKNN} &
  0.03708 & 0.05491 & 0.06517 & 0.08221 & 0.09819 & 0.03708 & 0.04411 & 0.04716 & 0.04994 & 0.05086 \\
\textbf{SMF} &
  0.01541 &
  0.03738 &
  0.05308 &
  0.07805 &
  0.11089 &
  0.01541 &
  0.02472 &
  0.02828 &
  0.03158 &
  0.03383 \\
\textbf{Item2Vec} &
  0.00277 &
  0.00635 &
  0.0091 &
  0.01435 &
  0.02182 &
  0.00277 &
  0.00432 &
  0.00494 &
  0.00562 &
  0.00613 \\
\textbf{GRU4Rec+} &
  0.01486 &
  0.03487 &
  0.04798 &
  0.06753 &
  0.08719 &
  0.01486 &
  0.02347 &
  0.02645 &
  0.02907 &
  0.03045 \\
\textbf{NARM} &
  0.02977 &
  0.05278 &
  0.0766 &
  0.10895 &
  0.16401 &
  0.02977 &
  0.03948 &
  0.04463 &
  0.04903 &
  0.05226 \\
\textbf{STAMP} &
  0.04389 &
  0.08695 &
  0.11129 &
  0.14826 &
  0.19037 &
  0.04389 &
  0.06255 &
  0.06808 &
  0.073 &
  0.07594 \\
\textbf{NextItNet} &
  0.00512 &
  0.01129 &
  0.0149 &
  0.02329 &
  0.03225 &
  0.00512 &
  0.00778 &
  0.00863 &
  0.00975 &
  0.01035 \\
\textbf{SRGNN} &
  0.03473 &
  0.07134 &
  0.09095 &
  0.11958 &
  0.15473 &
  0.03473 &
  0.05057 &
  0.05501 &
  0.05881 &
  0.06124 \\
\textbf{CSRM} &
  0.02439 &
  0.04779 &
  0.06201 &
  0.08311 &
  0.11113 &
  0.02439 &
  0.03428 &
  0.0375 &
  0.04029 &
  0.04225 \\ \hline
\cellcolor[HTML]{333333}{\color[HTML]{FFFFFF} } &
  \multicolumn{5}{c|}{\textbf{HR@}} &
  \multicolumn{5}{c|}{\textbf{MRR@}} \\ \cline{2-11} 
\multirow{-2}{*}{\cellcolor[HTML]{333333}{\color[HTML]{FFFFFF} \textbf{ROCKET}}} &
  \textbf{1} &
  \textbf{3} &
  \textbf{5} &
  \textbf{10} &
  \textbf{20} &
  \textbf{1} &
  \textbf{3} &
  \textbf{5} &
  \textbf{10} &
  \textbf{20} \\ \hline
\textbf{S-POP} &
  0.02694 &
  0.08517 &
  0.10168 &
  0.10979 &
  0.11182 &
  0.02694 &
  0.0533 &
  0.05716 &
  0.05835 &
  0.05851 \\
\textbf{AR} &
  0.0394 &
  0.07677 &
  0.10371 &
  0.1405 &
  0.14079 &
  0.0394 &
  0.05528 &
  0.06138 &
  0.06638 &
  0.06639 \\
\textbf{SR} &
  0.03708 &
  0.07561 &
  0.10632 &
  0.14108 &
  0.17207 &
  0.03708 &
  0.0534 &
  0.06048 &
  0.06522 &
  0.06741 \\
\textbf{VSKNN} &
  0.13640 & 0.18619 & 0.20856 & 0.23430 & 0.25643 & 0.13640 & 0.15897 & 0.16397 & 0.16753 & 0.16910 \\
\textbf{SMF} &
  0.02064 &
  0.08191 &
  0.11738 &
  0.17736 &
  0.23928 &
  0.02064 &
  0.04703 &
  0.05507 &
  0.06311 &
  0.06742 \\
\textbf{Item2Vec} &
  0.0181 &
  0.04741 &
  0.06494 &
  0.08966 &
  0.12385 &
  0.0181 &
  0.03051 &
  0.03455 &
  0.03766 &
  0.04 \\
\textbf{GRU4Rec+} &
  0.0408 &
  0.09519 &
  0.12935 &
  0.18153 &
  0.23656 &
  0.0408 &
  0.06388 &
  0.0717 &
  0.07853 &
  0.08239 \\
\textbf{NARM} &
  0.12836 &
  0.19752 &
  0.26391 &
  0.32877 &
  0.42441 &
  0.12836 &
  0.15714 &
  0.17538 &
  0.18215 &
  0.18764 \\
\textbf{STAMP} &
  0.05774 &
  0.13395 &
  0.18476 &
  0.24942 &
  0.30947 &
  0.05774 &
  0.08968 &
  0.10065 &
  0.11001 &
  0.11423 \\
\textbf{NextItNet} &
  0.06753 &
  0.12356 &
  0.1523 &
  0.19828 &
  0.25072 &
  0.06753 &
  0.09243 &
  0.09908 &
  0.10503 &
  0.10865 \\
\textbf{SRGNN} &
  0.07229 &
  0.15663 &
  0.18072 &
  0.21687 &
  0.28012 &
  0.07229 &
  0.10894 &
  0.11451 &
  0.11918 &
  0.12356 \\
\textbf{CSRM} &
  0.12174 &
  0.21739 &
  0.24348 &
  0.29565 &
  0.3913 &
  0.12174 &
  0.16377 &
  0.16942 &
  0.1764 &
  0.18293 \\ \hline
\end{tabular}}
\label{tab:freq-intermediate}
\end{table*}
