# Supplementary material for: Comprehensive Empirical Evaluation of Deep Learning Approaches for Session-based Recommendation in E-Commerce
Source: arXiv:2010.12540 source file (2020-10-17)
Supplement: Supplementary file 6 [file tab23.tex]

\begin{table*}[!h]
\centering
\caption{RQ3: performance of predictions on items whose frequency is high in the training set \textless{}300 (\textless{}100) for RECSYS and TMALL (CIKMCUP and ROCKET).}
\resizebox{0.9\textwidth}{!}{\begin{tabular}{|c|ccccc|ccccc|}
\hline
\cellcolor[HTML]{333333}{\color[HTML]{FFFFFF} } &
  \multicolumn{5}{c|}{\textbf{HR@}} &
  \multicolumn{5}{c|}{\textbf{MRR@}} \\ \cline{2-11} 
\multirow{-2}{*}{\cellcolor[HTML]{333333}{\color[HTML]{FFFFFF} \textbf{RECSYS}}} &
  \textbf{1} &
  \textbf{3} &
  \textbf{5} &
  \textbf{10} &
  \textbf{20} &
  \textbf{1} &
  \textbf{3} &
  \textbf{5} &
  \textbf{10} &
  \textbf{20} \\ \hline
\textbf{S-POP} &
  0.02965 &
  0.08348 &
  0.10068 &
  0.11201 &
  0.11567 &
  0.02965 &
  0.05318 &
  0.05716 &
  0.05876 &
  0.05903 \\
\textbf{AR} &
  0.06229 &
  0.13253 &
  0.18055 &
  0.23641 &
  0.23653 &
  0.06229 &
  0.09247 &
  0.10354 &
  0.11137 &
  0.11138 \\
\textbf{SR} &
  0.06404 &
  0.13906 &
  0.18478 &
  0.25462 &
  0.32176 &
  0.06404 &
  0.09611 &
  0.10658 &
  0.11598 &
  0.12069 \\
\textbf{VSKNN} &
  0.12145 & 0.19252 & 0.22658 & 0.27055 & 0.30935 & 0.12145 & 0.15222 & 0.15997 & 0.16591 & 0.16859 \\
\textbf{SMF} &
  0.07773 &
  0.19466 &
  0.26617 &
  0.37344 &
  0.47746 &
  0.07773 &
  0.12742 &
  0.14373 &
  0.15814 &
  0.16542 \\
\textbf{Item2Vec} &
  0.02379 &
  0.06006 &
  0.08493 &
  0.13688 &
  0.20754 &
  0.02379 &
  0.03907 &
  0.04471 &
  0.05157 &
  0.05639 \\
\textbf{GRU4Rec+} &
  0.06738 &
  0.16485 &
  0.23388 &
  0.3334 &
  0.43655 &
  0.06738 &
  0.10849 &
  0.12414 &
  0.13738 &
  0.14461 \\
\textbf{NARM} &
  0.08668 &
  0.23752 &
  0.34514 &
  0.49449 &
  0.67083 &
  0.08668 &
  0.1501 &
  0.17472 &
  0.19456 &
  0.20536 \\
\textbf{STAMP} &
  0.12467 &
  0.25739 &
  0.33313 &
  0.45037 &
  0.57278 &
  0.12467 &
  0.18193 &
  0.19928 &
  0.2148 &
  0.22335 \\
\textbf{NextItNet} &
  0.07759 &
  0.17643 &
  0.23628 &
  0.32736 &
  0.42361 &
  0.07759 &
  0.11999 &
  0.13372 &
  0.14584 &
  0.15245 \\
\textbf{SRGNN} &
  0.13276 &
  0.27234 &
  0.35266 &
  0.47393 &
  0.59412 &
  0.13276 &
  0.19275 &
  0.21098 &
  0.22719 &
  0.23559 \\
\textbf{CSRM} &
  0.14143 &
  0.29268 &
  0.38443 &
  0.53237 &
  0.66124 &
  0.14143 &
  0.20662 &
  0.22746 &
  0.24731 &
  0.25636 \\ \hline
\cellcolor[HTML]{333333}{\color[HTML]{FFFFFF} } &
  \multicolumn{5}{c|}{\textbf{HR@}} &
  \multicolumn{5}{c|}{\textbf{MRR@}} \\ \cline{2-11} 
\multirow{-2}{*}{\cellcolor[HTML]{333333}{\color[HTML]{FFFFFF} \textbf{CIKMCUP}}} &
  \textbf{1} &
  \textbf{3} &
  \textbf{5} &
  \textbf{10} &
  \textbf{20} &
  \textbf{1} &
  \textbf{3} &
  \textbf{5} &
  \textbf{10} &
  \textbf{20} \\ \hline
\textbf{S-POP} &
  0.03808 &
  0.09823 &
  0.1137 &
  0.12163 &
  0.12229 &
  0.03808 &
  0.06443 &
  0.06799 &
  0.06914 &
  0.06919 \\
\textbf{AR} &
  0.03781 &
  0.08911 &
  0.12731 &
  0.18496 &
  0.18522 &
  0.03781 &
  0.05938 &
  0.06803 &
  0.07599 &
  0.07601 \\
\textbf{SR} &
  0.03609 &
  0.0817 &
  0.10986 &
  0.16631 &
  0.22025 &
  0.03609 &
  0.05539 &
  0.06181 &
  0.06943 &
  0.07322 \\
\textbf{VSKNN} &
  0.05006 & 0.09606 & 0.12706 & 0.16433 & 0.20701 & 0.05006 & 0.07007 & 0.07717 & 0.08218 & 0.08516 \\
\textbf{SMF} &
  0.03597 &
  0.09279 &
  0.13817 &
  0.22414 &
  0.3386 &
  0.03597 &
  0.05977 &
  0.07005 &
  0.08132 &
  0.08921 \\
\textbf{Item2Vec} &
  0.02148 &
  0.04719 &
  0.06801 &
  0.10584 &
  0.16054 &
  0.02148 &
  0.03245 &
  0.03716 &
  0.04206 &
  0.04584 \\
\textbf{GRU4Rec+} &
  0.02366 &
  0.06237 &
  0.09798 &
  0.15968 &
  0.24153 &
  0.02366 &
  0.04005 &
  0.048 &
  0.05601 &
  0.06161 \\
\textbf{NARM} &
  0.04279 &
  0.11939 &
  0.18348 &
  0.29642 &
  0.49613 &
  0.04279 &
  0.07397 &
  0.0897 &
  0.1037 &
  0.11496 \\
\textbf{STAMP} &
  0.05061 &
  0.13103 &
  0.18448 &
  0.30132 &
  0.41958 &
  0.05061 &
  0.08578 &
  0.09796 &
  0.11344 &
  0.12157 \\
\textbf{NextItNet} &
  0.03207 &
  0.05984 &
  0.07946 &
  0.1259 &
  0.1843 &
  0.03207 &
  0.04404 &
  0.0484 &
  0.0544 &
  0.05842 \\
\textbf{SRGNN} &
  0.06144 &
  0.14825 &
  0.21139 &
  0.32131 &
  0.44025 &
  0.06144 &
  0.09902 &
  0.11323 &
  0.12809 &
  0.13647 \\
\textbf{CSRM} &
  0.06061 &
  0.13853 &
  0.19913 &
  0.30303 &
  0.42352 &
  0.06061 &
  0.09355 &
  0.10734 &
  0.12104 &
  0.12932 \\ \hline
\cellcolor[HTML]{333333}{\color[HTML]{FFFFFF} } &
  \multicolumn{5}{c|}{\textbf{HR@}} &
  \multicolumn{5}{c|}{\textbf{MRR@}} \\ \cline{2-11} 
\multirow{-2}{*}{\cellcolor[HTML]{333333}{\color[HTML]{FFFFFF} \textbf{TMALL}}} &
  \textbf{1} &
  \textbf{3} &
  \textbf{5} &
  \textbf{10} &
  \textbf{20} &
  \textbf{1} &
  \textbf{3} &
  \textbf{5} &
  \textbf{10} &
  \textbf{20} \\ \hline
\textbf{S-POP} &
  0.04786 &
  0.11212 &
  0.14145 &
  0.17235 &
  0.18893 &
  0.04786 &
  0.04786 &
  0.04786 &
  0.04786 &
  0.04786 \\
\textbf{AR} &
  0.01193 &
  0.02584 &
  0.0349 &
  0.04775 &
  0.04803 &
  0.01193 &
  0.01791 &
  0.01996 &
  0.02174 &
  0.02176 \\
\textbf{SR} &
  0.01131 &
  0.02331 &
  0.03048 &
  0.0419 &
  0.05356 &
  0.01131 &
  0.01638 &
  0.018 &
  0.01952 &
  0.02034 \\
\textbf{VSKNN} &
  0.03898 & 0.05936 & 0.07050 & 0.08488 & 0.10198 & 0.03898 & 0.04813 & 0.05053 & 0.05233 & 0.05348 \\
\textbf{SMF} &
  0.01576 &
  0.03863 &
  0.0535 &
  0.07881 &
  0.11158 &
  0.01576 &
  0.0255 &
  0.02885 &
  0.03222 &
  0.03448 \\
\textbf{Item2Vec} &
  0.00262 &
  0.00638 &
  0.00896 &
  0.01432 &
  0.02166 &
  0.00262 &
  0.00422 &
  0.0048 &
  0.0055 &
  0.006 \\
\textbf{GRU4Rec+} &
  0.01501 &
  0.03553 &
  0.04791 &
  0.06812 &
  0.08859 &
  0.01501 &
  0.02369 &
  0.02649 &
  0.02922 &
  0.03063 \\
\textbf{NARM} &
  0.02221 &
  0.05435 &
  0.07404 &
  0.10642 &
  0.15955 &
  0.02221 &
  0.03541 &
  0.0406 &
  0.04471 &
  0.04779 \\
\textbf{STAMP} &
  0.04522 &
  0.09184 &
  0.11527 &
  0.15435 &
  0.19446 &
  0.04522 &
  0.06542 &
  0.07073 &
  0.07592 &
  0.07873 \\
\textbf{NextItNet} &
  0.00722 &
  0.01445 &
  0.01892 &
  0.02763 &
  0.03612 &
  0.00722 &
  0.01047 &
  0.01148 &
  0.01264 &
  0.01324 \\
\textbf{SRGNN} &
  0.03601 &
  0.07434 &
  0.09503 &
  0.12623 &
  0.16066 &
  0.03601 &
  0.05252 &
  0.05718 &
  0.06135 &
  0.06373 \\
\textbf{CSRM} &
  0.02447 &
  0.0472 &
  0.06335 &
  0.08831 &
  0.11705 &
  0.02447 &
  0.03424 &
  0.03792 &
  0.04123 &
  0.04322 \\ \hline
\cellcolor[HTML]{333333}{\color[HTML]{FFFFFF} } &
  \multicolumn{5}{c|}{\textbf{HR@}} &
  \multicolumn{5}{c|}{\textbf{MRR@}} \\ \cline{2-11} 
\multirow{-2}{*}{\cellcolor[HTML]{333333}{\color[HTML]{FFFFFF} \textbf{ROCKET}}} &
  \textbf{1} &
  \textbf{3} &
  \textbf{5} &
  \textbf{10} &
  \textbf{20} &
  \textbf{1} &
  \textbf{3} &
  \textbf{5} &
  \textbf{10} &
  \textbf{20} \\ \hline
\textbf{S-POP} &
  0.03542 &
  0.09596 &
  0.11253 &
  0.12082 &
  0.12334 &
  0.03542 &
  0.06309 &
  0.06696 &
  0.06812 &
  0.06831 \\
\textbf{AR} &
  0.04572 &
  0.08616 &
  0.11454 &
  0.15172 &
  0.15197 &
  0.04572 &
  0.06284 &
  0.06922 &
  0.07424 &
  0.07425 \\
\textbf{SR} &
  0.04245 &
  0.08541 &
  0.1158 &
  0.15398 &
  0.18915 &
  0.04245 &
  0.06083 &
  0.06783 &
  0.07302 &
  0.07551 \\
\textbf{VSKNN} &
  0.12192 & 0.17954 & 0.20077 & 0.22362 & 0.24788 & 0.12192 & 0.14753 & 0.15238 & 0.15546 & 0.15723 \\
\textbf{SMF} &
  0.028 &
  0.08747 &
  0.13227 &
  0.20427 &
  0.27093 &
  0.028 &
  0.05378 &
  0.06403 &
  0.07365 &
  0.07821 \\
\textbf{Item2Vec} &
  0.0202 &
  0.04339 &
  0.05686 &
  0.08379 &
  0.11746 &
  0.0202 &
  0.03005 &
  0.03315 &
  0.03661 &
  0.03888 \\
\textbf{GRU4Rec+} &
  0.05248 &
  0.10839 &
  0.14689 &
  0.20042 &
  0.25185 &
  0.05248 &
  0.07652 &
  0.08526 &
  0.09237 &
  0.09591 \\
\textbf{NARM} &
  0.11779 &
  0.22135 &
  0.27157 &
  0.30696 &
  0.41763 &
  0.11779 &
  0.1769 &
  0.18172 &
  0.1856 &
  0.19288 \\
\textbf{STAMP} &
  0.07227 &
  0.13281 &
  0.1875 &
  0.25781 &
  0.33203 &
  0.07227 &
  0.09928 &
  0.11198 &
  0.12193 &
  0.12685 \\
\textbf{NextItNet} &
  0.07466 &
  0.13784 &
  0.17422 &
  0.22591 &
  0.26867 &
  0.07466 &
  0.10083 &
  0.10913 &
  0.11591 &
  0.11893 \\
\textbf{SRGNN} &
  0.09898 &
  0.18528 &
  0.21574 &
  0.25888 &
  0.31472 &
  0.09898 &
  0.13536 &
  0.14222 &
  0.14772 &
  0.15166 \\
\textbf{CSRM} &
  0.08889 &
  0.22963 &
  0.25185 &
  0.31852 &
  0.4 &
  0.08889 &
  0.15185 &
  0.15667 &
  0.16503 &
  0.17032 \\ \hline
\end{tabular}}
\label{tab:freq-high}
\end{table*}
