# Supplementary material for: Comprehensive Empirical Evaluation of Deep Learning Approaches for Session-based Recommendation in E-Commerce
Source: arXiv:2010.12540 source file (2020-10-17)
Supplement: Supplementary file 7 [file tab4.tex]

\begin{table*}[!h]
\centering
\caption{RQ2: testing using short sessions of length \textless 5}
\resizebox{0.9\textwidth}{!}{\begin{tabular}{|c|ccccc|ccccc|}
\hline
\cellcolor[HTML]{333333}{\color[HTML]{FFFFFF} } &
  \multicolumn{5}{c|}{\textbf{HR@}} &
  \multicolumn{5}{c|}{\textbf{MRR@}} \\ \cline{2-11} 
\multirow{-2}{*}{\cellcolor[HTML]{333333}{\color[HTML]{FFFFFF} \textbf{RECSYS}}} &
  \textbf{1} &
  \textbf{3} &
  \textbf{5} &
  \textbf{10} &
  \textbf{20} &
  \textbf{1} &
  \textbf{3} &
  \textbf{5} &
  \textbf{10} &
  \textbf{20} \\ \hline
\textbf{S-POP} &
  0.0269 &
  0.05629 &
  0.07384 &
  0.10915 &
  0.13707 &
  0.0269 &
  0.04088 &
  0.04449 &
  0.04974 &
  0.0514 \\
\textbf{AR} &
  0.17392 &
  0.31574 &
  0.38767 &
  0.47335 &
  0.47525 &
  0.17392 &
  0.23582 &
  0.25205 &
  0.26409 &
  0.26422 \\
\textbf{SR} &
  0.1734 &
  0.31706 &
  0.39096 &
  0.49258 &
  0.57665 &
  0.1734 &
  0.23595 &
  0.25272 &
  0.26642 &
  0.27228 \\
\textbf{VSKNN} &
  0.15971 & 0.30883 & 0.36927 & 0.42770 & 0.47628 & 0.15971 & 0.22525 & 0.23924 & 0.24706 & 0.25050 \\
\textbf{SMF} &
  0.09855 &
  0.24571 &
  0.34652 &
  0.48278 &
  0.58805 &
  0.09855 &
  0.16094 &
  0.18395 &
  0.20227 &
  0.20969 \\
\textbf{Item2Vec} &
  0.0996 &
  0.19145 &
  0.24224 &
  0.32531 &
  0.42594 &
  0.0996 &
  0.13983 &
  0.15142 &
  0.1626 &
  0.16957 \\
\textbf{GRU4Rec+} &
  0.10461 &
  0.22054 &
  0.29743 &
  0.41623 &
  0.53429 &
  0.10461 &
  0.15432 &
  0.17157 &
  0.18724 &
  0.19558 \\
\textbf{NARM} &
  0.15464 &
  0.31151 &
  0.39978 &
  0.51841 &
  0.67293 &
  0.15464 &
  0.2238 &
  0.24387 &
  0.2597 &
  0.26937 \\
\textbf{STAMP} &
  0.17596 &
  0.33125 &
  0.40926 &
  0.51956 &
  0.62162 &
  0.17596 &
  0.24344 &
  0.26132 &
  0.27606 &
  0.2832 \\
\textbf{NextItNet} &
  0.17636 &
  0.33789 &
  0.40924 &
  0.50632 &
  0.608 &
  0.17636 &
  0.24684 &
  0.26304 &
  0.27599 &
  0.28312 \\
\textbf{SRGNN} &
  0.18954 &
  0.35229 &
  0.4302 &
  0.54235 &
  0.64055 &
  0.18954 &
  0.26043 &
  0.27815 &
  0.29307 &
  0.29991 \\
\textbf{CSRM} &
  0.19072 &
  0.35588 &
  0.43302 &
  0.54522 &
  0.6534 &
  0.19072 &
  0.26177 &
  0.27919 &
  0.29413 &
  0.3017 \\ \hline
\cellcolor[HTML]{333333}{\color[HTML]{FFFFFF} } &
  \multicolumn{5}{c|}{\textbf{HR@}} &
  \multicolumn{5}{c|}{\textbf{MRR@}} \\ \cline{2-11} 
\multirow{-2}{*}{\cellcolor[HTML]{333333}{\color[HTML]{FFFFFF} \textbf{CIKMCUP}}} &
  \textbf{1} &
  \textbf{3} &
  \textbf{5} &
  \textbf{10} &
  \textbf{20} &
  \textbf{1} &
  \textbf{3} &
  \textbf{5} &
  \textbf{10} &
  \textbf{20} \\ \hline
\textbf{S-POP} &
  0.02893 &
  0.05944 &
  0.06207 &
  0.06575 &
  0.06996 &
  0.02893 &
  0.04322 &
  0.04385 &
  0.04437 &
  0.04466 \\
\textbf{AR} &
  0.05786 &
  0.13519 &
  0.18727 &
  0.26355 &
  0.26407 &
  0.05786 &
  0.09022 &
  0.10216 &
  0.11283 &
  0.11286 \\
\textbf{SR} &
  0.05734 &
  0.13046 &
  0.17307 &
  0.24934 &
  0.31352 &
  0.05734 &
  0.0889 &
  0.09832 &
  0.10844 &
  0.11295 \\
\textbf{VSKNN} &
  0.08068 & 0.15030 & 0.18488 & 0.23651 & 0.27294 & 0.08068 & 0.11119 & 0.11907 & 0.12592 & 0.12848 \\
\textbf{SMF} &
  0.04085 &
  0.11088 &
  0.16446 &
  0.25517 &
  0.3687 &
  0.04085 &
  0.06985 &
  0.08197 &
  0.09375 &
  0.10166 \\
\textbf{Item2Vec} &
  0.03019 &
  0.06091 &
  0.08369 &
  0.13294 &
  0.19439 &
  0.03019 &
  0.04352 &
  0.04861 &
  0.05515 &
  0.05938 \\
\textbf{GRU4Rec+} &
  0.03568 &
  0.08185 &
  0.11752 &
  0.19465 &
  0.26915 &
  0.03568 &
  0.05526 &
  0.06347 &
  0.07358 &
  0.07852 \\
\textbf{NARM} &
  0.05892 &
  0.14541 &
  0.18182 &
  0.26581 &
  0.44966 &
  0.05892 &
  0.0973 &
  0.10568 &
  0.11676 &
  0.12762 \\
\textbf{STAMP} &
  0.04158 &
  0.10474 &
  0.15474 &
  0.25 &
  0.35632 &
  0.04158 &
  0.06833 &
  0.07936 &
  0.09199 &
  0.09923 \\
\textbf{NextItNet} &
  0.03125 &
  0.07031 &
  0.09462 &
  0.14583 &
  0.19792 &
  0.03125 &
  0.04745 &
  0.05279 &
  0.05975 &
  0.0634 \\
\textbf{SRGNN} &
  0.05573 &
  0.13177 &
  0.19062 &
  0.28906 &
  0.39844 &
  0.05573 &
  0.08811 &
  0.10134 &
  0.11433 &
  0.12186 \\
\textbf{CSRM} &
  0.05247 &
  0.12697 &
  0.17629 &
  0.26443 &
  0.38143 &
  0.05247 &
  0.08377 &
  0.09492 &
  0.10656 &
  0.11459 \\ \hline
\cellcolor[HTML]{333333}{\color[HTML]{FFFFFF} } &
  \multicolumn{5}{c|}{\textbf{HR@}} &
  \multicolumn{5}{c|}{\textbf{MRR@}} \\ \cline{2-11} 
\multirow{-2}{*}{\cellcolor[HTML]{333333}{\color[HTML]{FFFFFF} \textbf{TMALL}}} &
  \textbf{1} &
  \textbf{3} &
  \textbf{5} &
  \textbf{10} &
  \textbf{20} &
  \textbf{1} &
  \textbf{3} &
  \textbf{5} &
  \textbf{10} &
  \textbf{20} \\ \hline
\textbf{S-POP} &
  0.02761 &
  0.05606 &
  0.05817 &
  0.0588 &
  0.06217 &
  0.02761 &
  0.02761 &
  0.02761 &
  0.02761 &
  0.02761 \\
\textbf{AR} &
  0.03477 &
  0.06913 &
  0.08851 &
  0.11697 &
  0.11823 &
  0.03477 &
  0.04946 &
  0.05383 &
  0.05766 &
  0.05776 \\
\textbf{SR} &
  0.03288 &
  0.06238 &
  0.07861 &
  0.10411 &
  0.1294 &
  0.03288 &
  0.04549 &
  0.04914 &
  0.05258 &
  0.05434 \\
\textbf{VSKNN} &
  0.09997 & 0.12910 & 0.14484 & 0.16661 & 0.17883 & 0.09997 & 0.11319 & 0.11678 & 0.11973 & 0.12058 \\
\textbf{SMF} &
  0.02065 &
  0.05248 &
  0.06913 &
  0.09589 &
  0.12919 &
  0.02065 &
  0.034 &
  0.03776 &
  0.04132 &
  0.04363 \\
\textbf{Item2Vec} &
  0.00889 &
  0.01948 &
  0.02605 &
  0.03558 &
  0.0521 &
  0.00889 &
  0.01324 &
  0.01472 &
  0.016 &
  0.01717 \\
\textbf{GRU4Rec+} &
  0.01466 &
  0.04168 &
  0.05928 &
  0.08421 &
  0.11437 &
  0.01466 &
  0.02615 &
  0.03018 &
  0.03355 &
  0.03567 \\
\textbf{NARM} &
  0.03504 &
  0.08759 &
  0.11503 &
  0.15281 &
  0.21064 &
  0.03504 &
  0.05794 &
  0.06421 &
  0.06928 &
  0.07271 \\
\textbf{STAMP} &
  0.03562 &
  0.08706 &
  0.11151 &
  0.14798 &
  0.17917 &
  0.03562 &
  0.05811 &
  0.06363 &
  0.06854 &
  0.07069 \\
\textbf{NextItNet} &
  0.01075 &
  0.01949 &
  0.02386 &
  0.02923 &
  0.04671 &
  0.01075 &
  0.01434 &
  0.01531 &
  0.0161 &
  0.01731 \\
\textbf{SRGNN} &
  0.04564 &
  0.09642 &
  0.12027 &
  0.15481 &
  0.19038 &
  0.04564 &
  0.06781 &
  0.07332 &
  0.078 &
  0.08042 \\
\textbf{CSRM} &
  0.03145 &
  0.06501 &
  0.0859 &
  0.11207 &
  0.14436 &
  0.03145 &
  0.04591 &
  0.05066 &
  0.05417 &
  0.05642 \\ \hline
\cellcolor[HTML]{333333}{\color[HTML]{FFFFFF} } &
  \multicolumn{5}{c|}{\textbf{HR@}} &
  \multicolumn{5}{c|}{\textbf{MRR@}} \\ \cline{2-11} 
\multirow{-2}{*}{\cellcolor[HTML]{333333}{\color[HTML]{FFFFFF} \textbf{ROCKET}}} &
  \textbf{1} &
  \textbf{3} &
  \textbf{5} &
  \textbf{10} &
  \textbf{20} &
  \textbf{1} &
  \textbf{3} &
  \textbf{5} &
  \textbf{10} &
  \textbf{20} \\ \hline
\textbf{S-POP} &
  0.03014 &
  0.08856 &
  0.09225 &
  0.09902 &
  0.11009 &
  0.03014 &
  0.05822 &
  0.05905 &
  0.05989 &
  0.06071 \\
\textbf{AR} &
  0.09533 &
  0.1845 &
  0.22263 &
  0.26876 &
  0.26876 &
  0.09533 &
  0.13448 &
  0.14306 &
  0.14961 &
  0.14961 \\
\textbf{SR} &
  0.08672 &
  0.16913 &
  0.19926 &
  0.23247 &
  0.25953 &
  0.08672 &
  0.12157 &
  0.12845 &
  0.13292 &
  0.13481 \\
\textbf{VSKNN} &
  0.20636 & 0.30220 & 0.33197 & 0.35971 & 0.38091 & 0.20636 & 0.24871 & 0.25566 & 0.25947 & 0.26095 \\
\textbf{SMF} &
  0.07011 &
  0.16052 &
  0.21956 &
  0.29705 &
  0.37023 &
  0.07011 &
  0.10978 &
  0.12352 &
  0.13405 &
  0.13922 \\
\textbf{Item2Vec} &
  0.02928 &
  0.06938 &
  0.09039 &
  0.13622 &
  0.17314 &
  0.02928 &
  0.04657 &
  0.05138 &
  0.05762 &
  0.06023 \\
\textbf{GRU4Rec+} &
  0.0805 &
  0.15108 &
  0.18638 &
  0.23653 &
  0.27678 &
  0.0805 &
  0.11053 &
  0.11851 &
  0.12523 &
  0.12801 \\
\textbf{NARM} &
  0.12316 &
  0.22037 &
  0.26322 &
  0.32652 &
  0.39736 &
  0.12316 &
  0.16441 &
  0.1743 &
  0.18262 &
  0.18678 \\
\textbf{STAMP} &
  0.08452 &
  0.1504 &
  0.19888 &
  0.25855 &
  0.31448 &
  0.08452 &
  0.11239 &
  0.12361 &
  0.13162 &
  0.13567 \\
\textbf{NextItNet} &
  0.05574 &
  0.08699 &
  0.10473 &
  0.13682 &
  0.15963 &
  0.05574 &
  0.06898 &
  0.07328 &
  0.07751 &
  0.07914 \\
\textbf{SRGNN} &
  0.08954 &
  0.17428 &
  0.21755 &
  0.27284 &
  0.31971 &
  0.08954 &
  0.1271 &
  0.13708 &
  0.14461 &
  0.14785 \\
\textbf{CSRM} &
  0.1105 &
  0.20036 &
  0.25015 &
  0.31876 &
  0.36551 &
  0.1105 &
  0.14835 &
  0.15998 &
  0.16888 &
  0.17209 \\ \hline
\end{tabular}}
\label{tab:test-short}
\end{table*}
