# Supplementary material for: Comprehensive Empirical Evaluation of Deep Learning Approaches for Session-based Recommendation in E-Commerce
Source: arXiv:2010.12540 source file (2020-10-17)
Supplement: Supplementary file 8 [file tab5.tex]

\begin{table*}[!h]
\centering
\caption{RQ2: testing using intermediate sessions of length \textgreater= 5 and \textless10}
\resizebox{0.9\textwidth}{!}{\begin{tabular}{|c|ccccc|ccccc|}
\hline
\cellcolor[HTML]{333333}{\color[HTML]{FFFFFF} } &
  \multicolumn{5}{c|}{\textbf{HR@}} &
  \multicolumn{5}{c|}{\textbf{MRR@}} \\ \cline{2-11} 
\multirow{-2}{*}{\cellcolor[HTML]{333333}{\color[HTML]{FFFFFF} \textbf{RECSYS}}} &
  \textbf{1} &
  \textbf{3} &
  \textbf{5} &
  \textbf{10} &
  \textbf{20} &
  \textbf{1} &
  \textbf{3} &
  \textbf{5} &
  \textbf{10} &
  \textbf{20} \\ \hline
\textbf{S-POP} &
  0.04456 &
  0.12103 &
  0.14258 &
  0.16652 &
  0.18302 &
  0.04456 &
  0.07841 &
  0.08335 &
  0.08661 &
  0.08764 \\
\textbf{AR} &
  0.11452 &
  0.23455 &
  0.30338 &
  0.37567 &
  0.37793 &
  0.11452 &
  0.16585 &
  0.18148 &
  0.1917 &
  0.19186 \\
\textbf{SR} &
  0.11545 &
  0.23535 &
  0.30644 &
  0.40121 &
  0.49591 &
  0.11545 &
  0.16684 &
  0.18307 &
  0.19571 &
  0.20234 \\
\textbf{VSKNN} &
  0.10486 & 0.23228 & 0.29541 & 0.38039 & 0.45762 & 0.10486 & 0.15992 & 0.17427 & 0.18568 & 0.19106 \\
\textbf{SMF} &
  0.0796 &
  0.20529 &
  0.29268 &
  0.43573 &
  0.57093 &
  0.0796 &
  0.13302 &
  0.15282 &
  0.17191 &
  0.18148 \\
\textbf{Item2Vec} &
  0.07452 &
  0.1432 &
  0.18583 &
  0.26385 &
  0.35502 &
  0.07452 &
  0.10403 &
  0.1136 &
  0.12408 &
  0.13028 \\
\textbf{GRU4Rec+} &
  0.07385 &
  0.17894 &
  0.25613 &
  0.39058 &
  0.5273 &
  0.07385 &
  0.11864 &
  0.13615 &
  0.154 &
  0.16359 \\
\textbf{NARM} &
  0.1143 &
  0.28252 &
  0.38658 &
  0.53892 &
  0.72268 &
  0.1143 &
  0.1867 &
  0.21054 &
  0.23086 &
  0.24239 \\
\textbf{STAMP} &
  0.13134 &
  0.27368 &
  0.36166 &
  0.49068 &
  0.61303 &
  0.13134 &
  0.19256 &
  0.21244 &
  0.22966 &
  0.23817 \\
\textbf{NextItNet} &
  0.1424 &
  0.27738 &
  0.36179 &
  0.4797 &
  0.59343 &
  0.1424 &
  0.20135 &
  0.22057 &
  0.23623 &
  0.24415 \\
\textbf{SRGNN} &
  0.13486 &
  0.28688 &
  0.37851 &
  0.51026 &
  0.64109 &
  0.13486 &
  0.19957 &
  0.22035 &
  0.23786 &
  0.247 \\
\textbf{CSRM} &
  0.16494 &
  0.32902 &
  0.41941 &
  0.5561 &
  0.68058 &
  0.16494 &
  0.23577 &
  0.25634 &
  0.27463 &
  0.28335 \\ \hline
\cellcolor[HTML]{333333}{\color[HTML]{FFFFFF} } &
  \multicolumn{5}{c|}{\textbf{HR@}} &
  \multicolumn{5}{c|}{\textbf{MRR@}} \\ \cline{2-11} 
\multirow{-2}{*}{\cellcolor[HTML]{333333}{\color[HTML]{FFFFFF} \textbf{CIKMCUP}}} &
  \textbf{1} &
  \textbf{3} &
  \textbf{5} &
  \textbf{10} &
  \textbf{20} &
  \textbf{1} &
  \textbf{3} &
  \textbf{5} &
  \textbf{10} &
  \textbf{20} \\ \hline
\textbf{S-POP} &
  0.04262 &
  0.10037 &
  0.11427 &
  0.11705 &
  0.1223 &
  0.04262 &
  0.06861 &
  0.07187 &
  0.07226 &
  0.07262 \\
\textbf{AR} &
  0.04663 &
  0.11087 &
  0.15503 &
  0.22051 &
  0.22051 &
  0.04663 &
  0.07376 &
  0.08386 &
  0.09285 &
  0.09285 \\
\textbf{SR} &
  0.0454 &
  0.10222 &
  0.13897 &
  0.20754 &
  0.26467 &
  0.0454 &
  0.06949 &
  0.07778 &
  0.08697 &
  0.09085 \\
\textbf{VSKNN} &
  0.06231 & 0.12067 & 0.16070 & 0.21962 & 0.26924 & 0.06231 & 0.08768 & 0.09674 & 0.10474 & 0.10810 \\
\textbf{SMF} &
  0.04716 &
  0.11077 &
  0.16972 &
  0.25939 &
  0.37388 &
  0.04716 &
  0.07405 &
  0.08744 &
  0.09933 &
  0.10722 \\
\textbf{Item2Vec} &
  0.02227 &
  0.0464 &
  0.06619 &
  0.10145 &
  0.14383 &
  0.02227 &
  0.03258 &
  0.03696 &
  0.04149 &
  0.0443 \\
\textbf{GRU4Rec+} &
  0.02978 &
  0.07369 &
  0.11022 &
  0.18238 &
  0.27326 &
  0.02978 &
  0.04856 &
  0.05678 &
  0.06613 &
  0.07239 \\
\textbf{NARM} &
  0.05508 &
  0.12937 &
  0.1728 &
  0.27023 &
  0.47843 &
  0.05508 &
  0.08522 &
  0.09507 &
  0.10776 &
  0.12012 \\
\textbf{STAMP} &
  0.03922 &
  0.09852 &
  0.15195 &
  0.24768 &
  0.34713 &
  0.03922 &
  0.06408 &
  0.07619 &
  0.08865 &
  0.09551 \\
\textbf{NextItNet} &
  0.02699 &
  0.06108 &
  0.08665 &
  0.13352 &
  0.1946 &
  0.02699 &
  0.04119 &
  0.04716 &
  0.05342 &
  0.0576 \\
\textbf{SRGNN} &
  0.04748 &
  0.1226 &
  0.18269 &
  0.28666 &
  0.40385 &
  0.04748 &
  0.07868 &
  0.09253 &
  0.10597 &
  0.11409 \\
\textbf{CSRM} &
  0.04775 &
  0.11922 &
  0.16913 &
  0.27418 &
  0.39526 &
  0.04775 &
  0.07779 &
  0.08908 &
  0.10294 &
  0.11121 \\ \hline
\cellcolor[HTML]{333333}{\color[HTML]{FFFFFF} } &
  \multicolumn{5}{c|}{\textbf{HR@}} &
  \multicolumn{5}{c|}{\textbf{MRR@}} \\ \cline{2-11} 
\multirow{-2}{*}{\cellcolor[HTML]{333333}{\color[HTML]{FFFFFF} \textbf{TMALL}}} &
  \textbf{1} &
  \textbf{3} &
  \textbf{5} &
  \textbf{10} &
  \textbf{20} &
  \textbf{1} &
  \textbf{3} &
  \textbf{5} &
  \textbf{10} &
  \textbf{20} \\ \hline
\textbf{S-POP} &
  0.05123 &
  0.12518 &
  0.14093 &
  0.14428 &
  0.14665 &
  0.05123 &
  0.05123 &
  0.05123 &
  0.05123 &
  0.05123 \\
\textbf{AR} &
  0.02121 &
  0.04393 &
  0.05766 &
  0.07711 &
  0.07799 &
  0.02121 &
  0.03093 &
  0.03403 &
  0.03674 &
  0.03681 \\
\textbf{SR} &
  0.02095 &
  0.04252 &
  0.05352 &
  0.06998 &
  0.08697 &
  0.02095 &
  0.03025 &
  0.03276 &
  0.03494 &
  0.03615 \\
\textbf{VSKNN} &
  0.07838 & 0.11025 & 0.12595 & 0.14634 & 0.16507 & 0.07838 & 0.09236 & 0.09593 & 0.09864 & 0.09994 \\
\textbf{SMF} &
  0.02007 &
  0.05079 &
  0.06787 &
  0.09613 &
  0.12614 &
  0.02007 &
  0.03316 &
  0.03706 &
  0.04084 &
  0.04292 \\
\textbf{Item2Vec} &
  0.00378 &
  0.0109 &
  0.01485 &
  0.02364 &
  0.03498 &
  0.00378 &
  0.00688 &
  0.00778 &
  0.00891 &
  0.00968 \\
\textbf{GRU4Rec+} &
  0.01898 &
  0.04292 &
  0.05955 &
  0.08602 &
  0.11127 &
  0.01898 &
  0.02899 &
  0.03272 &
  0.03627 &
  0.03805 \\
\textbf{NARM} &
  0.04579 &
  0.09158 &
  0.11868 &
  0.15649 &
  0.2157 &
  0.04579 &
  0.06541 &
  0.07165 &
  0.07673 &
  0.08021 \\
\textbf{STAMP} &
  0.04454 &
  0.08636 &
  0.1088 &
  0.1404 &
  0.17245 &
  0.04454 &
  0.06259 &
  0.0677 &
  0.07197 &
  0.0742 \\
\textbf{NextItNet} &
  0.00781 &
  0.0186 &
  0.02716 &
  0.03609 &
  0.0506 &
  0.00781 &
  0.01271 &
  0.01463 &
  0.01579 &
  0.01677 \\
\textbf{SRGNN} &
  0.0553 &
  0.09867 &
  0.1221 &
  0.15344 &
  0.18706 &
  0.0553 &
  0.07423 &
  0.07965 &
  0.08382 &
  0.08615 \\
\textbf{CSRM} &
  0.03386 &
  0.06456 &
  0.08377 &
  0.11193 &
  0.14018 &
  0.03386 &
  0.0469 &
  0.05133 &
  0.05508 &
  0.05705 \\ \hline
\cellcolor[HTML]{333333}{\color[HTML]{FFFFFF} } &
  \multicolumn{5}{c|}{\textbf{HR@}} &
  \multicolumn{5}{c|}{\textbf{MRR@}} \\ \cline{2-11} 
\multirow{-2}{*}{\cellcolor[HTML]{333333}{\color[HTML]{FFFFFF} \textbf{ROCKET}}} &
  \textbf{1} &
  \textbf{3} &
  \textbf{5} &
  \textbf{10} &
  \textbf{20} &
  \textbf{1} &
  \textbf{3} &
  \textbf{5} &
  \textbf{10} &
  \textbf{20} \\ \hline
\textbf{S-POP} &
  0.05278 &
  0.14352 &
  0.16759 &
  0.175 &
  0.18056 &
  0.05278 &
  0.09259 &
  0.09838 &
  0.09938 &
  0.09976 \\
\textbf{AR} &
  0.0537 &
  0.10278 &
  0.13241 &
  0.16019 &
  0.16204 &
  0.0537 &
  0.07562 &
  0.08228 &
  0.08608 &
  0.08618 \\
\textbf{SR} &
  0.04537 &
  0.09167 &
  0.12037 &
  0.14074 &
  0.16481 &
  0.04537 &
  0.06528 &
  0.07194 &
  0.07478 &
  0.07658 \\
\textbf{VSKNN} &
  0.13689 & 0.25213 & 0.29157 & 0.33952 & 0.37200 & 0.13689 & 0.18600 & 0.19520 & 0.20155 & 0.20380 \\
\textbf{SMF} &
  0.03796 &
  0.11481 &
  0.15556 &
  0.21759 &
  0.30463 &
  0.03796 &
  0.07176 &
  0.08088 &
  0.08902 &
  0.0949 \\
\textbf{Item2Vec} &
  0.02908 &
  0.05816 &
  0.0666 &
  0.09568 &
  0.12101 &
  0.02908 &
  0.04112 &
  0.04295 &
  0.04662 &
  0.04842 \\
\textbf{GRU4Rec+} &
  0.03568 &
  0.086 &
  0.12534 &
  0.16377 &
  0.20037 &
  0.03568 &
  0.05764 &
  0.06665 &
  0.07158 &
  0.07411 \\
\textbf{NARM} &
  0.05778 &
  0.15252 &
  0.19321 &
  0.24591 &
  0.36052 &
  0.05778 &
  0.09898 &
  0.10842 &
  0.11552 &
  0.1222 \\
\textbf{STAMP} &
  0.04171 &
  0.09546 &
  0.13902 &
  0.1835 &
  0.23355 &
  0.04171 &
  0.06518 &
  0.07547 &
  0.08129 &
  0.08475 \\
\textbf{NextItNet} &
  0.01562 &
  0.03906 &
  0.04688 &
  0.05469 &
  0.08203 &
  0.01562 &
  0.02669 &
  0.02845 &
  0.02954 &
  0.03144 \\
\textbf{SRGNN} &
  0.05382 &
  0.1224 &
  0.16059 &
  0.2066 &
  0.25694 &
  0.05382 &
  0.08333 &
  0.09193 &
  0.09824 &
  0.10176 \\
\textbf{CSRM} &
  0.06938 &
  0.14246 &
  0.18316 &
  0.24977 &
  0.29787 &
  0.06938 &
  0.1013 &
  0.11055 &
  0.11956 &
  0.12283 \\ \hline
\end{tabular}}
\label{tab:test-intermediate}
\end{table*}
