# Supplementary material for: Comprehensive Empirical Evaluation of Deep Learning Approaches for Session-based Recommendation in E-Commerce
Source: arXiv:2010.12540 source file (2020-10-17)
Supplement: Supplementary file 9 [file tab13.tex]

% Please add the following required packages to your document preamble:
% \usepackage{multirow}
% \usepackage[table,xcdraw]{xcolor}
% If you use beamer only pass "xcolor=table" option, i.e. \documentclass[xcolor=table]{beamer}
\begin{table*}[!h]
\centering
\caption{RQ6: training using sessions of the most recent 30 days before the testing set.}
\resizebox{0.9\textwidth}{!}{\begin{tabular}{|c|ccccc|ccccc|}
\hline
\cellcolor[HTML]{333333}{\color[HTML]{FFFFFF} } &
  \multicolumn{5}{c|}{\textbf{HR@}} &
  \multicolumn{5}{c|}{\textbf{MRR@}} \\ \cline{2-11} 
\multirow{-2}{*}{\cellcolor[HTML]{333333}{\color[HTML]{FFFFFF} \textbf{RECSYS}}} &
  \textbf{1} &
  \textbf{3} &
  \textbf{5} &
  \textbf{10} &
  \textbf{20} &
  \textbf{1} &
  \textbf{3} &
  \textbf{5} &
  \textbf{10} &
  \textbf{20} \\ \hline
\textbf{S-POP} &
  0.03596 &
  0.09942 &
  0.12356 &
  0.14465 &
  0.15653 &
  0.03596 &
  0.06387 &
  0.0694 &
  0.07234 &
  0.07318 \\
\textbf{AR} &
  0.11756 &
  0.22679 &
  0.28838 &
  0.3558 &
  0.35688 &
  0.11756 &
  0.16466 &
  0.17865 &
  0.1883 &
  0.18836 \\
\textbf{SR} &
  0.04213 &
  0.09349 &
  0.12579 &
  0.18443 &
  0.24126 &
  0.04213 &
  0.06397 &
  0.07129 &
  0.07916 &
  0.08314 \\
\textbf{VSKNN} &
  0.08734 & 0.17051 & 0.20827 & 0.26180 & 0.30811 & 0.08734 & 0.12380 & 0.13191 & 0.13913 & 0.14189 \\
\textbf{SMF} &
  0.06566 &
  0.20381 &
  0.29315 &
  0.43566 &
  0.56815 &
  0.06566 &
  0.12382 &
  0.14412 &
  0.1631 &
  0.17237 \\
\textbf{Item2Vec} &
  0.0847 &
  0.16657 &
  0.21624 &
  0.2965 &
  0.38568 &
  0.0847 &
  0.12015 &
  0.13141 &
  0.14205 &
  0.14817 \\
\textbf{GRU4Rec+} &
  0.08952 &
  0.20018 &
  0.28003 &
  0.40954 &
  0.54153 &
  0.08952 &
  0.13643 &
  0.15457 &
  0.17184 &
  0.18107 \\
\textbf{NARM} &
  0.11983 &
  0.27936 &
  0.3797 &
  0.5217 &
  0.70695 &
  0.11983 &
  0.18611 &
  0.20724 &
  0.22832 &
  0.23934 \\
\textbf{STAMP} &
  0.13336 &
  0.27264 &
  0.35459 &
  0.48032 &
  0.60696 &
  0.13336 &
  0.19339 &
  0.21206 &
  0.22891 &
  0.23778 \\
\textbf{NextItNet} &
  0.18071 &
  0.3442 &
  0.42323 &
  0.52906 &
  0.6247 &
  0.18071 &
  0.2512 &
  0.26929 &
  0.28341 &
  0.29012 \\
\textbf{SRGNN} &
  0.14191 &
  0.28852 &
  0.37334 &
  0.49911 &
  0.61951 &
  0.14191 &
  0.20517 &
  0.22445 &
  0.24118 &
  0.24958 \\
\textbf{CSRM} &
  0.16867 &
  0.32838 &
  0.41316 &
  0.54922 &
  0.67667 &
  0.16867 &
  0.23756 &
  0.25684 &
  0.27494 &
  0.28388 \\ \hline
\cellcolor[HTML]{333333}{\color[HTML]{FFFFFF} } &
  \multicolumn{5}{c|}{\textbf{HR@}} &
  \multicolumn{5}{c|}{\textbf{MRR@}} \\ \cline{2-11} 
\multirow{-2}{*}{\cellcolor[HTML]{333333}{\color[HTML]{FFFFFF} \textbf{CIKMCUP}}} &
  \textbf{1} &
  \textbf{3} &
  \textbf{5} &
  \textbf{10} &
  \textbf{20} &
  \textbf{1} &
  \textbf{3} &
  \textbf{5} &
  \textbf{10} &
  \textbf{20} \\ \hline
\textbf{S-POP} &
  0.03958 &
  0.10163 &
  0.11996 &
  0.13162 &
  0.1366 &
  0.03958 &
  0.06676 &
  0.071 &
  0.07267 &
  0.07302 \\
\textbf{AR} &
  0.04638 &
  0.10272 &
  0.144 &
  0.20131 &
  0.20155 &
  0.04638 &
  0.07014 &
  0.07949 &
  0.08745 &
  0.08747 \\
\textbf{SR} &
  0.0475 &
  0.10586 &
  0.14264 &
  0.20992 &
  0.27246 &
  0.0475 &
  0.07232 &
  0.08067 &
  0.08965 &
  0.09401 \\
\textbf{VSKNN} &
  0.05065 & 0.09875 & 0.12945 & 0.17178 & 0.21390 & 0.05065 & 0.07145 & 0.07838 & 0.08404 & 0.08698 \\
\textbf{SMF} &
  0.03443 &
  0.09768 &
  0.14701 &
  0.23846 &
  0.35299 &
  0.03443 &
  0.06123 &
  0.07247 &
  0.08471 &
  0.09254 \\
\textbf{Item2Vec} &
  0.01971 &
  0.04676 &
  0.0628 &
  0.09646 &
  0.15473 &
  0.01971 &
  0.0313 &
  0.03486 &
  0.03931 &
  0.04326 \\
\textbf{GRU4Rec+} &
  0.02723 &
  0.06813 &
  0.10225 &
  0.16953 &
  0.25702 &
  0.02723 &
  0.04433 &
  0.05204 &
  0.0609 &
  0.06687 \\
\textbf{NARM} &
  0.03642 &
  0.10692 &
  0.16702 &
  0.2591 &
  0.45553 &
  0.03642 &
  0.06606 &
  0.07969 &
  0.0917 &
  0.10304 \\
\textbf{STAMP} &
  0.03764 &
  0.09957 &
  0.14463 &
  0.22538 &
  0.3343 &
  0.03764 &
  0.06387 &
  0.07407 &
  0.08466 &
  0.09215 \\
\textbf{NextItNet} &
  0.03079 &
  0.06388 &
  0.09053 &
  0.13419 &
  0.19853 &
  0.03079 &
  0.0445 &
  0.05038 &
  0.05621 &
  0.06068 \\
\textbf{SRGNN} &
  0.05012 &
  0.12031 &
  0.17404 &
  0.26707 &
  0.37981 &
  0.05012 &
  0.07957 &
  0.09169 &
  0.10414 &
  0.11194 \\
\textbf{CSRM} &
  0.03919 &
  0.10503 &
  0.15882 &
  0.25788 &
  0.37739 &
  0.03919 &
  0.06675 &
  0.079 &
  0.09197 &
  0.10016 \\ \hline
\cellcolor[HTML]{333333}{\color[HTML]{FFFFFF} } &
  \multicolumn{5}{c|}{\textbf{HR@}} &
  \multicolumn{5}{c|}{\textbf{MRR@}} \\ \cline{2-11} 
\multirow{-2}{*}{\cellcolor[HTML]{333333}{\color[HTML]{FFFFFF} \textbf{TMALL}}} &
  \textbf{1} &
  \textbf{3} &
  \textbf{5} &
  \textbf{10} &
  \textbf{20} &
  \textbf{1} &
  \textbf{3} &
  \textbf{5} &
  \textbf{10} &
  \textbf{20} \\ \hline
\textbf{S-POP} &
  0.04434 &
  0.10295 &
  0.1304 &
  0.1627 &
  0.18396 &
  0.04434 &
  0.06969 &
  0.07596 &
  0.08036 &
  0.08189 \\
\textbf{AR} &
  0.01533 &
  0.03149 &
  0.04229 &
  0.05675 &
  0.05713 &
  0.01533 &
  0.02225 &
  0.02469 &
  0.02671 &
  0.02673 \\
\textbf{SR} &
  0.01514 &
  0.03106 &
  0.04078 &
  0.05555 &
  0.07272 &
  0.01514 &
  0.022 &
  0.02421 &
  0.02618 &
  0.02737 \\
\textbf{VSKNN} &
  0.02512 & 0.03891 & 0.04485 & 0.05749 & 0.06797 & 0.02512 & 0.03074 & 0.03210 & 0.03438 & 0.03499 \\
\textbf{SMF} &
  0.01704 &
  0.05033 &
  0.06319 &
  0.09471 &
  0.12743 &
  0.01704 &
  0.0229 &
  0.03583 &
  0.03603 &
  0.03954 \\
\textbf{Item2Vec} &
  0.0023 &
  0.00507 &
  0.00734 &
  0.0119 &
  0.01849 &
  0.0023 &
  0.00347 &
  0.00398 &
  0.00457 &
  0.00502 \\
\textbf{GRU4Rec+} &
  0.03101 &
  0.06645 &
  0.08865 &
  0.12219 &
  0.15954 &
  0.03101 &
  0.0463 &
  0.05135 &
  0.0558 &
  0.05838 \\
\textbf{NARM} &
  0.038 &
  0.09152 &
  0.12595 &
  0.16387 &
  0.25301 &
  0.038 &
  0.06145 &
  0.06961 &
  0.07449 &
  0.08008 \\
\textbf{STAMP} &
  0.03071 &
  0.06109 &
  0.08078 &
  0.11104 &
  0.14734 &
  0.03071 &
  0.04374 &
  0.0482 &
  0.05222 &
  0.05473 \\
\textbf{NextItNet} &
  0.02848 &
  0.05471 &
  0.06847 &
  0.09396 &
  0.11839 &
  0.02848 &
  0.03992 &
  0.04313 &
  0.04641 &
  0.04809 \\
\textbf{SRGNN} &
  0.04025 &
  0.07967 &
  0.10416 &
  0.14104 &
  0.18182 &
  0.04025 &
  0.05735 &
  0.06294 &
  0.06784 &
  0.07067 \\
\textbf{CSRM} &
  0.03715 &
  0.07736 &
  0.10183 &
  0.14033 &
  0.18497 &
  0.03715 &
  0.05447 &
  0.06006 &
  0.06516 &
  0.06824 \\ \hline
\cellcolor[HTML]{333333}{\color[HTML]{FFFFFF} } &
  \multicolumn{5}{c|}{\textbf{HR@}} &
  \multicolumn{5}{c|}{\textbf{MRR@}} \\ \cline{2-11} 
\multirow{-2}{*}{\cellcolor[HTML]{333333}{\color[HTML]{FFFFFF} \textbf{ROCKET}}} &
  \textbf{1} &
  \textbf{3} &
  \textbf{5} &
  \textbf{10} &
  \textbf{20} &
  \textbf{1} &
  \textbf{3} &
  \textbf{5} &
  \textbf{10} &
  \textbf{20} \\ \hline
\textbf{S-POP} &
  0.03955 &
  0.11389 &
  0.12938 &
  0.14248 &
  0.15225 &
  0.03955 &
  0.07263 &
  0.07623 &
  0.07795 &
  0.07866 \\
\textbf{AR} &
  0.05313 &
  0.1077 &
  0.13486 &
  0.16536 &
  0.16559 &
  0.05313 &
  0.07696 &
  0.08305 &
  0.08739 &
  0.0874 \\
\textbf{SR} &
  0.05075 &
  0.10102 &
  0.12294 &
  0.15058 &
  0.1706 &
  0.05075 &
  0.07231 &
  0.07736 &
  0.08111 &
  0.08256 \\
\textbf{VSKNN} &
  0.12109 & 0.19103 & 0.21187 & 0.24051 & 0.26339 & 0.12109 & 0.15188 & 0.15659 & 0.16046 & 0.16207 \\
\textbf{SMF} &
  0.0417 &
  0.10484 &
  0.15035 &
  0.20944 &
  0.27448 &
  0.0417 &
  0.06926 &
  0.07966 &
  0.08744 &
  0.0919 \\
\textbf{Item2Vec} &
  0.02292 &
  0.05169 &
  0.06584 &
  0.09583 &
  0.12753 &
  0.02292 &
  0.03584 &
  0.039 &
  0.04299 &
  0.0452 \\
\textbf{GRU4Rec+} &
  0.04282 &
  0.08682 &
  0.11632 &
  0.15747 &
  0.19981 &
  0.04282 &
  0.06157 &
  0.06836 &
  0.07382 &
  0.07676 \\
\textbf{NARM} &
  0.06051 &
  0.1328 &
  0.17737 &
  0.2357 &
  0.32289 &
  0.06051 &
  0.09174 &
  0.10207 &
  0.10985 &
  0.11513 \\
\textbf{STAMP} &
  0.04865 &
  0.10137 &
  0.13372 &
  0.17925 &
  0.22957 &
  0.04865 &
  0.07117 &
  0.07849 &
  0.08458 &
  0.08813 \\
\textbf{NextItNet} &
  0.04297 &
  0.07031 &
  0.09115 &
  0.11263 &
  0.13802 &
  0.04297 &
  0.0548 &
  0.05971 &
  0.06268 &
  0.06454 \\
\textbf{SRGNN} &
  0.05777 &
  0.12121 &
  0.16004 &
  0.20123 &
  0.24645 &
  0.05777 &
  0.08464 &
  0.09356 &
  0.09907 &
  0.10217 \\
\textbf{CSRM} &
  0.06665 &
  0.12666 &
  0.1703 &
  0.22509 &
  0.28344 &
  0.06665 &
  0.0927 &
  0.10271 &
  0.10999 &
  0.11407 \\ \hline
\end{tabular}}
\label{tab:timespan-30}
\end{table*}
