# Supplementary material for: Comprehensive Empirical Evaluation of Deep Learning Approaches for Session-based Recommendation in E-Commerce
Source: arXiv:2010.12540 source file (2020-10-17)
Supplement: Supplementary file 10 [file tab14.tex]

% Please add the following required packages to your document preamble:
% \usepackage{multirow}
% \usepackage[table,xcdraw]{xcolor}
% If you use beamer only pass "xcolor=table" option, i.e. \documentclass[xcolor=table]{beamer}
\begin{table*}[!h]
\centering
\caption{RQ5: training using random 1/8, 1/2, 1/8, 1/2 portions of the full training set for RECSYS, CIKMCUP, TMALL, ROCKET datasets respectively.}
\resizebox{0.9\textwidth}{!}{\begin{tabular}{|c|ccccc|ccccc|}
\hline
\cellcolor[HTML]{333333}{\color[HTML]{FFFFFF} } &
  \multicolumn{5}{c|}{\textbf{HR@}} &
  \multicolumn{5}{c|}{\textbf{MRR@}} \\ \cline{2-11} 
\multirow{-2}{*}{\cellcolor[HTML]{333333}{\color[HTML]{FFFFFF} \textbf{RECSYS}}} &
  \textbf{1} &
  \textbf{3} &
  \textbf{5} &
  \textbf{10} &
  \textbf{20} &
  \textbf{1} &
  \textbf{3} &
  \textbf{5} &
  \textbf{10} &
  \textbf{20} \\ \hline
\textbf{S-POP} &
  0.03582 &
  0.09813 &
  0.123 &
  0.14269 &
  0.15112 &
  0.03582 &
  0.06312 &
  0.06885 &
  0.07159 &
  0.07221 \\
\textbf{AR} &
  0.09641 &
  0.19159 &
  0.2539 &
  0.31463 &
  0.31472 &
  0.09641 &
  0.13741 &
  0.15159 &
  0.16022 &
  0.16022 \\
\textbf{SR} &
  0.10089 &
  0.1919 &
  0.25294 &
  0.33392 &
  0.41752 &
  0.10089 &
  0.14016 &
  0.15411 &
  0.1649 &
  0.17073 \\
\textbf{VSKNN} &
  0.06080 & 0.10004 & 0.11868 & 0.14825 & 0.18166 & 0.06080 & 0.07828 & 0.08256 & 0.08518 & 0.09676 \\
\textbf{SMF} &
  0.06719 &
  0.18664 &
  0.26748 &
  0.39281 &
  0.51018 &
  0.06719 &
  0.11789 &
  0.13632 &
  0.1531 &
  0.16131 \\
\textbf{Item2Vec} &
  0.05411 &
  0.10943 &
  0.14973 &
  0.21677 &
  0.30772 &
  0.05411 &
  0.07761 &
  0.08674 &
  0.09546 &
  0.10179 \\
\textbf{GRU4Rec+} &
  0.07695 &
  0.17757 &
  0.2516 &
  0.37679 &
  0.50812 &
  0.07695 &
  0.11968 &
  0.13645 &
  0.15309 &
  0.16222 \\
\textbf{NARM} &
  0.09475 &
  0.22753 &
  0.3239 &
  0.47069 &
  0.6611 &
  0.09475 &
  0.15178 &
  0.17375 &
  0.19343 &
  0.20506 \\
\textbf{STAMP} &
  0.10893 &
  0.23219 &
  0.30545 &
  0.41642 &
  0.53818 &
  0.10893 &
  0.1619 &
  0.17852 &
  0.19333 &
  0.20183 \\
\textbf{NextItNet} &
  0.16425 &
  0.30563 &
  0.38028 &
  0.48445 &
  0.5813 &
  0.16425 &
  0.22542 &
  0.24234 &
  0.25631 &
  0.26312 \\
\textbf{SRGNN} &
  0.12413 &
  0.25342 &
  0.32953 &
  0.44566 &
  0.56492 &
  0.12413 &
  0.17982 &
  0.19709 &
  0.21253 &
  0.22082 \\
\textbf{CSRM} &
  0.14415 &
  0.2902 &
  0.37905 &
  0.51586 &
  0.64403 &
  0.14415 &
  0.20671 &
  0.22692 &
  0.24506 &
  0.25402 \\ \hline
\cellcolor[HTML]{333333}{\color[HTML]{FFFFFF} } &
  \multicolumn{5}{c|}{\textbf{HR@}} &
  \multicolumn{5}{c|}{\textbf{MRR@}} \\ \cline{2-11} 
\multirow{-2}{*}{\cellcolor[HTML]{333333}{\color[HTML]{FFFFFF} \textbf{CIKMCUP}}} &
  \textbf{1} &
  \textbf{3} &
  \textbf{5} &
  \textbf{10} &
  \textbf{20} &
  \textbf{1} &
  \textbf{3} &
  \textbf{5} &
  \textbf{10} &
  \textbf{20} \\ \hline
\textbf{S-POP} &
  0.03873 &
  0.09847 &
  0.11678 &
  0.13016 &
  0.13509 &
  0.03873 &
  0.06502 &
  0.06926 &
  0.07115 &
  0.07147 \\
\textbf{AR} &
  0.04531 &
  0.09941 &
  0.13897 &
  0.19413 &
  0.19448 &
  0.04531 &
  0.06858 &
  0.07758 &
  0.08528 &
  0.08531 \\
\textbf{SR} &
  0.0412 &
  0.09178 &
  0.127 &
  0.18052 &
  0.23721 &
  0.0412 &
  0.06244 &
  0.07044 &
  0.07746 &
  0.08141 \\
\textbf{VSKNN} &
  0.05080 & 0.09945 & 0.12383 & 0.15723 & 0.19300 & 0.05080 & 0.07181 & 0.07731 & 0.08182 & 0.08434 \\
\textbf{SMF} &
  0.03913 &
  0.09853 &
  0.14284 &
  0.22345 &
  0.33412 &
  0.03913 &
  0.064 &
  0.07414 &
  0.08472 &
  0.09235 \\
\textbf{Item2Vec} &
  0.01384 &
  0.03241 &
  0.04802 &
  0.07689 &
  0.12243 &
  0.01384 &
  0.0218 &
  0.02534 &
  0.02916 &
  0.03225 \\
\textbf{GRU4Rec+} &
  0.02868 &
  0.07175 &
  0.10874 &
  0.17149 &
  0.26326 &
  0.02868 &
  0.04694 &
  0.05526 &
  0.06355 &
  0.0698 \\
\textbf{NARM} &
  0.04576 &
  0.11402 &
  0.16323 &
  0.26194 &
  0.40417 &
  0.04576 &
  0.07474 &
  0.08598 &
  0.09894 &
  0.10949 \\
\textbf{STAMP} &
  0.0385 &
  0.09367 &
  0.13441 &
  0.21376 &
  0.30896 &
  0.0385 &
  0.06194 &
  0.07124 &
  0.08172 &
  0.08828 \\
\textbf{NextItNet} &
  0.03125 &
  0.07858 &
  0.10202 &
  0.15579 &
  0.22748 &
  0.03125 &
  0.05124 &
  0.05662 &
  0.06373 &
  0.06868 \\
\textbf{SRGNN} &
  0.04594 &
  0.10961 &
  0.15672 &
  0.24079 &
  0.34993 &
  0.04594 &
  0.07317 &
  0.08382 &
  0.09498 &
  0.10256 \\
\textbf{CSRM} &
  0.04382 &
  0.10789 &
  0.15689 &
  0.24841 &
  0.36867 &
  0.04382 &
  0.07077 &
  0.08181 &
  0.09384 &
  0.10215 \\ \hline
\cellcolor[HTML]{333333}{\color[HTML]{FFFFFF} } &
  \multicolumn{5}{c|}{\textbf{HR@}} &
  \multicolumn{5}{c|}{\textbf{MRR@}} \\ \cline{2-11} 
\multirow{-2}{*}{\cellcolor[HTML]{333333}{\color[HTML]{FFFFFF} \textbf{TMALL}}} &
  \textbf{1} &
  \textbf{3} &
  \textbf{5} &
  \textbf{10} &
  \textbf{20} &
  \textbf{1} &
  \textbf{3} &
  \textbf{5} &
  \textbf{10} &
  \textbf{20} \\ \hline
\textbf{S-POP} &
  0.04681 &
  0.1092 &
  0.13858 &
  0.17092 &
  0.19057 &
  0.04681 &
  0.04681 &
  0.04681 &
  0.04681 &
  0.04681 \\
\textbf{AR} &
  0.01108 &
  0.02335 &
  0.03168 &
  0.04302 &
  0.04321 &
  0.01108 &
  0.01634 &
  0.01822 &
  0.01979 &
  0.0198 \\
\textbf{SR} &
  0.01052 &
  0.02163 &
  0.02863 &
  0.03919 &
  0.05029 &
  0.01052 &
  0.01528 &
  0.01686 &
  0.01826 &
  0.01902 \\
\textbf{VSKNN} &
  0.02664 & 0.04336 & 0.05019 & 0.06198 & 0.07408 & 0.02664 & 0.03403 & 0.03527 & 0.03770 & 0.03782 \\
\textbf{SMF} &
  0.01233 &
  0.03175 &
  0.0454 &
  0.06768 &
  0.09429 &
  0.01233 &
  0.02061 &
  0.02371 &
  0.02666 &
  0.02847 \\
\textbf{Item2Vec} &
  0.00168 &
  0.00428 &
  0.00613 &
  0.01015 &
  0.01681 &
  0.00168 &
  0.00278 &
  0.0032 &
  0.00373 &
  0.00418 \\
\textbf{GRU4Rec+} &
  0.0176 &
  0.04029 &
  0.05466 &
  0.07668 &
  0.0997 &
  0.0176 &
  0.02722 &
  0.03049 &
  0.0334 &
  0.03499 \\
\textbf{NARM} &
  0.02502 &
  0.05624 &
  0.07271 &
  0.10318 &
  0.13814 &
  0.02502 &
  0.0384 &
  0.04217 &
  0.04617 &
  0.04898 \\
\textbf{STAMP} &
  0.02199 &
  0.04927 &
  0.06511 &
  0.08955 &
  0.11524 &
  0.02199 &
  0.03363 &
  0.03723 &
  0.04047 &
  0.04225 \\
\textbf{NextItNet} &
  0.01128 &
  0.02279 &
  0.02978 &
  0.04208 &
  0.05212 &
  0.01128 &
  0.0161 &
  0.01769 &
  0.01932 &
  0.02 \\
\textbf{SRGNN} &
  0.03064 &
  0.05915 &
  0.07542 &
  0.10044 &
  0.12745 &
  0.03064 &
  0.04285 &
  0.04654 &
  0.04985 &
  0.05172 \\
\textbf{CSRM} &
  0.02102 &
  0.04584 &
  0.0609 &
  0.08462 &
  0.11239 &
  0.02102 &
  0.03168 &
  0.03511 &
  0.03826 &
  0.04018 \\ \hline
\cellcolor[HTML]{333333}{\color[HTML]{FFFFFF} } &
  \multicolumn{5}{c|}{\textbf{HR@}} &
  \multicolumn{5}{c|}{\textbf{MRR@}} \\ \cline{2-11} 
\multirow{-2}{*}{\cellcolor[HTML]{333333}{\color[HTML]{FFFFFF} \textbf{ROCKET}}} &
  \textbf{1} &
  \textbf{3} &
  \textbf{5} &
  \textbf{10} &
  \textbf{20} &
  \textbf{1} &
  \textbf{3} &
  \textbf{5} &
  \textbf{10} &
  \textbf{20} \\ \hline
\textbf{S-POP} &
  0.04175 &
  0.11118 &
  0.12635 &
  0.13975 &
  0.14832 &
  0.04175 &
  0.07376 &
  0.07727 &
  0.07907 &
  0.07969 \\
\textbf{AR} &
  0.05296 &
  0.1002 &
  0.12744 &
  0.1626 &
  0.16326 &
  0.05296 &
  0.07321 &
  0.07956 &
  0.08446 &
  0.0845 \\
\textbf{SR} &
  0.04746 &
  0.09778 &
  0.11887 &
  0.15205 &
  0.18062 &
  0.04746 &
  0.06962 &
  0.07449 &
  0.07897 &
  0.08101 \\
\textbf{VSKNN} &
  0.11022 & 0.17396 & 0.19361 & 0.21275 & 0.22949 & 0.11022 & 0.13873 & 0.14324 & 0.14583 & 0.14698 \\
\textbf{SMF} &
  0.04109 &
  0.10525 &
  0.1503 &
  0.21819 &
  0.28785 &
  0.04109 &
  0.06845 &
  0.07871 &
  0.0877 &
  0.09252 \\
\textbf{Item2Vec} &
  0.01586 &
  0.03776 &
  0.05295 &
  0.07752 &
  0.11104 &
  0.01586 &
  0.02536 &
  0.0288 &
  0.03201 &
  0.03428 \\
\textbf{GRU4Rec+} &
  0.04275 &
  0.0877 &
  0.12649 &
  0.17915 &
  0.23491 &
  0.04275 &
  0.06211 &
  0.07074 &
  0.07769 &
  0.08158 \\
\textbf{NARM} &
  0.06045 &
  0.14172 &
  0.19803 &
  0.26383 &
  0.36641 &
  0.06045 &
  0.09539 &
  0.10834 &
  0.11731 &
  0.12341 \\
\textbf{STAMP} &
  0.04618 &
  0.09943 &
  0.13456 &
  0.19156 &
  0.2468 &
  0.04618 &
  0.06919 &
  0.07717 &
  0.08467 &
  0.08841 \\
\textbf{NextItNet} &
  0.06899 &
  0.12382 &
  0.14328 &
  0.18868 &
  0.22642 &
  0.06899 &
  0.09296 &
  0.09742 &
  0.10371 &
  0.10638 \\
\textbf{SRGNN} &
  0.07487 &
  0.14062 &
  0.18273 &
  0.23676 &
  0.29036 &
  0.07487 &
  0.10341 &
  0.11294 &
  0.12008 &
  0.12378 \\
\textbf{CSRM} &
  0.07669 &
  0.15403 &
  0.19991 &
  0.26742 &
  0.33734 &
  0.07669 &
  0.10975 &
  0.1202 &
  0.12928 &
  0.13403 \\ \hline
\end{tabular}}
\label{tab:size-large}
\end{table*}
