# Supplementary material for: Comprehensive Empirical Evaluation of Deep Learning Approaches for Session-based Recommendation in E-Commerce
Source: arXiv:2010.12540 source file (2020-10-17)
Supplement: Supplementary file 11 [file tab15.tex]

% Please add the following required packages to your document preamble:
% \usepackage{multirow}
% \usepackage[table,xcdraw]{xcolor}
% If you use beamer only pass "xcolor=table" option, i.e. \documentclass[xcolor=table]{beamer}
\begin{table*}[!h]
\centering
\caption{RQ5: training using random 1/16, 1/8, 1/16, 1/8 portions of the full training set for RECSYS, CIKMCUP, TMALL, ROCKET datasets respectively.}
\resizebox{0.9\textwidth}{!}{\begin{tabular}{|c|ccccc|ccccc|}
\hline
\cellcolor[HTML]{333333}{\color[HTML]{FFFFFF} } &
  \multicolumn{5}{c|}{\textbf{HR@}} &
  \multicolumn{5}{c|}{\textbf{MRR@}} \\ \cline{2-11} 
\multirow{-2}{*}{\cellcolor[HTML]{333333}{\color[HTML]{FFFFFF} \textbf{RECSYS}}} &
  \textbf{1} &
  \textbf{3} &
  \textbf{5} &
  \textbf{10} &
  \textbf{20} &
  \textbf{1} &
  \textbf{3} &
  \textbf{5} &
  \textbf{10} &
  \textbf{20} \\ \hline
\textbf{S-POP} &
  0.12986 &
  0.21113 &
  0.23887 &
  0.25946 &
  0.26744 &
  0.12986 &
  0.1659 &
  0.17229 &
  0.17518 &
  0.17577 \\
\textbf{AR} &
  0.07738 &
  0.15404 &
  0.20174 &
  0.25593 &
  0.25641 &
  0.07738 &
  0.11089 &
  0.12179 &
  0.12935 &
  0.12938 \\
\textbf{SR} &
  0.09684 &
  0.18548 &
  0.23781 &
  0.30971 &
  0.38576 &
  0.09684 &
  0.13505 &
  0.14695 &
  0.15661 &
  0.16186 \\
\textbf{VSKNN} &
  0.08387 & 0.14548 & 0.18405 & 0.23012 & 0.28761 & 0.08387 & 0.11094 & 0.11959 & 0.12575 & 0.12962 \\
\textbf{SMF} &
  0.06524 &
  0.17399 &
  0.25059 &
  0.36415 &
  0.48033 &
  0.06524 &
  0.11162 &
  0.12911 &
  0.14428 &
  0.15239 \\
\textbf{Item2Vec} &
  0.04703 &
  0.09883 &
  0.13127 &
  0.19867 &
  0.28418 &
  0.04703 &
  0.0695 &
  0.07685 &
  0.08561 &
  0.09154 \\
\textbf{GRU4Rec+} &
  0.07526 &
  0.16944 &
  0.23867 &
  0.3545 &
  0.47698 &
  0.07526 &
  0.11525 &
  0.13098 &
  0.14635 &
  0.15489 \\
\textbf{NARM} &
  0.09725 &
  0.2191 &
  0.30572 &
  0.43926 &
  0.6317 &
  0.09725 &
  0.1498 &
  0.16939 &
  0.18731 &
  0.19892 \\
\textbf{STAMP} &
  0.10244 &
  0.21142 &
  0.28161 &
  0.38967 &
  0.50613 &
  0.10244 &
  0.14941 &
  0.16534 &
  0.17974 &
  0.18781 \\
\textbf{NextItNet} &
  0.15686 &
  0.28851 &
  0.35782 &
  0.45975 &
  0.55857 &
  0.15686 &
  0.21334 &
  0.22923 &
  0.24285 &
  0.24973 \\
\textbf{SRGNN} &
  0.11629 &
  0.2394 &
  0.31111 &
  0.42231 &
  0.53981 &
  0.11629 &
  0.16958 &
  0.18589 &
  0.2007 &
  0.20882 \\
\textbf{CSRM} &
  0.1403 &
  0.27246 &
  0.3521 &
  0.47999 &
  0.60582 &
  0.1403 &
  0.19663 &
  0.21471 &
  0.23169 &
  0.24048 \\ \hline
\cellcolor[HTML]{333333}{\color[HTML]{FFFFFF} } &
  \multicolumn{5}{c|}{\textbf{HR@}} &
  \multicolumn{5}{c|}{\textbf{MRR@}} \\ \cline{2-11} 
\multirow{-2}{*}{\cellcolor[HTML]{333333}{\color[HTML]{FFFFFF} \textbf{CIKMCUP}}} &
  \textbf{1} &
  \textbf{3} &
  \textbf{5} &
  \textbf{10} &
  \textbf{20} &
  \textbf{1} &
  \textbf{3} &
  \textbf{5} &
  \textbf{10} &
  \textbf{20} \\ \hline
\textbf{S-POP} &
  0.04024 &
  0.10131 &
  0.12099 &
  0.13493 &
  0.14039 &
  0.04024 &
  0.0667 &
  0.07126 &
  0.07322 &
  0.07359 \\
\textbf{AR} &
  0.03319 &
  0.08047 &
  0.11553 &
  0.15649 &
  0.15706 &
  0.03319 &
  0.0537 &
  0.0616 &
  0.06725 &
  0.06729 \\
\textbf{SR} &
  0.03075 &
  0.06998 &
  0.0957 &
  0.13335 &
  0.16842 &
  0.03075 &
  0.04773 &
  0.0536 &
  0.05858 &
  0.06104 \\
\textbf{VSKNN} &
  0.05956 & 0.11756 & 0.14896 & 0.19229 & 0.23239 & 0.05956 & 0.08464 & 0.09177 & 0.09750 & 0.10029 \\
\textbf{SMF} &
  0.0342 &
  0.08272 &
  0.11634 &
  0.19556 &
  0.291 &
  0.0342 &
  0.05461 &
  0.0622 &
  0.07273 &
  0.07931 \\
\textbf{Item2Vec} &
  0.01836 &
  0.04082 &
  0.05903 &
  0.09618 &
  0.1511 &
  0.01836 &
  0.0278 &
  0.03192 &
  0.03678 &
  0.04051 \\
\textbf{GRU4Rec+} &
  0.02074 &
  0.04987 &
  0.07274 &
  0.11095 &
  0.16323 &
  0.02074 &
  0.03301 &
  0.03821 &
  0.04334 &
  0.04695 \\
\textbf{NARM} &
  0.02831 &
  0.07686 &
  0.11283 &
  0.1868 &
  0.33921 &
  0.02831 &
  0.04931 &
  0.05754 &
  0.06724 &
  0.07602 \\
\textbf{STAMP} &
  0.02271 &
  0.0572 &
  0.08896 &
  0.14027 &
  0.21328 &
  0.02271 &
  0.03696 &
  0.04413 &
  0.05086 &
  0.05586 \\
\textbf{NextItNet} &
  0.01058 &
  0.02268 &
  0.03427 &
  0.05595 &
  0.08065 &
  0.01058 &
  0.01579 &
  0.01839 &
  0.02114 &
  0.02278 \\
\textbf{SRGNN} &
  0.03523 &
  0.09034 &
  0.13125 &
  0.20327 &
  0.29119 &
  0.03523 &
  0.05814 &
  0.06738 &
  0.077 &
  0.0831 \\
\textbf{CSRM} &
  0.03142 &
  0.07971 &
  0.11646 &
  0.18291 &
  0.26967 &
  0.03142 &
  0.05184 &
  0.06025 &
  0.06895 &
  0.07491 \\ \hline
\cellcolor[HTML]{333333}{\color[HTML]{FFFFFF} } &
  \multicolumn{5}{c|}{\textbf{HR@}} &
  \multicolumn{5}{c|}{\textbf{MRR@}} \\ \cline{2-11} 
\multirow{-2}{*}{\cellcolor[HTML]{333333}{\color[HTML]{FFFFFF} \textbf{TMALL}}} &
  \textbf{1} &
  \textbf{3} &
  \textbf{5} &
  \textbf{10} &
  \textbf{20} &
  \textbf{1} &
  \textbf{3} &
  \textbf{5} &
  \textbf{10} &
  \textbf{20} \\ \hline
\textbf{S-POP} &
  0.04815 &
  0.11308 &
  0.14347 &
  0.17564 &
  0.19308 &
  0.04815 &
  0.04815 &
  0.04815 &
  0.04815 &
  0.04815 \\
\textbf{AR} &
  0.01039 &
  0.02176 &
  0.02975 &
  0.04059 &
  0.04064 &
  0.01039 &
  0.01524 &
  0.01706 &
  0.01854 &
  0.01855 \\
\textbf{SR} &
  0.00983 &
  0.01939 &
  0.02522 &
  0.03486 &
  0.04385 &
  0.00983 &
  0.01391 &
  0.01524 &
  0.01653 &
  0.01716 \\
\textbf{VSKNN} &
  0.03073 & 0.04769 & 0.05684 & 0.07158 & 0.08502 & 0.03073 & 0.03776 & 0.03948 & 0.04292 & 0.04306 \\
\textbf{SMF} &
  0.01322 &
  0.03258 &
  0.04575 &
  0.06853 &
  0.09756 &
  0.01322 &
  0.02149 &
  0.02446 &
  0.02747 &
  0.02945 \\
\textbf{Item2Vec} &
  0.00234 &
  0.0053 &
  0.00772 &
  0.01275 &
  0.01909 &
  0.00234 &
  0.00361 &
  0.00417 &
  0.00482 &
  0.00525 \\
\textbf{GRU4Rec+} &
  0.01421 &
  0.03257 &
  0.04454 &
  0.06189 &
  0.07763 &
  0.01421 &
  0.022 &
  0.02472 &
  0.02703 &
  0.02813 \\
\textbf{NARM} &
  0.01707 &
  0.04165 &
  0.05639 &
  0.08374 &
  0.13195 &
  0.01707 &
  0.02788 &
  0.03128 &
  0.03499 &
  0.03805 \\
\textbf{STAMP} &
  0.02826 &
  0.05622 &
  0.07118 &
  0.09256 &
  0.11514 &
  0.02826 &
  0.04044 &
  0.04386 &
  0.0467 &
  0.04826 \\
\textbf{NextItNet} &
  0.0055 &
  0.01299 &
  0.01732 &
  0.02189 &
  0.02926 &
  0.0055 &
  0.00866 &
  0.00964 &
  0.01024 &
  0.01074 \\
\textbf{SRGNN} &
  0.02639 &
  0.05019 &
  0.06309 &
  0.0825 &
  0.10492 &
  0.02639 &
  0.03673 &
  0.03966 &
  0.04225 &
  0.04379 \\
\textbf{CSRM} &
  0.01637 &
  0.03432 &
  0.04509 &
  0.06196 &
  0.08155 &
  0.01637 &
  0.02408 &
  0.02653 &
  0.02876 &
  0.03011 \\ \hline
\cellcolor[HTML]{333333}{\color[HTML]{FFFFFF} } &
  \multicolumn{5}{c|}{\textbf{HR@}} &
  \multicolumn{5}{c|}{\textbf{MRR@}} \\ \cline{2-11} 
\multirow{-2}{*}{\cellcolor[HTML]{333333}{\color[HTML]{FFFFFF} \textbf{ROCKET}}} &
  \textbf{1} &
  \textbf{3} &
  \textbf{5} &
  \textbf{10} &
  \textbf{20} &
  \textbf{1} &
  \textbf{3} &
  \textbf{5} &
  \textbf{10} &
  \textbf{20} \\ \hline
\textbf{S-POP} &
  0.04497 &
  0.11588 &
  0.12828 &
  0.14154 &
  0.15221 &
  0.04497 &
  0.07774 &
  0.08062 &
  0.08238 &
  0.08313 \\
\textbf{AR} &
  0.05045 &
  0.09052 &
  0.11242 &
  0.13289 &
  0.13289 &
  0.05045 &
  0.06798 &
  0.07291 &
  0.07575 &
  0.07575 \\
\textbf{SR} &
  0.03575 &
  0.06976 &
  0.0885 &
  0.10781 &
  0.12367 &
  0.03575 &
  0.0504 &
  0.05475 &
  0.05744 &
  0.05858 \\
\textbf{VSKNN} &
  0.14355 & 0.22521 & 0.24895 & 0.27712 & 0.29621 & 0.14355 & 0.18005 & 0.18544 & 0.18913 & 0.19048 \\
\textbf{SMF} &
  0.03459 &
  0.08821 &
  0.1205 &
  0.17325 &
  0.21678 &
  0.03459 &
  0.05751 &
  0.06489 &
  0.072 &
  0.07505 \\
\textbf{Item2Vec} &
  0.01352 &
  0.03086 &
  0.04703 &
  0.06614 &
  0.09142 &
  0.01352 &
  0.02092 &
  0.0247 &
  0.02726 &
  0.02896 \\
\textbf{GRU4Rec+} &
  0.02917 &
  0.0652 &
  0.08693 &
  0.11124 &
  0.13697 &
  0.02917 &
  0.04466 &
  0.04966 &
  0.0529 &
  0.05463 \\
\textbf{NARM} &
  0.07116 &
  0.12208 &
  0.14715 &
  0.20231 &
  0.25761 &
  0.07116 &
  0.09361 &
  0.0993 &
  0.10652 &
  0.10963 \\
\textbf{STAMP} &
  0.03475 &
  0.07298 &
  0.09238 &
  0.12598 &
  0.16421 &
  0.03475 &
  0.05126 &
  0.0556 &
  0.06016 &
  0.06275 \\
\textbf{NextItNet} &
  0.01711 &
  0.03571 &
  0.04464 &
  0.0558 &
  0.07143 &
  0.01711 &
  0.02517 &
  0.02718 &
  0.02871 &
  0.02969 \\
\textbf{SRGNN} &
  0.04576 &
  0.0865 &
  0.10603 &
  0.13142 &
  0.15792 &
  0.04576 &
  0.06273 &
  0.06721 &
  0.07054 &
  0.07237 \\
\textbf{CSRM} &
  0.05695 &
  0.10876 &
  0.13938 &
  0.18832 &
  0.22896 &
  0.05695 &
  0.07899 &
  0.08582 &
  0.09221 &
  0.09497 \\ \hline
\end{tabular}}
\label{tab:size-medium}
\end{table*}
