# Supplementary material for: Comprehensive Empirical Evaluation of Deep Learning Approaches for Session-based Recommendation in E-Commerce
Source: arXiv:2010.12540 source file (2020-10-17)
Supplement: Supplementary file 12 [file tab16.tex]

% Please add the following required packages to your document preamble:
% \usepackage{multirow}
% \usepackage[table,xcdraw]{xcolor}
% If you use beamer only pass "xcolor=table" option, i.e. \documentclass[xcolor=table]{beamer}
\begin{table*}[!h]
\centering
\caption{RQ5: training using random 1/64, 1/16, 1/64, 1/16 portions of the full training set for RECSYS, CIKMCUP, TMALL, ROCKET datasets respectively.}
\resizebox{0.9\textwidth}{!}{\begin{tabular}{|c|ccccc|ccccc|}
\hline
\cellcolor[HTML]{333333}{\color[HTML]{FFFFFF} } &
  \multicolumn{5}{c|}{\textbf{HR@}} &
  \multicolumn{5}{c|}{\textbf{MRR@}} \\ \cline{2-11} 
\multirow{-2}{*}{\cellcolor[HTML]{333333}{\color[HTML]{FFFFFF} \textbf{RECSYS}}} &
  \textbf{1} &
  \textbf{3} &
  \textbf{5} &
  \textbf{10} &
  \textbf{20} &
  \textbf{1} &
  \textbf{3} &
  \textbf{5} &
  \textbf{10} &
  \textbf{20} \\ \hline
\textbf{S-POP} &
  0.03608 &
  0.09813 &
  0.12375 &
  0.14404 &
  0.15225 &
  0.03608 &
  0.06319 &
  0.06909 &
  0.07191 &
  0.07251 \\
\textbf{AR} &
  0.06248 &
  0.12136 &
  0.15408 &
  0.2001 &
  0.20054 &
  0.06248 &
  0.08831 &
  0.09584 &
  0.10216 &
  0.10219 \\
\textbf{SR} &
  0.07653 &
  0.15096 &
  0.19775 &
  0.2552 &
  0.31408 &
  0.07653 &
  0.10874 &
  0.11946 &
  0.12719 &
  0.13135 \\
\textbf{VSKNN} &
  0.07295 & 0.13216 & 0.15433 & 0.18276 & 0.20241 & 0.07295 & 0.09876 & 0.10386 & 0.10774 & 0.10911 \\
\textbf{SMF} &
  0.05043 &
  0.13755 &
  0.1912 &
  0.26832 &
  0.3603 &
  0.05043 &
  0.08771 &
  0.09989 &
  0.11014 &
  0.11652 \\
\textbf{Item2Vec} &
  0.03715 &
  0.0827 &
  0.12048 &
  0.19485 &
  0.28513 &
  0.03715 &
  0.05624 &
  0.06474 &
  0.07462 &
  0.08089 \\
\textbf{GRU4Rec+} &
  0.05889 &
  0.13143 &
  0.18468 &
  0.28116 &
  0.39492 &
  0.05889 &
  0.08984 &
  0.1019 &
  0.11469 &
  0.12255 \\
\textbf{NARM} &
  0.10208 &
  0.20746 &
  0.2733 &
  0.38933 &
  0.56824 &
  0.10208 &
  0.14956 &
  0.16586 &
  0.1813 &
  0.1919 \\
\textbf{STAMP} &
  0.08157 &
  0.16428 &
  0.21915 &
  0.31514 &
  0.42291 &
  0.08157 &
  0.1169 &
  0.12933 &
  0.14206 &
  0.14953 \\
\textbf{NextItNet} &
  0.10322 &
  0.19201 &
  0.25321 &
  0.34322 &
  0.43078 &
  0.10322 &
  0.1414 &
  0.15534 &
  0.16735 &
  0.17345 \\
\textbf{SRGNN} &
  0.08626 &
  0.18614 &
  0.2493 &
  0.34921 &
  0.4534 &
  0.08626 &
  0.12894 &
  0.14318 &
  0.15646 &
  0.16369 \\
\textbf{CSRM} &
  0.11145 &
  0.2286 &
  0.29914 &
  0.41273 &
  0.52951 &
  0.11145 &
  0.16185 &
  0.17787 &
  0.19304 &
  0.20116 \\ \hline
\cellcolor[HTML]{333333}{\color[HTML]{FFFFFF} } &
  \multicolumn{5}{c|}{\textbf{HR@}} &
  \multicolumn{5}{c|}{\textbf{MRR@}} \\ \cline{2-11} 
\multirow{-2}{*}{\cellcolor[HTML]{333333}{\color[HTML]{FFFFFF} \textbf{CIKMCUP}}} &
  \textbf{1} &
  \textbf{3} &
  \textbf{5} &
  \textbf{10} &
  \textbf{20} &
  \textbf{1} &
  \textbf{3} &
  \textbf{5} &
  \textbf{10} &
  \textbf{20} \\ \hline
\textbf{S-POP} &
  0.04096 &
  0.10371 &
  0.12219 &
  0.13579 &
  0.14084 &
  0.04096 &
  0.06871 &
  0.07293 &
  0.07484 &
  0.0752 \\
\textbf{AR} &
  0.03312 &
  0.07739 &
  0.10946 &
  0.14677 &
  0.14712 &
  0.03312 &
  0.05215 &
  0.05932 &
  0.06461 &
  0.06463 \\
\textbf{SR} &
  0.02876 &
  0.06484 &
  0.08297 &
  0.11853 &
  0.14189 &
  0.02876 &
  0.04439 &
  0.04847 &
  0.05318 &
  0.05486 \\
\textbf{VSKNN} &
  0.06980 & 0.13555 & 0.17333 & 0.22338 & 0.27157 & 0.06980 & 0.09876 & 0.10744 & 0.11405 & 0.11744 \\
\textbf{SMF} &
  0.03123 &
  0.07817 &
  0.11797 &
  0.19026 &
  0.28895 &
  0.03123 &
  0.05093 &
  0.05994 &
  0.06944 &
  0.07631 \\
\textbf{Item2Vec} &
  0.01601 &
  0.04209 &
  0.06116 &
  0.0966 &
  0.15075 &
  0.01601 &
  0.02722 &
  0.03153 &
  0.03623 &
  0.03991 \\
\textbf{GRU4Rec+} &
  0.01793 &
  0.0391 &
  0.05259 &
  0.07564 &
  0.10705 &
  0.01793 &
  0.02658 &
  0.0296 &
  0.0327 &
  0.03489 \\
\textbf{NARM} &
  0.03531 &
  0.07614 &
  0.11051 &
  0.16532 &
  0.28534 &
  0.03531 &
  0.05311 &
  0.0609 &
  0.06811 &
  0.07522 \\
\textbf{STAMP} &
  0.02354 &
  0.05021 &
  0.0727 &
  0.11349 &
  0.16335 &
  0.02354 &
  0.03527 &
  0.04041 &
  0.0456 &
  0.049 \\
\textbf{NextItNet} &
  0.00223 &
  0.00446 &
  0.00893 &
  0.01674 &
  0.02567 &
  0.00223 &
  0.00316 &
  0.00417 &
  0.00528 &
  0.00587 \\
\textbf{SRGNN} &
  0.03142 &
  0.08021 &
  0.11545 &
  0.17083 &
  0.22986 &
  0.03142 &
  0.05211 &
  0.06007 &
  0.06743 &
  0.07154 \\
\textbf{CSRM} &
  0.03531 &
  0.07692 &
  0.10927 &
  0.16346 &
  0.23217 &
  0.03531 &
  0.053 &
  0.0604 &
  0.06749 &
  0.07224 \\ \hline
\cellcolor[HTML]{333333}{\color[HTML]{FFFFFF} } &
  \multicolumn{5}{c|}{\textbf{HR@}} &
  \multicolumn{5}{c|}{\textbf{MRR@}} \\ \cline{2-11} 
\multirow{-2}{*}{\cellcolor[HTML]{333333}{\color[HTML]{FFFFFF} \textbf{TMALL}}} &
  \textbf{1} &
  \textbf{3} &
  \textbf{5} &
  \textbf{10} &
  \textbf{20} &
  \textbf{1} &
  \textbf{3} &
  \textbf{5} &
  \textbf{10} &
  \textbf{20} \\ \hline
\textbf{S-POP} &
  0.05564 &
  0.12872 &
  0.15952 &
  0.18701 &
  0.20051 &
  0.05564 &
  0.05564 &
  0.05564 &
  0.05564 &
  0.05564 \\
\textbf{AR} &
  0.00983 &
  0.02134 &
  0.02908 &
  0.03873 &
  0.03878 &
  0.00983 &
  0.01473 &
  0.01649 &
  0.01783 &
  0.01784 \\
\textbf{SR} &
  0.00821 &
  0.01734 &
  0.02274 &
  0.03082 &
  0.03684 &
  0.00821 &
  0.01217 &
  0.0134 &
  0.01449 &
  0.01492 \\
\textbf{VSKNN} &
  0.04325 & 0.06773 & 0.08435 & 0.10454 & 0.12633 & 0.04325 & 0.05389 & 0.05871 & 0.06169 & 0.06310 \\
\textbf{SMF} &
  0.0158 &
  0.03463 &
  0.04833 &
  0.07104 &
  0.09703 &
  0.0158 &
  0.02384 &
  0.02693 &
  0.02994 &
  0.03173 \\
\textbf{Item2Vec} &
  0.0032 &
  0.00717 &
  0.01009 &
  0.01576 &
  0.02275 &
  0.0032 &
  0.00491 &
  0.00557 &
  0.00632 &
  0.0068 \\
\textbf{GRU4Rec+} &
  0.00911 &
  0.01992 &
  0.02633 &
  0.03561 &
  0.04397 &
  0.00911 &
  0.01378 &
  0.01523 &
  0.01649 &
  0.01709 \\
\textbf{NARM} &
  0.01433 &
  0.03025 &
  0.04121 &
  0.05647 &
  0.08501 &
  0.01433 &
  0.02159 &
  0.0241 &
  0.02613 &
  0.02796 \\
\textbf{STAMP} &
  0.00963 &
  0.0209 &
  0.02788 &
  0.03903 &
  0.05114 &
  0.00963 &
  0.0144 &
  0.016 &
  0.01747 &
  0.0183 \\
\textbf{NextItNet} &
  0 &
  0.00041 &
  0.00137 &
  0.0037 &
  0.00781 &
  0 &
  0.00021 &
  0.00041 &
  0.00072 &
  0.00098 \\
\textbf{SRGNN} &
  0.02192 &
  0.03924 &
  0.04779 &
  0.06071 &
  0.07336 &
  0.02192 &
  0.02946 &
  0.03141 &
  0.03311 &
  0.03397 \\
\textbf{CSRM} &
  0.01072 &
  0.02194 &
  0.02679 &
  0.03472 &
  0.04298 &
  0.01072 &
  0.01562 &
  0.01672 &
  0.01775 &
  0.01832 \\ \hline
\cellcolor[HTML]{333333}{\color[HTML]{FFFFFF} } &
  \multicolumn{5}{c|}{\textbf{HR@}} &
  \multicolumn{5}{c|}{\textbf{MRR@}} \\ \cline{2-11} 
\multirow{-2}{*}{\cellcolor[HTML]{333333}{\color[HTML]{FFFFFF} \textbf{ROCKET}}} &
  \textbf{1} &
  \textbf{3} &
  \textbf{5} &
  \textbf{10} &
  \textbf{20} &
  \textbf{1} &
  \textbf{3} &
  \textbf{5} &
  \textbf{10} &
  \textbf{20} \\ \hline
\textbf{S-POP} &
  0.04467 &
  0.11974 &
  0.13363 &
  0.14227 &
  0.15278 &
  0.04467 &
  0.07927 &
  0.08246 &
  0.08371 &
  0.08435 \\
\textbf{AR} &
  0.0488 &
  0.08671 &
  0.10736 &
  0.1265 &
  0.128 &
  0.0488 &
  0.06494 &
  0.06982 &
  0.07245 &
  0.07253 \\
\textbf{SR} &
  0.03829 &
  0.0762 &
  0.08934 &
  0.10435 &
  0.11074 &
  0.03829 &
  0.05487 &
  0.05791 &
  0.05987 &
  0.06034 \\
\textbf{VSKNN} &
  0.16886 & 0.26844 & 0.30210 & 0.34053 & 0.36410 & 0.16886 & 0.21323 & 0.22099 & 0.22615 & 0.22780 \\
\textbf{SMF} &
  0.04017 &
  0.09009 &
  0.11787 &
  0.15728 &
  0.20233 &
  0.04017 &
  0.06169 &
  0.06786 &
  0.073 &
  0.07611 \\
\textbf{Item2Vec} &
  0.01272 &
  0.02967 &
  0.03815 &
  0.05434 &
  0.07938 &
  0.01272 &
  0.01985 &
  0.02175 &
  0.02379 &
  0.02549 \\
\textbf{GRU4Rec+} &
  0.02827 &
  0.0547 &
  0.07232 &
  0.08994 &
  0.1083 &
  0.02827 &
  0.03995 &
  0.04399 &
  0.04635 &
  0.04766 \\
\textbf{NARM} &
  0.05727 &
  0.1115 &
  0.13706 &
  0.1701 &
  0.23093 &
  0.05727 &
  0.07953 &
  0.08523 &
  0.08951 &
  0.09295 \\
\textbf{STAMP} &
  0.04832 &
  0.07739 &
  0.09513 &
  0.12344 &
  0.16233 &
  0.04832 &
  0.06084 &
  0.06497 &
  0.06865 &
  0.07132 \\
\textbf{NextItNet} &
  0.00189 &
  0.00663 &
  0.00947 &
  0.01231 &
  0.01989 &
  0.00189 &
  0.00379 &
  0.00445 &
  0.00479 &
  0.0054 \\
\textbf{SRGNN} &
  0.01562 &
  0.0279 &
  0.04278 &
  0.05952 &
  0.07589 &
  0.01562 &
  0.02083 &
  0.02416 &
  0.02644 &
  0.02753 \\
\textbf{CSRM} &
  0.04406 &
  0.09858 &
  0.1292 &
  0.16729 &
  0.21098 &
  0.04406 &
  0.06647 &
  0.07339 &
  0.0784 &
  0.08139 \\ \hline
\end{tabular}}
\label{tab:size-small}
\end{table*}
