# Supplementary material for: Comprehensive Empirical Evaluation of Deep Learning Approaches for Session-based Recommendation in E-Commerce
Source: arXiv:2010.12540 source file (2020-10-17)
Supplement: Supplementary file 13 [file tab17.tex]

% Please add the following required packages to your document preamble:
% \usepackage{multirow}
% \usepackage[table,xcdraw]{xcolor}
% If you use beamer only pass "xcolor=table" option, i.e. \documentclass[xcolor=table]{beamer}
\begin{table*}[!h]
\centering
\caption{RQ5: training using random 1/256, 1/64, 1/256, 1/64 portions of the full training set for RECSYS, CIKMCUP, TMALL, ROCKET datasets respectively.}
\resizebox{0.9\textwidth}{!}{\begin{tabular}{|c|ccccc|ccccc|}
\hline
\cellcolor[HTML]{333333}{\color[HTML]{FFFFFF} } &
  \multicolumn{5}{c|}{\textbf{HR@}} &
  \multicolumn{5}{c|}{\textbf{MRR@}} \\ \cline{2-11} 
\multirow{-2}{*}{\cellcolor[HTML]{333333}{\color[HTML]{FFFFFF} \textbf{RECSYS}}} &
  \textbf{1} &
  \textbf{3} &
  \textbf{5} &
  \textbf{10} &
  \textbf{20} &
  \textbf{1} &
  \textbf{3} &
  \textbf{5} &
  \textbf{10} &
  \textbf{20} \\ \hline
\textbf{S-POP} &
  0.03827 &
  0.10796 &
  0.13246 &
  0.14926 &
  0.15584 &
  0.03827 &
  0.06891 &
  0.07456 &
  0.07696 &
  0.07743 \\
\textbf{AR} &
  0.07232 &
  0.1408 &
  0.17881 &
  0.23217 &
  0.23257 &
  0.07232 &
  0.10236 &
  0.11112 &
  0.11843 &
  0.11846 \\
\textbf{SR} &
  0.05649 &
  0.11649 &
  0.14106 &
  0.18143 &
  0.21049 &
  0.05649 &
  0.0826 &
  0.08816 &
  0.0938 &
  0.09586 \\
\textbf{VSKNN} &
  0.08639 & 0.16533 & 0.19799 & 0.23072 & 0.25202 & 0.08639 & 0.12113 & 0.12862 & 0.13314 & 0.13466 \\
\textbf{SMF} &
  0.05219 &
  0.12152 &
  0.17083 &
  0.23665 &
  0.30497 &
  0.05219 &
  0.08197 &
  0.09317 &
  0.10198 &
  0.10677 \\
\textbf{Item2Vec} &
  0.03791 &
  0.08272 &
  0.10802 &
  0.15402 &
  0.20422 &
  0.03791 &
  0.0573 &
  0.06305 &
  0.06917 &
  0.07277 \\
\textbf{GRU4Rec+} &
  0.03892 &
  0.09125 &
  0.13167 &
  0.19888 &
  0.27554 &
  0.03892 &
  0.06123 &
  0.0704 &
  0.07924 &
  0.0846 \\
\textbf{NARM} &
  0.08399 &
  0.17221 &
  0.23365 &
  0.31805 &
  0.41573 &
  0.08399 &
  0.121 &
  0.13512 &
  0.14632 &
  0.15213 \\
\textbf{STAMP} &
  0.05689 &
  0.12279 &
  0.16974 &
  0.22895 &
  0.27613 &
  0.05689 &
  0.08432 &
  0.09496 &
  0.10287 &
  0.10614 \\
\textbf{NextItNet} &
  0.04783 &
  0.11017 &
  0.14867 &
  0.20483 &
  0.26758 &
  0.04783 &
  0.07458 &
  0.08323 &
  0.09082 &
  0.09514 \\
\textbf{SRGNN} &
  0.04863 &
  0.12826 &
  0.17498 &
  0.23546 &
  0.28588 &
  0.04863 &
  0.08327 &
  0.0939 &
  0.10201 &
  0.10555 \\
\textbf{CSRM} &
  0.07143 &
  0.16404 &
  0.22736 &
  0.31655 &
  0.39529 &
  0.07143 &
  0.11136 &
  0.12587 &
  0.13775 &
  0.14319 \\ \hline
\cellcolor[HTML]{333333}{\color[HTML]{FFFFFF} } &
  \multicolumn{5}{c|}{\textbf{HR@}} &
  \multicolumn{5}{c|}{\textbf{MRR@}} \\ \cline{2-11} 
\multirow{-2}{*}{\cellcolor[HTML]{333333}{\color[HTML]{FFFFFF} \textbf{CIKMCUP}}} &
  \textbf{1} &
  \textbf{3} &
  \textbf{5} &
  \textbf{10} &
  \textbf{20} &
  \textbf{1} &
  \textbf{3} &
  \textbf{5} &
  \textbf{10} &
  \textbf{20} \\ \hline
\textbf{S-POP} &
  0.04992 &
  0.1188 &
  0.13977 &
  0.15075 &
  0.16007 &
  0.04992 &
  0.08109 &
  0.08585 &
  0.08736 &
  0.088 \\
\textbf{AR} &
  0.03494 &
  0.08053 &
  0.09884 &
  0.13544 &
  0.13577 &
  0.03494 &
  0.05458 &
  0.05875 &
  0.06386 &
  0.06389 \\
\textbf{SR} &
  0.02296 &
  0.05358 &
  0.07022 &
  0.09085 &
  0.09817 &
  0.02296 &
  0.03594 &
  0.03977 &
  0.04264 &
  0.04317 \\
\textbf{VSKNN} &
  0.11390 & 0.20891 & 0.26981 & 0.35100 & 0.43614 & 0.11390 & 0.15553 & 0.16946 & 0.18026 & 0.18618 \\
\textbf{SMF} &
  0.03892 &
  0.09011 &
  0.12938 &
  0.1946 &
  0.26683 &
  0.03892 &
  0.06025 &
  0.06912 &
  0.07768 &
  0.08271 \\
\textbf{Item2Vec} &
  0.00746 &
  0.01669 &
  0.02273 &
  0.03303 &
  0.04119 &
  0.00746 &
  0.01142 &
  0.01275 &
  0.01405 &
  0.01457 \\
\textbf{GRU4Rec+} &
  0.01455 &
  0.03226 &
  0.03795 &
  0.04744 &
  0.05819 &
  0.01455 &
  0.02224 &
  0.02357 &
  0.02475 &
  0.02552 \\
\textbf{NARM} &
  0.04539 &
  0.07754 &
  0.10799 &
  0.14002 &
  0.23091 &
  0.04539 &
  0.05943 &
  0.06637 &
  0.07057 &
  0.07582 \\
\textbf{STAMP} &
  0.02264 &
  0.04794 &
  0.06558 &
  0.08755 &
  0.12017 &
  0.02264 &
  0.03362 &
  0.03772 &
  0.04055 &
  0.04279 \\
\textbf{NextItNet} &
  0.00347 &
  0.00781 &
  0.01042 &
  0.01389 &
  0.0191 &
  0.00347 &
  0.00521 &
  0.00577 &
  0.00625 &
  0.00659 \\
\textbf{SRGNN} &
  0.02051 &
  0.03646 &
  0.04622 &
  0.06413 &
  0.09212 &
  0.02051 &
  0.02734 &
  0.02957 &
  0.03196 &
  0.03392 \\
\textbf{CSRM} &
  0.04088 &
  0.09417 &
  0.12969 &
  0.18231 &
  0.24162 &
  0.04088 &
  0.06356 &
  0.07177 &
  0.07878 &
  0.08287 \\ \hline
\cellcolor[HTML]{333333}{\color[HTML]{FFFFFF} } &
  \multicolumn{5}{c|}{\textbf{HR@}} &
  \multicolumn{5}{c|}{\textbf{MRR@}} \\ \cline{2-11} 
\multirow{-2}{*}{\cellcolor[HTML]{333333}{\color[HTML]{FFFFFF} \textbf{TMALL}}} &
  \textbf{1} &
  \textbf{3} &
  \textbf{5} &
  \textbf{10} &
  \textbf{20} &
  \textbf{1} &
  \textbf{3} &
  \textbf{5} &
  \textbf{10} &
  \textbf{20} \\ \hline
\textbf{S-POP} &
  0.06277 &
  0.14833 &
  0.17862 &
  0.19928 &
  0.20615 &
  0.06277 &
  0.06277 &
  0.06277 &
  0.06277 &
  0.06277 \\
\textbf{AR} &
  0.01093 &
  0.02436 &
  0.03367 &
  0.0457 &
  0.04663 &
  0.01093 &
  0.01681 &
  0.01893 &
  0.02056 &
  0.02063 \\
\textbf{SR} &
  0.00885 &
  0.01863 &
  0.02555 &
  0.03341 &
  0.03773 &
  0.00885 &
  0.01298 &
  0.01452 &
  0.01559 &
  0.01591 \\
\textbf{VSKNN} &
  0.08804 & 0.13645 & 0.16206 & 0.20220 & 0.24390 & 0.08804 & 0.10826 & 0.11423 & 0.12021 & 0.12373 \\
\textbf{SMF} &
  0.01665 &
  0.04044 &
  0.05538 &
  0.08197 &
  0.1119 &
  0.01665 &
  0.02687 &
  0.03025 &
  0.03374 &
  0.03579 \\
\textbf{Item2Vec} &
  0.00367 &
  0.00859 &
  0.01226 &
  0.01807 &
  0.02289 &
  0.00367 &
  0.00588 &
  0.0067 &
  0.00749 &
  0.00783 \\
\textbf{GRU4Rec+} &
  0.01045 &
  0.02163 &
  0.02606 &
  0.03271 &
  0.03965 &
  0.01045 &
  0.01532 &
  0.01633 &
  0.01724 &
  0.01772 \\
\textbf{NARM} &
  0.02656 &
  0.04186 &
  0.05831 &
  0.0743 &
  0.11858 &
  0.02656 &
  0.03313 &
  0.03684 &
  0.03898 &
  0.04154 \\
\textbf{STAMP} &
  0.00781 &
  0.01822 &
  0.02535 &
  0.03544 &
  0.04502 &
  0.00781 &
  0.01232 &
  0.01394 &
  0.01531 &
  0.01599 \\
\textbf{NextItNet} &
  0 &
  0.00199 &
  0.00299 &
  0.00498 &
  0.00936 &
  0 &
  0.00093 &
  0.00116 &
  0.00141 &
  0.0017 \\
\textbf{SRGNN} &
  0.01454 &
  0.03053 &
  0.03849 &
  0.0505 &
  0.06431 &
  0.01454 &
  0.0215 &
  0.02333 &
  0.02494 &
  0.02588 \\
\textbf{CSRM} &
  0.01849 &
  0.03854 &
  0.051 &
  0.06778 &
  0.08352 &
  0.01849 &
  0.02709 &
  0.02995 &
  0.03216 &
  0.03326 \\ \hline
\cellcolor[HTML]{333333}{\color[HTML]{FFFFFF} } &
  \multicolumn{5}{c|}{\textbf{HR@}} &
  \multicolumn{5}{c|}{\textbf{MRR@}} \\ \cline{2-11} 
\multirow{-2}{*}{\cellcolor[HTML]{333333}{\color[HTML]{FFFFFF} \textbf{ROCKET}}} &
  \textbf{1} &
  \textbf{3} &
  \textbf{5} &
  \textbf{10} &
  \textbf{20} &
  \textbf{1} &
  \textbf{3} &
  \textbf{5} &
  \textbf{10} &
  \textbf{20} \\ \hline
\textbf{S-POP} &
  0.04885 &
  0.1235 &
  0.13272 &
  0.14194 &
  0.15115 &
  0.04885 &
  0.08295 &
  0.08512 &
  0.08632 &
  0.08692 \\
\textbf{AR} &
  0.06728 &
  0.10138 &
  0.12166 &
  0.14747 &
  0.14747 &
  0.06728 &
  0.08218 &
  0.08674 &
  0.09041 &
  0.09041 \\
\textbf{SR} &
  0.04055 &
  0.06912 &
  0.08664 &
  0.09585 &
  0.09677 &
  0.04055 &
  0.05253 &
  0.0565 &
  0.05778 &
  0.05786 \\
\textbf{VSKNN} &
  0.21889 & 0.37774 & 0.42527 & 0.48218 & 0.52283 & 0.21889 & 0.28976 & 0.30087 & 0.30872 & 0.31165 \\
\textbf{SMF} &
  0.0424 &
  0.08756 &
  0.11521 &
  0.14839 &
  0.18433 &
  0.0424 &
  0.06206 &
  0.06846 &
  0.07303 &
  0.07557 \\
\textbf{Item2Vec} &
  0.00884 &
  0.01866 &
  0.02259 &
  0.03536 &
  0.04126 &
  0.00884 &
  0.0131 &
  0.01393 &
  0.01563 &
  0.01608 \\
\textbf{GRU4Rec+} &
  0.03568 &
  0.06032 &
  0.07477 &
  0.08241 &
  0.09176 &
  0.03568 &
  0.04673 &
  0.05 &
  0.05097 &
  0.05162 \\
\textbf{NARM} &
  0.0775 &
  0.10681 &
  0.14397 &
  0.17718 &
  0.21746 &
  0.0775 &
  0.09006 &
  0.09854 &
  0.10293 &
  0.10527 \\
\textbf{STAMP} &
  0.02783 &
  0.04917 &
  0.05937 &
  0.07885 &
  0.09833 &
  0.02783 &
  0.03556 &
  0.03788 &
  0.04031 &
  0.04168 \\
\textbf{NextItNet} &
  0.01042 &
  0.0125 &
  0.0125 &
  0.01667 &
  0.01875 &
  0.01042 &
  0.01146 &
  0.01146 &
  0.01199 &
  0.01214 \\
\textbf{SRGNN} &
  0.00434 &
  0.00781 &
  0.01215 &
  0.02517 &
  0.03472 &
  0.00434 &
  0.0055 &
  0.00645 &
  0.00815 &
  0.0088 \\
\textbf{CSRM} &
  0.0537 &
  0.10556 &
  0.13333 &
  0.17593 &
  0.20556 &
  0.0537 &
  0.0767 &
  0.08299 &
  0.08859 &
  0.09051 \\ \hline
\end{tabular}}
\label{tab:size-verysmall}
\end{table*}
