# Supplementary material for: Comprehensive Empirical Evaluation of Deep Learning Approaches for Session-based Recommendation in E-Commerce
Source: arXiv:2010.12540 source file (2020-10-17)
Supplement: Supplementary file 14 [file tab2.tex]

% Please add the following required packages to your document preamble:
% \usepackage{multirow}
% \usepackage[table,xcdraw]{xcolor}
% If you use beamer only pass "xcolor=table" option, i.e. \documentclass[xcolor=table]{beamer}
\begin{table*}[!h]
\centering
\caption{RQ2: training using intermediate sessions of length \textgreater= 5 and \textless 10}
\resizebox{0.9\textwidth}{!}{\begin{tabular}{|c|ccccc|ccccc|}
\hline
\cellcolor[HTML]{333333}{\color[HTML]{FFFFFF} } &
  \multicolumn{5}{c|}{\textbf{HR@}} &
  \multicolumn{5}{c|}{\textbf{MRR@}} \\ \cline{2-11} 
\multirow{-2}{*}{\cellcolor[HTML]{333333}{\color[HTML]{FFFFFF} \textbf{RECSYS}}} &
  \textbf{1} &
  \textbf{3} &
  \textbf{5} &
  \textbf{10} &
  \textbf{20} &
  \textbf{1} &
  \textbf{3} &
  \textbf{5} &
  \textbf{10} &
  \textbf{20} \\ \hline
\textbf{S-POP} &
  0.03547 &
  0.09781 &
  0.12276 &
  0.14267 &
  0.15184 &
  0.03547 &
  0.06286 &
  0.0686 &
  0.07137 &
  0.07203 \\
\textbf{AR} &
  0.10598 &
  0.20605 &
  0.27188 &
  0.33464 &
  0.33476 &
  0.10598 &
  0.14925 &
  0.16427 &
  0.17318 &
  0.17318 \\
\textbf{SR} &
  0.10341 &
  0.20396 &
  0.27026 &
  0.35461 &
  0.44292 &
  0.10341 &
  0.14683 &
  0.16194 &
  0.17319 &
  0.17934 \\
\textbf{VSKNN} &
  0.04063 & 0.06920 & 0.08340 & 0.09837 & 0.10915 & 0.04063 & 0.05305 & 0.05627 & 0.05827 & 0.05902 \\
\textbf{SMF} &
  0.07313 &
  0.20402 &
  0.29364 &
  0.42592 &
  0.55463 &
  0.07313 &
  0.12941 &
  0.14973 &
  0.16747 &
  0.1765 \\
\textbf{Item2Vec} &
  0.06528 &
  0.13535 &
  0.17862 &
  0.24964 &
  0.33291 &
  0.06528 &
  0.0952 &
  0.10501 &
  0.11438 &
  0.1201 \\
\textbf{GRU4Rec+} &
  0.08075 &
  0.19213 &
  0.27336 &
  0.40318 &
  0.53603 &
  0.08075 &
  0.12833 &
  0.14683 &
  0.16403 &
  0.17335 \\
\textbf{NARM} &
  0.09845 &
  0.23784 &
  0.32845 &
  0.46146 &
  0.65748 &
  0.09845 &
  0.15752 &
  0.17854 &
  0.19728 &
  0.20878 \\
\textbf{STAMP} &
  0.11844 &
  0.24822 &
  0.32552 &
  0.44741 &
  0.57275 &
  0.11844 &
  0.1743 &
  0.19192 &
  0.20806 &
  0.21682 \\
\textbf{NextItNet} &
  0.17399 &
  0.32805 &
  0.40625 &
  0.50543 &
  0.60462 &
  0.17399 &
  0.24054 &
  0.25829 &
  0.27152 &
  0.27847 \\
\textbf{SRGNN} &
  0.12678 &
  0.26065 &
  0.34112 &
  0.46363 &
  0.58693 &
  0.12678 &
  0.18436 &
  0.20263 &
  0.21893 &
  0.22751 \\
\textbf{CSRM} &
  0.1372 &
  0.27576 &
  0.36188 &
  0.50036 &
  0.63671 &
  0.1372 &
  0.1968 &
  0.21635 &
  0.2348 &
  0.24435 \\ \hline
\cellcolor[HTML]{333333}{\color[HTML]{FFFFFF} } &
  \multicolumn{5}{c|}{\textbf{HR@}} &
  \multicolumn{5}{c|}{\textbf{MRR@}} \\ \cline{2-11} 
\multirow{-2}{*}{\cellcolor[HTML]{333333}{\color[HTML]{FFFFFF} \textbf{CIKMCUP}}} &
  \textbf{1} &
  \textbf{3} &
  \textbf{5} &
  \textbf{10} &
  \textbf{20} &
  \textbf{1} &
  \textbf{3} &
  \textbf{5} &
  \textbf{10} &
  \textbf{20} \\ \hline
\textbf{S-POP} &
  0.03931 &
  0.10119 &
  0.11757 &
  0.13055 &
  0.13431 &
  0.03931 &
  0.06614 &
  0.07001 &
  0.07181 &
  0.07206 \\
\textbf{AR} &
  0.04234 &
  0.10095 &
  0.1388 &
  0.18964 &
  0.18964 &
  0.04234 &
  0.0673 &
  0.07587 &
  0.08299 &
  0.08299 \\
\textbf{SR} &
  0.04004 &
  0.08991 &
  0.12339 &
  0.17629 &
  0.22555 &
  0.04004 &
  0.06153 &
  0.06919 &
  0.07625 &
  0.07969 \\
\textbf{VSKNN} &
  0.05069 & 0.10094 & 0.13116 & 0.17687 & 0.21848 & 0.05069 & 0.07244 & 0.07936 & 0.08558 & 0.08847 \\
\textbf{SMF} &
  0.03531 &
  0.09415 &
  0.14014 &
  0.22834 &
  0.33827 &
  0.03531 &
  0.0602 &
  0.07067 &
  0.08237 &
  0.08985 \\
\textbf{Item2Vec} &
  0.0152 &
  0.0354 &
  0.05291 &
  0.08515 &
  0.12833 &
  0.0152 &
  0.02378 &
  0.02772 &
  0.03191 &
  0.03483 \\
\textbf{GRU4Rec+} &
  0.02549 &
  0.07007 &
  0.1057 &
  0.17045 &
  0.25489 &
  0.02549 &
  0.04417 &
  0.05222 &
  0.06074 &
  0.06648 \\
\textbf{NARM} &
  0.04467 &
  0.115 &
  0.16946 &
  0.25691 &
  0.43963 &
  0.04467 &
  0.07474 &
  0.08692 &
  0.09852 &
  0.10913 \\
\textbf{STAMP} &
  0.0375 &
  0.09137 &
  0.13554 &
  0.21709 &
  0.31853 &
  0.0375 &
  0.06057 &
  0.07064 &
  0.08148 &
  0.0884 \\
\textbf{NextItNet} &
  0.02987 &
  0.06342 &
  0.09191 &
  0.13787 &
  0.19623 &
  0.02987 &
  0.04427 &
  0.05077 &
  0.05683 &
  0.06083 \\
\textbf{SRGNN} &
  0.04748 &
  0.10697 &
  0.15517 &
  0.25072 &
  0.35661 &
  0.04748 &
  0.07274 &
  0.08364 &
  0.09612 &
  0.10345 \\
\textbf{CSRM} &
  0.04246 &
  0.1129 &
  0.16326 &
  0.24939 &
  0.36703 &
  0.04246 &
  0.07208 &
  0.08349 &
  0.09499 &
  0.10312 \\ \hline
\cellcolor[HTML]{333333}{\color[HTML]{FFFFFF} } &
  \multicolumn{5}{c|}{\textbf{HR@}} &
  \multicolumn{5}{c|}{\textbf{MRR@}} \\ \cline{2-11} 
\multirow{-2}{*}{\cellcolor[HTML]{333333}{\color[HTML]{FFFFFF} \textbf{TMALL}}} &
  \textbf{1} &
  \textbf{3} &
  \textbf{5} &
  \textbf{10} &
  \textbf{20} &
  \textbf{1} &
  \textbf{3} &
  \textbf{5} &
  \textbf{10} &
  \textbf{20} \\ \hline
\textbf{S-POP} &
  0.047 &
  0.10821 &
  0.13787 &
  0.17055 &
  0.18977 &
  0.047 &
  0.07359 &
  0.08036 &
  0.0848 &
  0.08617 \\
\textbf{AR} &
  0.01572 &
  0.03081 &
  0.04054 &
  0.05225 &
  0.05243 &
  0.01572 &
  0.02217 &
  0.02438 &
  0.02602 &
  0.02603 \\
\textbf{SR} &
  0.0139 &
  0.02734 &
  0.03571 &
  0.04706 &
  0.05846 &
  0.0139 &
  0.01968 &
  0.02157 &
  0.02309 &
  0.02389 \\
\textbf{VSKNN} &
  0.02450 & 0.04068 & 0.04991 & 0.06327 & 0.07359 & 0.02450 & 0.03160 & 0.03345 & 0.03563 & 0.03637 \\
\textbf{SMF} &
  0.01563 &
  0.04054 &
  0.05804 &
  0.08576 &
  0.11923 &
  0.01563 &
  0.02624 &
  0.03019 &
  0.03386 &
  0.03617 \\
\textbf{Item2Vec} &
  0.00224 &
  0.00463 &
  0.00677 &
  0.01118 &
  0.01746 &
  0.00224 &
  0.00327 &
  0.00375 &
  0.00434 &
  0.00476 \\
\textbf{GRU4Rec+} &
  0.02212 &
  0.05056 &
  0.0687 &
  0.09553 &
  0.12324 &
  0.02212 &
  0.03428 &
  0.03839 &
  0.04198 &
  0.0439 \\
\textbf{NARM} &
  0.03582 &
  0.07501 &
  0.10016 &
  0.13375 &
  0.19952 &
  0.03582 &
  0.05294 &
  0.05849 &
  0.06277 &
  0.06665 \\
\textbf{STAMP} &
  0.02378 &
  0.05065 &
  0.06745 &
  0.09238 &
  0.12075 &
  0.02378 &
  0.03533 &
  0.03915 &
  0.04246 &
  0.04444 \\
\textbf{NextItNet} &
  0.02382 &
  0.04556 &
  0.05813 &
  0.07791 &
  0.09495 &
  0.02382 &
  0.03322 &
  0.03605 &
  0.0387 &
  0.03987 \\
\textbf{SRGNN} &
  0.0372 &
  0.07477 &
  0.09626 &
  0.12867 &
  0.16531 &
  0.0372 &
  0.05336 &
  0.05824 &
  0.06254 &
  0.06506 \\
\textbf{CSRM} &
  0.03124 &
  0.06581 &
  0.08688 &
  0.11989 &
  0.15569 &
  0.03124 &
  0.04618 &
  0.05099 &
  0.05539 &
  0.05786 \\ \hline
\cellcolor[HTML]{333333}{\color[HTML]{FFFFFF} } &
  \multicolumn{5}{c|}{\textbf{HR@}} &
  \multicolumn{5}{c|}{\textbf{MRR@}} \\ \cline{2-11} 
\multirow{-2}{*}{\cellcolor[HTML]{333333}{\color[HTML]{FFFFFF} \textbf{ROCKET}}} &
  \textbf{1} &
  \textbf{3} &
  \textbf{5} &
  \textbf{10} &
  \textbf{20} &
  \textbf{1} &
  \textbf{3} &
  \textbf{5} &
  \textbf{10} &
  \textbf{20} \\ \hline
\textbf{S-POP} &
  0.03978 &
  0.11384 &
  0.12876 &
  0.14446 &
  0.15362 &
  0.03978 &
  0.07376 &
  0.07728 &
  0.07937 &
  0.08003 \\
\textbf{AR} &
  0.05444 &
  0.10468 &
  0.13845 &
  0.17927 &
  0.1798 &
  0.05444 &
  0.07611 &
  0.08381 &
  0.08951 &
  0.08954 \\
\textbf{SR} &
  0.04449 &
  0.09657 &
  0.12353 &
  0.15781 &
  0.18398 &
  0.04449 &
  0.06691 &
  0.07307 &
  0.07771 &
  0.07951 \\
\textbf{VSKNN} &
  0.11272 & 0.18481 & 0.22810 & 0.26302 & 0.29304 & 0.11272 & 0.14400 & 0.15403 & 0.15884 & 0.16095 \\
\textbf{SMF} &
  0.039 &
  0.10207 &
  0.15284 &
  0.2201 &
  0.29547 &
  0.039 &
  0.06525 &
  0.07681 &
  0.08564 &
  0.09089 \\
\textbf{Item2Vec} &
  0.02171 &
  0.04629 &
  0.06276 &
  0.09493 &
  0.12945 &
  0.02171 &
  0.03203 &
  0.03583 &
  0.04004 &
  0.0425 \\
\textbf{GRU4Rec+} &
  0.03417 &
  0.07981 &
  0.11502 &
  0.16771 &
  0.21857 &
  0.03417 &
  0.05373 &
  0.06185 &
  0.06873 &
  0.07228 \\
\textbf{NARM} &
  0.11004 &
  0.18413 &
  0.22816 &
  0.28578 &
  0.38245 &
  0.11004 &
  0.1428 &
  0.15309 &
  0.16052 &
  0.16624 \\
\textbf{STAMP} &
  0.03792 &
  0.08428 &
  0.10982 &
  0.16434 &
  0.21148 &
  0.03792 &
  0.05733 &
  0.06312 &
  0.0704 &
  0.07364 \\
\textbf{NextItNet} &
  0.0327 &
  0.06177 &
  0.08576 &
  0.10901 &
  0.1439 &
  0.0327 &
  0.04494 &
  0.05013 &
  0.05328 &
  0.05561 \\
\textbf{SRGNN} &
  0.06563 &
  0.14427 &
  0.19193 &
  0.24948 &
  0.30703 &
  0.06563 &
  0.09939 &
  0.11033 &
  0.11796 &
  0.1219 \\
\textbf{CSRM} &
  0.07186 &
  0.14397 &
  0.18693 &
  0.24603 &
  0.31138 &
  0.07186 &
  0.10245 &
  0.1123 &
  0.1201 &
  0.12463 \\ \hline
\end{tabular}}
\label{tab:train-intermediate}
\end{table*}
