# Supplementary material for: Comprehensive Empirical Evaluation of Deep Learning Approaches for Session-based Recommendation in E-Commerce
Source: arXiv:2010.12540 source file (2020-10-17)
Supplement: Supplementary file 15 [file tab20.tex]

% Please add the following required packages to your document preamble:
% \usepackage{multirow}
% \usepackage[table,xcdraw]{xcolor}
% If you use beamer only pass "xcolor=table" option, i.e. \documentclass[xcolor=table]{beamer}
\begin{table*}[!h]
\centering
\caption{RQ3: performance of predictions on items whose frequency is very low in the training set \textless{}50 (\textless{}10) for RECSYS and TMALL (CIKMCUP and ROCKET).}
\resizebox{0.9\textwidth}{!}{\begin{tabular}{|c|ccccc|ccccc|}
\hline
\cellcolor[HTML]{333333}{\color[HTML]{FFFFFF} } &
  \multicolumn{5}{c|}{\textbf{HR@}} &
  \multicolumn{5}{c|}{\textbf{MRR@}} \\ \cline{2-11} 
\multirow{-2}{*}{\cellcolor[HTML]{333333}{\color[HTML]{FFFFFF} \textbf{RECSYS}}} &
  \textbf{1} &
  \textbf{3} &
  \textbf{5} &
  \textbf{10} &
  \textbf{20} &
  \textbf{1} &
  \textbf{3} &
  \textbf{5} &
  \textbf{10} &
  \textbf{20} \\ \hline
\textbf{S-POP} &
  0.02672 &
  0.07818 &
  0.09101 &
  0.09788 &
  0.10246 &
  0.02672 &
  0.04942 &
  0.05233 &
  0.0533 &
  0.05363 \\
\textbf{AR} &
  0.04672 &
  0.10215 &
  0.1443 &
  0.20079 &
  0.2011 &
  0.04672 &
  0.07055 &
  0.08025 &
  0.08801 &
  0.08803 \\
\textbf{SR} &
  0.04779 &
  0.10368 &
  0.14384 &
  0.19499 &
  0.23927 &
  0.04779 &
  0.07187 &
  0.0809 &
  0.08774 &
  0.09091 \\
\textbf{VSKNN} &
  0.13741 & 0.21331 & 0.24221 & 0.28548 & 0.32004 & 0.13741 & 0.17086 & 0.17753 & 0.18337 & 0.18581 \\
\textbf{SMF} &
  0.05181 &
  0.14053 &
  0.20131 &
  0.30308 &
  0.41628 &
  0.05181 &
  0.0893 &
  0.10311 &
  0.11659 &
  0.12452 \\
\textbf{Item2Vec} &
  0.03446 &
  0.08271 &
  0.1138 &
  0.16674 &
  0.23625 &
  0.03446 &
  0.05475 &
  0.06174 &
  0.06878 &
  0.07359 \\
\textbf{GRU4Rec+} &
  0.06429 &
  0.15171 &
  0.20933 &
  0.30125 &
  0.38534 &
  0.06429 &
  0.1013 &
  0.11431 &
  0.12661 &
  0.13245 \\
\textbf{NARM} &
  0.08034 &
  0.2361 &
  0.32998 &
  0.46588 &
  0.62454 &
  0.08034 &
  0.14917 &
  0.17048 &
  0.18861 &
  0.19839 \\
\textbf{STAMP} &
  0.12098 &
  0.22935 &
  0.29511 &
  0.41309 &
  0.53335 &
  0.12098 &
  0.16756 &
  0.18261 &
  0.19821 &
  0.20663 \\
\textbf{NextItNet} &
  0.0636 &
  0.13667 &
  0.17952 &
  0.23726 &
  0.30041 &
  0.0636 &
  0.0951 &
  0.10464 &
  0.11247 &
  0.11689 \\
\textbf{SRGNN} &
  0.12395 &
  0.24873 &
  0.32603 &
  0.44362 &
  0.5565 &
  0.12395 &
  0.17751 &
  0.19498 &
  0.21077 &
  0.21875 \\
\textbf{CSRM} &
  0.15963 &
  0.30709 &
  0.38835 &
  0.51266 &
  0.62165 &
  0.15963 &
  0.22229 &
  0.24086 &
  0.25754 &
  0.26518 \\ \hline
\cellcolor[HTML]{333333}{\color[HTML]{FFFFFF} } &
  \multicolumn{5}{c|}{\textbf{HR@}} &
  \multicolumn{5}{c|}{\textbf{MRR@}} \\ \cline{2-11} 
\multirow{-2}{*}{\cellcolor[HTML]{333333}{\color[HTML]{FFFFFF} \textbf{CIKMCUP}}} &
  \textbf{1} &
  \textbf{3} &
  \textbf{5} &
  \textbf{10} &
  \textbf{20} &
  \textbf{1} &
  \textbf{3} &
  \textbf{5} &
  \textbf{10} &
  \textbf{20} \\ \hline
\textbf{S-POP} &
  0.02114 &
  0.05968 &
  0.06932 &
  0.07212 &
  0.07212 &
  0.02114 &
  0.03834 &
  0.04055 &
  0.04094 &
  0.04094 \\
\textbf{AR} &
  0.0115 &
  0.0373 &
  0.05657 &
  0.10134 &
  0.10134 &
  0.0115 &
  0.02254 &
  0.02686 &
  0.03287 &
  0.03287 \\
\textbf{SR} &
  0.01616 &
  0.03792 &
  0.05284 &
  0.08579 &
  0.10724 &
  0.01616 &
  0.02528 &
  0.02869 &
  0.03311 &
  0.03469 \\
\textbf{VSKNN} &
  0.09519 & 0.14978 & 0.17844 & 0.22689 & 0.27909 & 0.09519 & 0.11862 & 0.12518 & 0.13162 & 0.13525 \\
\textbf{SMF} &
  0.01407 &
  0.03498 &
  0.05227 &
  0.09811 &
  0.17169 &
  0.01407 &
  0.02285 &
  0.02685 &
  0.03282 &
  0.0378 \\
\textbf{Item2Vec} &
  0.02587 &
  0.05851 &
  0.07792 &
  0.12673 &
  0.19053 &
  0.02587 &
  0.03979 &
  0.04414 &
  0.0506 &
  0.05494 \\
\textbf{GRU4Rec+} &
  0.01137 &
  0.03107 &
  0.04358 &
  0.06859 &
  0.10231 &
  0.01137 &
  0.0197 &
  0.02258 &
  0.02578 &
  0.02793 \\
\textbf{NARM} &
  0.02947 &
  0.10465 &
  0.14566 &
  0.22695 &
  0.43636 &
  0.02947 &
  0.06205 &
  0.07034 &
  0.08001 &
  0.0923 \\
\textbf{STAMP} &
  0.04482 &
  0.1051 &
  0.1391 &
  0.22411 &
  0.29985 &
  0.04482 &
  0.07084 &
  0.07826 &
  0.0891 &
  0.09402 \\
\textbf{NextItNet} &
  0.00813 &
  0.02078 &
  0.02529 &
  0.03523 &
  0.04968 &
  0.00813 &
  0.01325 &
  0.01424 &
  0.01563 &
  0.01658 \\
\textbf{SRGNN} &
  0.03101 &
  0.09884 &
  0.15698 &
  0.24419 &
  0.34109 &
  0.03101 &
  0.0604 &
  0.07377 &
  0.08433 &
  0.09079 \\
\textbf{CSRM} &
  0.04553 &
  0.13835 &
  0.18739 &
  0.27671 &
  0.38179 &
  0.04553 &
  0.0864 &
  0.09726 &
  0.1086 &
  0.11593 \\ \hline
\cellcolor[HTML]{333333}{\color[HTML]{FFFFFF} } &
  \multicolumn{5}{c|}{\textbf{HR@}} &
  \multicolumn{5}{c|}{\textbf{MRR@}} \\ \cline{2-11} 
\multirow{-2}{*}{\cellcolor[HTML]{333333}{\color[HTML]{FFFFFF} \textbf{TMALL}}} &
  \textbf{1} &
  \textbf{3} &
  \textbf{5} &
  \textbf{10} &
  \textbf{20} &
  \textbf{1} &
  \textbf{3} &
  \textbf{5} &
  \textbf{10} &
  \textbf{20} \\ \hline
\textbf{S-POP} &
  0.04196 &
  0.10066 &
  0.12941 &
  0.15821 &
  0.17322 &
  0.04196 &
  0.04196 &
  0.04196 &
  0.04196 &
  0.04196 \\
\textbf{AR} &
  0.00814 &
  0.01958 &
  0.0282 &
  0.04123 &
  0.04145 &
  0.00814 &
  0.013 &
  0.01495 &
  0.01673 &
  0.01674 \\
\textbf{SR} &
  0.00738 &
  0.01757 &
  0.02373 &
  0.03414 &
  0.04448 &
  0.00738 &
  0.01167 &
  0.01306 &
  0.01446 &
  0.01518 \\
\textbf{VSKNN} &
  0.02641 & 0.04328 & 0.05241 & 0.06738 & 0.08610 & 0.02641 & 0.03375 & 0.03533 & 0.03716 & 0.03995 \\
\textbf{SMF} &
  0.01304 &
  0.0326 &
  0.04627 &
  0.07079 &
  0.10386 &
  0.01304 &
  0.02136 &
  0.02445 &
  0.02769 &
  0.02995 \\
\textbf{Item2Vec} &
  0.00292 &
  0.00668 &
  0.00976 &
  0.01516 &
  0.02302 &
  0.00292 &
  0.0045 &
  0.00519 &
  0.0059 &
  0.00644 \\
\textbf{GRU4Rec+} &
  0.01201 &
  0.0277 &
  0.03803 &
  0.05436 &
  0.07098 &
  0.01201 &
  0.01875 &
  0.02108 &
  0.02325 &
  0.02439 \\
\textbf{NARM} &
  0.02416 &
  0.06621 &
  0.08979 &
  0.12782 &
  0.21946 &
  0.02416 &
  0.0429 &
  0.0476 &
  0.05232 &
  0.0586 \\
\textbf{STAMP} &
  0.03802 &
  0.07837 &
  0.10038 &
  0.13486 &
  0.17179 &
  0.03802 &
  0.0554 &
  0.06041 &
  0.06504 &
  0.06762 \\
\textbf{NextItNet} &
  0.00174 &
  0.00456 &
  0.00644 &
  0.011 &
  0.0153 &
  0.00174 &
  0.003 &
  0.0034 &
  0.004 &
  0.00428 \\
\textbf{SRGNN} &
  0.03354 &
  0.06643 &
  0.08458 &
  0.11415 &
  0.14619 &
  0.03354 &
  0.04771 &
  0.05181 &
  0.05572 &
  0.05796 \\
\textbf{CSRM} &
  0.02655 &
  0.05172 &
  0.06751 &
  0.09239 &
  0.11916 &
  0.02655 &
  0.03724 &
  0.04083 &
  0.0441 &
  0.04597 \\ \hline
\cellcolor[HTML]{333333}{\color[HTML]{FFFFFF} } &
  \multicolumn{5}{c|}{\textbf{HR@}} &
  \multicolumn{5}{c|}{\textbf{MRR@}} \\ \cline{2-11} 
\multirow{-2}{*}{\cellcolor[HTML]{333333}{\color[HTML]{FFFFFF} \textbf{ROCKET}}} &
  \textbf{1} &
  \textbf{3} &
  \textbf{5} &
  \textbf{10} &
  \textbf{20} &
  \textbf{1} &
  \textbf{3} &
  \textbf{5} &
  \textbf{10} &
  \textbf{20} \\ \hline
\textbf{S-POP} &
  0.02277 &
  0.07005 &
  0.08056 &
  0.08494 &
  0.08494 &
  0.02277 &
  0.0432 &
  0.04565 &
  0.04632 &
  0.04632 \\
\textbf{AR} &
  0.02539 &
  0.04466 &
  0.06217 &
  0.08932 &
  0.09019 &
  0.02539 &
  0.03371 &
  0.03765 &
  0.04114 &
  0.04119 \\
\textbf{SR} &
  0.02014 &
  0.04028 &
  0.06042 &
  0.07618 &
  0.08844 &
  0.02014 &
  0.02846 &
  0.03292 &
  0.0351 &
  0.03595 \\
\textbf{VSKNN} &
  0.32281 & 0.40963 & 0.43962 & 0.46567 & 0.49408 & 0.32281 & 0.36135 & 0.36826 & 0.37180 & 0.37378 \\
\textbf{SMF} &
  0.01425 &
  0.03238 &
  0.03886 &
  0.06606 &
  0.09974 &
  0.01425 &
  0.02245 &
  0.02394 &
  0.02766 &
  0.0299 \\
\textbf{Item2Vec} &
  0.02418 &
  0.05872 &
  0.06908 &
  0.09845 &
  0.13126 &
  0.02418 &
  0.03915 &
  0.04131 &
  0.04481 &
  0.04719 \\
\textbf{GRU4Rec+} &
  0.02048 &
  0.05301 &
  0.06506 &
  0.08434 &
  0.09759 &
  0.02048 &
  0.03474 &
  0.03739 &
  0.03995 &
  0.04085 \\
\textbf{NARM} &
  0.08225 &
  0.12143 &
  0.14272 &
  0.14219 &
  0.25201 &
  0.08225 &
  0.09959 &
  0.11455 &
  0.11418 &
  0.12349 \\
\textbf{STAMP} &
  0.05128 &
  0.11111 &
  0.12821 &
  0.16239 &
  0.20513 &
  0.05128 &
  0.07123 &
  0.07507 &
  0.07959 &
  0.08255 \\
\textbf{NextItNet} &
  0.02658 &
  0.04319 &
  0.04817 &
  0.06645 &
  0.07475 &
  0.02658 &
  0.0335 &
  0.03458 &
  0.0373 &
  0.03789 \\
\textbf{SRGNN} &
  0.04255 &
  0.09574 &
  0.1383 &
  0.17021 &
  0.21277 &
  0.04255 &
  0.06383 &
  0.0734 &
  0.07776 &
  0.08034 \\
\textbf{CSRM} &
  0.02564 &
  0.10256 &
  0.15385 &
  0.20513 &
  0.33333 &
  0.02564 &
  0.05556 &
  0.06581 &
  0.07094 &
  0.07786 \\ \hline
\end{tabular}}
\label{tab:freq-verylow}
\end{table*}
