# Supplementary material for: Comprehensive Empirical Evaluation of Deep Learning Approaches for Session-based Recommendation in E-Commerce
Source: arXiv:2010.12540 source file (2020-10-17)
Supplement: Supplementary file 16 [file tab21.tex]

% Please add the following required packages to your document preamble:
% \usepackage{multirow}
% \usepackage[table,xcdraw]{xcolor}
% If you use beamer only pass "xcolor=table" option, i.e. \documentclass[xcolor=table]{beamer}
\begin{table*}[!h]
\centering
\caption{RQ3: performance of predictions on items whose frequency is very low in the training set \textless{}100 (\textless{}30) for RECSYS and TMALL (CIKMCUP and ROCKET).}
\resizebox{0.9\textwidth}{!}{\begin{tabular}{|c|ccccc|ccccc|}
\hline
\cellcolor[HTML]{333333}{\color[HTML]{FFFFFF} } &
  \multicolumn{5}{c|}{\textbf{HR@}} &
  \multicolumn{5}{c|}{\textbf{MRR@}} \\ \cline{2-11} 
\multirow{-2}{*}{\cellcolor[HTML]{333333}{\color[HTML]{FFFFFF} \textbf{RECSYS}}} &
  \textbf{1} &
  \textbf{3} &
  \textbf{5} &
  \textbf{10} &
  \textbf{20} &
  \textbf{1} &
  \textbf{3} &
  \textbf{5} &
  \textbf{10} &
  \textbf{20} \\ \hline
\textbf{S-POP} &
  0.02695 &
  0.08126 &
  0.09597 &
  0.10512 &
  0.10831 &
  0.02695 &
  0.051 &
  0.0544 &
  0.0557 &
  0.05592 \\
\textbf{AR} &
  0.05688 &
  0.12251 &
  0.16365 &
  0.21755 &
  0.21775 &
  0.05688 &
  0.08546 &
  0.0949 &
  0.1024 &
  0.10241 \\
\textbf{SR} &
  0.05791 &
  0.12734 &
  0.16941 &
  0.22269 &
  0.27268 &
  0.05791 &
  0.08764 &
  0.09716 &
  0.10439 &
  0.10792 \\
\textbf{VSKNN} &
  0.12074 & 0.18992 & 0.22056 & 0.26080 & 0.29291 & 0.12074 & 0.15110 & 0.15810 & 0.16353 & 0.16575 \\
\textbf{SMF} &
  0.06594 &
  0.17402 &
  0.24493 &
  0.34659 &
  0.44747 &
  0.06594 &
  0.11189 &
  0.12805 &
  0.14158 &
  0.14862 \\
\textbf{Item2Vec} &
  0.0324 &
  0.07573 &
  0.10743 &
  0.1612 &
  0.23151 &
  0.0324 &
  0.05083 &
  0.05795 &
  0.06508 &
  0.06994 \\
\textbf{GRU4Rec+} &
  0.06826 &
  0.16189 &
  0.22735 &
  0.31997 &
  0.41005 &
  0.06826 &
  0.10799 &
  0.12285 &
  0.13518 &
  0.14134 \\
\textbf{NARM} &
  0.11233 &
  0.24556 &
  0.35038 &
  0.49457 &
  0.66912 &
  0.11233 &
  0.16821 &
  0.19217 &
  0.21134 &
  0.2218 \\
\textbf{STAMP} &
  0.11916 &
  0.23721 &
  0.30625 &
  0.42528 &
  0.54227 &
  0.11916 &
  0.16944 &
  0.18517 &
  0.20097 &
  0.20906 \\
\textbf{NextItNet} &
  0.07584 &
  0.15075 &
  0.20069 &
  0.26998 &
  0.35737 &
  0.07584 &
  0.10752 &
  0.11888 &
  0.1282 &
  0.13427 \\
\textbf{SRGNN} &
  0.12279 &
  0.25396 &
  0.33067 &
  0.4562 &
  0.57389 &
  0.12279 &
  0.17922 &
  0.19677 &
  0.21356 &
  0.22176 \\
\textbf{CSRM} &
  0.15037 &
  0.30973 &
  0.4074 &
  0.55025 &
  0.66913 &
  0.15037 &
  0.2186 &
  0.24088 &
  0.26026 &
  0.26866 \\ \hline
\cellcolor[HTML]{333333}{\color[HTML]{FFFFFF} } &
  \multicolumn{5}{c|}{\textbf{HR@}} &
  \multicolumn{5}{c|}{\textbf{MRR@}} \\ \cline{2-11} 
\multirow{-2}{*}{\cellcolor[HTML]{333333}{\color[HTML]{FFFFFF} \textbf{CIKMCUP}}} &
  \textbf{1} &
  \textbf{3} &
  \textbf{5} &
  \textbf{10} &
  \textbf{20} &
  \textbf{1} &
  \textbf{3} &
  \textbf{5} &
  \textbf{10} &
  \textbf{20} \\ \hline
\textbf{S-POP} &
  0.03021 &
  0.08365 &
  0.09455 &
  0.09973 &
  0.10045 &
  0.03021 &
  0.05401 &
  0.0565 &
  0.05727 &
  0.05734 \\
\textbf{AR} &
  0.02556 &
  0.06577 &
  0.09687 &
  0.14799 &
  0.14799 &
  0.02556 &
  0.04257 &
  0.04963 &
  0.05661 &
  0.05661 \\
\textbf{SR} &
  0.02627 &
  0.05773 &
  0.08061 &
  0.12654 &
  0.16783 &
  0.02627 &
  0.03971 &
  0.04493 &
  0.05114 &
  0.05408 \\
\textbf{VSKNN} &
  0.06555 & 0.11554 & 0.14333 & 0.18738 & 0.23108 & 0.06555 & 0.08687 & 0.09318 & 0.09894 & 0.10202 \\
\textbf{SMF} &
  0.02414 &
  0.07321 &
  0.11041 &
  0.1854 &
  0.2869 &
  0.02414 &
  0.04449 &
  0.05297 &
  0.0629 &
  0.06989 \\
\textbf{Item2Vec} &
  0.02322 &
  0.05529 &
  0.07816 &
  0.12409 &
  0.18839 &
  0.02322 &
  0.03671 &
  0.04182 &
  0.04784 &
  0.05224 \\
\textbf{GRU4Rec+} &
  0.02298 &
  0.05707 &
  0.08158 &
  0.13596 &
  0.19341 &
  0.02298 &
  0.03757 &
  0.04305 &
  0.05003 &
  0.05401 \\
\textbf{NARM} &
  0.02766 &
  0.10442 &
  0.17503 &
  0.26153 &
  0.46585 &
  0.02766 &
  0.06129 &
  0.07726 &
  0.08871 &
  0.10073 \\
\textbf{STAMP} &
  0.04555 &
  0.12263 &
  0.1773 &
  0.2691 &
  0.39033 &
  0.04555 &
  0.07755 &
  0.09003 &
  0.10213 &
  0.11029 \\
\textbf{NextItNet} &
  0.02024 &
  0.03512 &
  0.04702 &
  0.075 &
  0.11964 &
  0.02024 &
  0.02679 &
  0.02926 &
  0.03304 &
  0.03599 \\
\textbf{SRGNN} &
  0.05455 &
  0.14805 &
  0.19654 &
  0.29957 &
  0.42857 &
  0.05455 &
  0.09307 &
  0.10416 &
  0.11748 &
  0.1262 \\
\textbf{CSRM} &
  0.04689 &
  0.11579 &
  0.17416 &
  0.27464 &
  0.3933 &
  0.04689 &
  0.07703 &
  0.09033 &
  0.10362 &
  0.1118 \\ \hline
\cellcolor[HTML]{333333}{\color[HTML]{FFFFFF} } &
  \multicolumn{5}{c|}{\textbf{HR@}} &
  \multicolumn{5}{c|}{\textbf{MRR@}} \\ \cline{2-11} 
\multirow{-2}{*}{\cellcolor[HTML]{333333}{\color[HTML]{FFFFFF} \textbf{TMALL}}} &
  \textbf{1} &
  \textbf{3} &
  \textbf{5} &
  \textbf{10} &
  \textbf{20} &
  \textbf{1} &
  \textbf{3} &
  \textbf{5} &
  \textbf{10} &
  \textbf{20} \\ \hline
\textbf{S-POP} &
  0.04561 &
  0.10708 &
  0.13657 &
  0.16644 &
  0.18252 &
  0.04561 &
  0.04561 &
  0.04561 &
  0.04561 &
  0.04561 \\
\textbf{AR} &
  0.00981 &
  0.02261 &
  0.03158 &
  0.04444 &
  0.04466 &
  0.00981 &
  0.01528 &
  0.01731 &
  0.01908 &
  0.01909 \\
\textbf{SR} &
  0.00912 &
  0.02027 &
  0.027 &
  0.03775 &
  0.04889 &
  0.00912 &
  0.01384 &
  0.01536 &
  0.01679 &
  0.01757 \\
\textbf{VSKNN} &
  0.03349 & 0.05237 & 0.06080 & 0.07669 & 0.09465 & 0.03349 & 0.04198 & 0.04243 & 0.04484 & 0.04668 \\
\textbf{SMF} &
  0.01462 &
  0.03588 &
  0.0506 &
  0.0765 &
  0.10856 &
  0.01462 &
  0.0236 &
  0.02694 &
  0.03035 &
  0.03256 \\
\textbf{Item2Vec} &
  0.00274 &
  0.0067 &
  0.00925 &
  0.01468 &
  0.02201 &
  0.00274 &
  0.00438 &
  0.00495 &
  0.00567 &
  0.00618 \\
\textbf{GRU4Rec+} &
  0.01522 &
  0.03423 &
  0.04578 &
  0.06377 &
  0.08204 &
  0.01522 &
  0.02344 &
  0.02607 &
  0.02848 &
  0.02973 \\
\textbf{NARM} &
  0.01687 &
  0.05475 &
  0.0836 &
  0.1073 &
  0.17362 &
  0.01687 &
  0.03391 &
  0.04091 &
  0.04437 &
  0.04879 \\
\textbf{STAMP} &
  0.03921 &
  0.08325 &
  0.10896 &
  0.1444 &
  0.18418 &
  0.03921 &
  0.0581 &
  0.06397 &
  0.0687 &
  0.07147 \\
\textbf{NextItNet} &
  0.00381 &
  0.0086 &
  0.01192 &
  0.01622 &
  0.02322 &
  0.00381 &
  0.00588 &
  0.00663 &
  0.00718 &
  0.00766 \\
\textbf{SRGNN} &
  0.03476 &
  0.06983 &
  0.09004 &
  0.11958 &
  0.15417 &
  0.03476 &
  0.04987 &
  0.05447 &
  0.05838 &
  0.06079 \\
\textbf{CSRM} &
  0.02613 &
  0.05198 &
  0.06864 &
  0.09654 &
  0.12634 &
  0.02613 &
  0.03719 &
  0.04097 &
  0.04468 &
  0.04676 \\ \hline
\cellcolor[HTML]{333333}{\color[HTML]{FFFFFF} } &
  \multicolumn{5}{c|}{\textbf{HR@}} &
  \multicolumn{5}{c|}{\textbf{MRR@}} \\ \cline{2-11} 
\multirow{-2}{*}{\cellcolor[HTML]{333333}{\color[HTML]{FFFFFF} \textbf{ROCKET}}} &
  \textbf{1} &
  \textbf{3} &
  \textbf{5} &
  \textbf{10} &
  \textbf{20} &
  \textbf{1} &
  \textbf{3} &
  \textbf{5} &
  \textbf{10} &
  \textbf{20} \\ \hline
\textbf{S-POP} &
  0.0221 &
  0.07656 &
  0.09195 &
  0.09629 &
  0.09747 &
  0.0221 &
  0.0463 &
  0.04991 &
  0.05049 &
  0.05057 \\
\textbf{AR} &
  0.02881 &
  0.05485 &
  0.07735 &
  0.11444 &
  0.11484 &
  0.02881 &
  0.03992 &
  0.04492 &
  0.04995 &
  0.04997 \\
\textbf{SR} &
  0.0292 &
  0.05564 &
  0.08445 &
  0.11365 &
  0.13812 &
  0.0292 &
  0.04025 &
  0.04688 &
  0.05087 &
  0.0526 \\
\textbf{VSKNN} &
  0.17762 & 0.24098 & 0.27098 & 0.30098 & 0.32693 & 0.17762 & 0.20498 & 0.21194 & 0.21575 & 0.21757 \\
\textbf{SMF} &
  0.02111 &
  0.06238 &
  0.09381 &
  0.13743 &
  0.19184 &
  0.02111 &
  0.03877 &
  0.04583 &
  0.05182 &
  0.05558 \\
\textbf{Item2Vec} &
  0.0225 &
  0.0512 &
  0.06943 &
  0.09116 &
  0.12645 &
  0.0225 &
  0.03523 &
  0.03946 &
  0.04228 &
  0.04477 \\
\textbf{GRU4Rec+} &
  0.03043 &
  0.07266 &
  0.10127 &
  0.13488 &
  0.17302 &
  0.03043 &
  0.04859 &
  0.05511 &
  0.05957 &
  0.06231 \\
\textbf{NARM} &
  0.07881 &
  0.25793 &
  0.32406 &
  0.3654 &
  0.43536 &
  0.07881 &
  0.15887 &
  0.17624 &
  0.18141 &
  0.19044 \\
\textbf{STAMP} &
  0.05112 &
  0.12141 &
  0.15655 &
  0.20128 &
  0.24601 &
  0.05112 &
  0.07774 &
  0.08605 &
  0.0924 &
  0.0955 \\
\textbf{NextItNet} &
  0.04809 &
  0.09437 &
  0.11797 &
  0.1461 &
  0.1833 &
  0.04809 &
  0.06745 &
  0.07285 &
  0.07658 &
  0.07921 \\
\textbf{SRGNN} &
  0.1 &
  0.1375 &
  0.16667 &
  0.2 &
  0.24167 &
  0.1 &
  0.11736 &
  0.12361 &
  0.12811 &
  0.13088 \\
\textbf{CSRM} &
  0.12346 &
  0.22222 &
  0.2716 &
  0.30864 &
  0.41975 &
  0.12346 &
  0.17078 &
  0.18189 &
  0.18587 &
  0.19471 \\ \hline
\end{tabular}}
\label{tab:freq-low}
\end{table*}
