# Supplementary material for: Comprehensive Empirical Evaluation of Deep Learning Approaches for Session-based Recommendation in E-Commerce
Source: arXiv:2010.12540 source file (2020-10-17)
Supplement: Supplementary file 17 [file tab3.tex]

% Please add the following required packages to your document preamble:
% \usepackage{multirow}
% \usepackage[table,xcdraw]{xcolor}
% If you use beamer only pass "xcolor=table" option, i.e. \documentclass[xcolor=table]{beamer}
\begin{table*}[!h]
\centering
\caption{RQ3: training using short sessions of length \textless 5}
\resizebox{0.9\textwidth}{!}{\begin{tabular}{|c|ccccc|ccccc|}
\hline
\cellcolor[HTML]{333333}{\color[HTML]{FFFFFF} } &
  \multicolumn{5}{c|}{\textbf{HR@}} &
  \multicolumn{5}{c|}{\textbf{MRR@}} \\ \cline{2-11} 
\multirow{-2}{*}{\cellcolor[HTML]{333333}{\color[HTML]{FFFFFF} \textbf{RECSYS}}} &
  \textbf{1} &
  \textbf{3} &
  \textbf{5} &
  \textbf{10} &
  \textbf{20} &
  \textbf{1} &
  \textbf{3} &
  \textbf{5} &
  \textbf{10} &
  \textbf{20} \\ \hline
\textbf{S-POP} &
  0.03644 &
  0.09834 &
  0.12266 &
  0.1425 &
  0.15247 &
  0.03644 &
  0.06351 &
  0.06912 &
  0.07188 &
  0.07258 \\
\textbf{AR} &
  0.10322 &
  0.19791 &
  0.2579 &
  0.32011 &
  0.32024 &
  0.10322 &
  0.14393 &
  0.15759 &
  0.16643 &
  0.16643 \\
\textbf{SR} &
  0.10079 &
  0.1924 &
  0.24833 &
  0.32656 &
  0.39729 &
  0.10079 &
  0.14024 &
  0.15295 &
  0.16344 &
  0.16844 \\
\textbf{VSKNN} &
  0.06313 & 0.11626 & 0.14516 & 0.14809 & 0.15442 & 0.06409 & 0.07982 & 0.09956 & 0.09118 & 0.11871 \\
\textbf{SMF} &
  0.06544 &
  0.19569 &
  0.28226 &
  0.40961 &
  0.53788 &
  0.06544 &
  0.12155 &
  0.14128 &
  0.1583 &
  0.16724 \\
\textbf{Item2Vec} &
  0.03962 &
  0.0979 &
  0.13476 &
  0.2007 &
  0.28738 &
  0.03962 &
  0.06386 &
  0.07227 &
  0.08089 &
  0.08681 \\
\textbf{GRU4Rec+} &
  0.08691 &
  0.19155 &
  0.26486 &
  0.38632 &
  0.51757 &
  0.08691 &
  0.13123 &
  0.14788 &
  0.16395 &
  0.17306 \\
\textbf{NARM} &
  0.09403 &
  0.20763 &
  0.29068 &
  0.42206 &
  0.61657 &
  0.09403 &
  0.14288 &
  0.16194 &
  0.17947 &
  0.19115 \\
\textbf{STAMP} &
  0.11745 &
  0.23601 &
  0.30889 &
  0.41641 &
  0.53369 &
  0.11745 &
  0.1685 &
  0.185 &
  0.19937 &
  0.20748 \\
\textbf{NextItNet} &
  0.16085 &
  0.30699 &
  0.37462 &
  0.47358 &
  0.57299 &
  0.16085 &
  0.22333 &
  0.23878 &
  0.2521 &
  0.25896 \\
\textbf{SRGNN} &
  0.12021 &
  0.24474 &
  0.31917 &
  0.43593 &
  0.5498 &
  0.12021 &
  0.17381 &
  0.19072 &
  0.20628 &
  0.21416 \\
\textbf{CSRM} &
  0.12375 &
  0.25084 &
  0.33285 &
  0.46219 &
  0.58686 &
  0.12375 &
  0.17806 &
  0.19668 &
  0.21388 &
  0.22261 \\ \hline
\cellcolor[HTML]{333333}{\color[HTML]{FFFFFF} } &
  \multicolumn{5}{c|}{\textbf{HR@}} &
  \multicolumn{5}{c|}{\textbf{MRR@}} \\ \cline{2-11} 
\multirow{-2}{*}{\cellcolor[HTML]{333333}{\color[HTML]{FFFFFF} \textbf{CIKMCUP}}} &
  \textbf{1} &
  \textbf{3} &
  \textbf{5} &
  \textbf{10} &
  \textbf{20} &
  \textbf{1} &
  \textbf{3} &
  \textbf{5} &
  \textbf{10} &
  \textbf{20} \\ \hline
\textbf{S-POP} &
  0.0404 &
  0.10294 &
  0.12132 &
  0.13353 &
  0.13894 &
  0.0404 &
  0.06796 &
  0.07221 &
  0.07391 &
  0.07432 \\
\textbf{AR} &
  0.04354 &
  0.09489 &
  0.12547 &
  0.16247 &
  0.16272 &
  0.04354 &
  0.0654 &
  0.07238 &
  0.0776 &
  0.07761 \\
\textbf{SR} &
  0.03876 &
  0.0808 &
  0.10735 &
  0.13705 &
  0.16058 &
  0.03876 &
  0.05651 &
  0.06262 &
  0.06679 &
  0.06846 \\
\textbf{VSKNN} &
  0.05404 & 0.10119 & 0.12081 & 0.14387 & 0.15661 & 0.05404 & 0.07480 & 0.07924 & 0.08236 & 0.08328 \\
\textbf{SMF} &
  0.0354 &
  0.09003 &
  0.13326 &
  0.21406 &
  0.31589 &
  0.0354 &
  0.05823 &
  0.06803 &
  0.07861 &
  0.08565 \\
\textbf{Item2Vec} &
  0.01482 &
  0.03906 &
  0.05672 &
  0.09539 &
  0.14527 &
  0.01482 &
  0.02516 &
  0.02915 &
  0.03422 &
  0.0376 \\
\textbf{GRU4Rec+} &
  0.02219 &
  0.05442 &
  0.07762 &
  0.12966 &
  0.19687 &
  0.02219 &
  0.03611 &
  0.04137 &
  0.04823 &
  0.05284 \\
\textbf{NARM} &
  0.03687 &
  0.09389 &
  0.13304 &
  0.21731 &
  0.36243 &
  0.03687 &
  0.06168 &
  0.07081 &
  0.08194 &
  0.0904 \\
\textbf{STAMP} &
  0.02769 &
  0.06293 &
  0.09075 &
  0.14072 &
  0.20503 &
  0.02769 &
  0.04275 &
  0.04903 &
  0.05562 &
  0.06006 \\
\textbf{NextItNet} &
  0.03358 &
  0.06297 &
  0.08629 &
  0.12174 &
  0.16511 &
  0.03358 &
  0.04641 &
  0.05168 &
  0.0562 &
  0.05921 \\
\textbf{SRGNN} &
  0.04055 &
  0.09474 &
  0.13318 &
  0.20573 &
  0.29973 &
  0.04055 &
  0.06374 &
  0.07248 &
  0.08208 &
  0.08849 \\
\textbf{CSRM} &
  0.036 &
  0.09284 &
  0.13793 &
  0.21245 &
  0.31034 &
  0.036 &
  0.05993 &
  0.07025 &
  0.08009 &
  0.08679 \\ \hline
\cellcolor[HTML]{333333}{\color[HTML]{FFFFFF} } &
  \multicolumn{5}{c|}{\textbf{HR@}} &
  \multicolumn{5}{c|}{\textbf{MRR@}} \\ \cline{2-11} 
\multirow{-2}{*}{\cellcolor[HTML]{333333}{\color[HTML]{FFFFFF} \textbf{TMALL}}} &
  \textbf{1} &
  \textbf{3} &
  \textbf{5} &
  \textbf{10} &
  \textbf{20} &
  \textbf{1} &
  \textbf{3} &
  \textbf{5} &
  \textbf{10} &
  \textbf{20} \\ \hline
\textbf{S-POP} &
  0.04902 &
  0.11254 &
  0.14287 &
  0.17589 &
  0.19452 &
  0.04902 &
  0.07663 &
  0.08359 &
  0.0881 &
  0.08945 \\
\textbf{AR} &
  0.01448 &
  0.02716 &
  0.03466 &
  0.04259 &
  0.04288 &
  0.01448 &
  0.01995 &
  0.02166 &
  0.02278 &
  0.02281 \\
\textbf{SR} &
  0.01212 &
  0.02245 &
  0.02776 &
  0.0345 &
  0.04104 &
  0.01212 &
  0.01655 &
  0.01776 &
  0.01868 &
  0.01914 \\
\textbf{VSKNN} &
  0.02776 & 0.04697 & 0.05310 & 0.06036 & 0.06451 & 0.02776 & 0.03662 & 0.03762 & 0.03845 & 0.03877 \\
\textbf{SMF} &
  0.01292 &
  0.03135 &
  0.0449 &
  0.06516 &
  0.08647 &
  0.01292 &
  0.02067 &
  0.02375 &
  0.02646 &
  0.02793 \\
\textbf{Item2Vec} &
  0.00312 &
  0.0067 &
  0.00941 &
  0.01408 &
  0.0204 &
  0.00312 &
  0.00464 &
  0.00525 &
  0.00587 &
  0.0063 \\
\textbf{GRU4Rec+} &
  0.01296 &
  0.0286 &
  0.04041 &
  0.06028 &
  0.0833 &
  0.01296 &
  0.01963 &
  0.0223 &
  0.02491 &
  0.02649 \\
\textbf{NARM} &
  0.01904 &
  0.04279 &
  0.05725 &
  0.0836 &
  0.12595 &
  0.01904 &
  0.02944 &
  0.03277 &
  0.03627 &
  0.03875 \\
\textbf{STAMP} &
  0.01704 &
  0.03272 &
  0.04271 &
  0.05851 &
  0.07606 &
  0.01704 &
  0.02382 &
  0.02609 &
  0.02821 &
  0.02942 \\
\textbf{NextItNet} &
  0.02054 &
  0.03996 &
  0.05145 &
  0.06283 &
  0.07366 &
  0.02054 &
  0.02915 &
  0.03182 &
  0.03335 &
  0.03411 \\
\textbf{SRGNN} &
  0.0267 &
  0.05291 &
  0.06934 &
  0.09432 &
  0.12215 &
  0.0267 &
  0.03797 &
  0.04171 &
  0.04503 &
  0.04694 \\
\textbf{CSRM} &
  0.01616 &
  0.03583 &
  0.04689 &
  0.06469 &
  0.08438 &
  0.01616 &
  0.02464 &
  0.02716 &
  0.02954 &
  0.03089 \\ \hline
\cellcolor[HTML]{333333}{\color[HTML]{FFFFFF} } &
  \multicolumn{5}{c|}{\textbf{HR@}} &
  \multicolumn{5}{c|}{\textbf{MRR@}} \\ \cline{2-11} 
\multirow{-2}{*}{\cellcolor[HTML]{333333}{\color[HTML]{FFFFFF} \textbf{ROCKET}}} &
  \textbf{1} &
  \textbf{3} &
  \textbf{5} &
  \textbf{10} &
  \textbf{20} &
  \textbf{1} &
  \textbf{3} &
  \textbf{5} &
  \textbf{10} &
  \textbf{20} \\ \hline
\textbf{S-POP} &
  0.04243 &
  0.11138 &
  0.1253 &
  0.13657 &
  0.14453 &
  0.04243 &
  0.07396 &
  0.07723 &
  0.07878 &
  0.07936 \\
\textbf{AR} &
  0.06188 &
  0.11867 &
  0.15006 &
  0.17746 &
  0.17812 &
  0.06188 &
  0.086 &
  0.09321 &
  0.09713 &
  0.09716 \\
\textbf{SR} &
  0.05326 &
  0.10674 &
  0.12972 &
  0.15271 &
  0.16552 &
  0.05326 &
  0.07613 &
  0.08145 &
  0.08456 &
  0.0855 \\
\textbf{VSKNN} &
  0.10918 & 0.17144 & 0.18953 & 0.20948 & 0.21921 & 0.10918 & 0.13681 & 0.14098 & 0.14371 & 0.14441 \\
\textbf{SMF} &
  0.03934 &
  0.11425 &
  0.15691 &
  0.22055 &
  0.28022 &
  0.03934 &
  0.07101 &
  0.08085 &
  0.08928 &
  0.0934 \\
\textbf{Item2Vec} &
  0.02144 &
  0.04446 &
  0.05597 &
  0.08305 &
  0.11893 &
  0.02144 &
  0.03122 &
  0.03381 &
  0.03741 &
  0.0399 \\
\textbf{GRU4Rec+} &
  0.047 &
  0.09909 &
  0.13234 &
  0.17779 &
  0.23387 &
  0.047 &
  0.06854 &
  0.07596 &
  0.08208 &
  0.08595 \\
\textbf{NARM} &
  0.09487 &
  0.16408 &
  0.20912 &
  0.26023 &
  0.33391 &
  0.09487 &
  0.12397 &
  0.13406 &
  0.14099 &
  0.14533 \\
\textbf{STAMP} &
  0.05532 &
  0.10287 &
  0.13486 &
  0.17618 &
  0.21928 &
  0.05532 &
  0.07583 &
  0.08309 &
  0.08865 &
  0.09161 \\
\textbf{NextItNet} &
  0.07986 &
  0.14352 &
  0.18345 &
  0.22859 &
  0.2662 &
  0.07986 &
  0.10764 &
  0.11701 &
  0.12307 &
  0.12565 \\
\textbf{SRGNN} &
  0.08615 &
  0.15972 &
  0.19835 &
  0.24891 &
  0.29405 &
  0.08615 &
  0.11762 &
  0.12643 &
  0.13349 &
  0.13675 \\
\textbf{CSRM} &
  0.08741 &
  0.15946 &
  0.20338 &
  0.26071 &
  0.31474 &
  0.08741 &
  0.11879 &
  0.12872 &
  0.13619 &
  0.14002 \\ \hline
\end{tabular}}
\label{tab:train-short}
\end{table*}
