# Supplementary material for: Comprehensive Empirical Evaluation of Deep Learning Approaches for Session-based Recommendation in E-Commerce
Source: arXiv:2010.12540 source file (2020-10-17)
Supplement: Supplementary file 18 [file tab6.tex]

% Please add the following required packages to your document preamble:
% \usepackage{multirow}
% \usepackage[table,xcdraw]{xcolor}
% If you use beamer only pass "xcolor=table" option, i.e. \documentclass[xcolor=table]{beamer}
\begin{table*}[!h]
\centering
\caption{RQ3: testing using long Sessions of length \textgreater= 10}
\resizebox{0.9\textwidth}{!}{\begin{tabular}{|c|ccccc|ccccc|}
\hline
\cellcolor[HTML]{333333}{\color[HTML]{FFFFFF} } &
  \multicolumn{5}{c|}{\textbf{HR@}} &
  \multicolumn{5}{c|}{\textbf{MRR@}} \\ \cline{2-11} 
\multirow{-2}{*}{\cellcolor[HTML]{333333}{\color[HTML]{FFFFFF} \textbf{RECSYS}}} &
  \textbf{1} &
  \textbf{3} &
  \textbf{5} &
  \textbf{10} &
  \textbf{20} &
  \textbf{1} &
  \textbf{3} &
  \textbf{5} &
  \textbf{10} &
  \textbf{20} \\ \hline
\textbf{S-POP} &
  0.04263 &
  0.12035 &
  0.1636 &
  0.21165 &
  0.23679 &
  0.04263 &
  0.07605 &
  0.08591 &
  0.09254 &
  0.09435 \\
\textbf{AR} &
  0.07969 &
  0.1648 &
  0.21566 &
  0.26714 &
  0.26875 &
  0.07969 &
  0.11593 &
  0.12749 &
  0.13491 &
  0.13503 \\
\textbf{SR} &
  0.08152 &
  0.16662 &
  0.21935 &
  0.30462 &
  0.39087 &
  0.08152 &
  0.1185 &
  0.13043 &
  0.14179 &
  0.14784 \\
\textbf{VSKNN} &
  0.07712 & 0.18216 & 0.23870 & 0.32259 & 0.41836 & 0.07712 & 0.12267 & 0.13559 & 0.14673 & 0.15340 \\
\textbf{SMF} &
  0.06486 &
  0.16751 &
  0.24241 &
  0.37656 &
  0.50565 &
  0.06486 &
  0.1083 &
  0.12526 &
  0.14312 &
  0.15212 \\
\textbf{Item2Vec} &
  0.04255 &
  0.08756 &
  0.11741 &
  0.1703 &
  0.24415 &
  0.04255 &
  0.06197 &
  0.06868 &
  0.07569 &
  0.08078 \\
\textbf{GRU4Rec+} &
  0.05066 &
  0.13116 &
  0.19353 &
  0.30392 &
  0.43304 &
  0.05066 &
  0.08464 &
  0.09878 &
  0.11342 &
  0.12234 \\
\textbf{NARM} &
  0.09528 &
  0.25597 &
  0.36131 &
  0.51359 &
  0.71232 &
  0.09528 &
  0.16319 &
  0.18721 &
  0.20846 &
  0.2202 \\
\textbf{STAMP} &
  0.09363 &
  0.19914 &
  0.27058 &
  0.39681 &
  0.54189 &
  0.09363 &
  0.13849 &
  0.1547 &
  0.17134 &
  0.18141 \\
\textbf{NextItNet} &
  0.0952 &
  0.22093 &
  0.2936 &
  0.4048 &
  0.53634 &
  0.0952 &
  0.14959 &
  0.16627 &
  0.18104 &
  0.19009 \\
\textbf{SRGNN} &
  0.09422 &
  0.20721 &
  0.28337 &
  0.41675 &
  0.55934 &
  0.09422 &
  0.14246 &
  0.15973 &
  0.17736 &
  0.18731 \\
\textbf{CSRM} &
  0.13927 &
  0.29161 &
  0.37752 &
  0.51519 &
  0.64915 &
  0.13927 &
  0.2053 &
  0.22471 &
  0.24303 &
  0.25241 \\ \hline
\cellcolor[HTML]{333333}{\color[HTML]{FFFFFF} } &
  \multicolumn{5}{c|}{\textbf{HR@}} &
  \multicolumn{5}{c|}{\textbf{MRR@}} \\ \cline{2-11} 
\multirow{-2}{*}{\cellcolor[HTML]{333333}{\color[HTML]{FFFFFF} \textbf{CIKMCUP}}} &
  \textbf{1} &
  \textbf{3} &
  \textbf{5} &
  \textbf{10} &
  \textbf{20} &
  \textbf{1} &
  \textbf{3} &
  \textbf{5} &
  \textbf{10} &
  \textbf{20} \\ \hline
\textbf{S-POP} &
  0.04248 &
  0.11997 &
  0.15337 &
  0.18515 &
  0.19293 &
  0.04248 &
  0.07609 &
  0.08378 &
  0.08833 &
  0.08888 \\
\textbf{AR} &
  0.03437 &
  0.07847 &
  0.11187 &
  0.15694 &
  0.15694 &
  0.03437 &
  0.05318 &
  0.06085 &
  0.06724 &
  0.06724 \\
\textbf{SR} &
  0.03372 &
  0.07263 &
  0.10409 &
  0.15013 &
  0.19747 &
  0.03372 &
  0.05042 &
  0.05749 &
  0.06376 &
  0.06711 \\
\textbf{VSKNN} &
  0.05352 & 0.12307 & 0.16480 & 0.22770 & 0.30360 & 0.05352 & 0.08280 & 0.09222 & 0.10040 & 0.10568 \\
\textbf{SMF} &
  0.03293 &
  0.0864 &
  0.13466 &
  0.22302 &
  0.33942 &
  0.03293 &
  0.05559 &
  0.06645 &
  0.07783 &
  0.0859 \\
\textbf{Item2Vec} &
  0.01509 &
  0.03412 &
  0.04921 &
  0.08005 &
  0.13255 &
  0.01509 &
  0.02335 &
  0.02681 &
  0.03085 &
  0.03442 \\
\textbf{GRU4Rec+} &
  0.02935 &
  0.06581 &
  0.09677 &
  0.16742 &
  0.24452 &
  0.02935 &
  0.04446 &
  0.05154 &
  0.06063 &
  0.06598 \\
\textbf{NARM} &
  0.03615 &
  0.09018 &
  0.12893 &
  0.22581 &
  0.43369 &
  0.03615 &
  0.05866 &
  0.06741 &
  0.07985 &
  0.09186 \\
\textbf{STAMP} &
  0.03243 &
  0.08625 &
  0.1297 &
  0.20169 &
  0.31258 &
  0.03243 &
  0.05529 &
  0.06506 &
  0.07452 &
  0.08207 \\
\textbf{NextItNet} &
  0.02083 &
  0.05208 &
  0.07292 &
  0.12847 &
  0.16319 &
  0.02083 &
  0.03299 &
  0.03819 &
  0.04533 &
  0.04743 \\
\textbf{SRGNN} &
  0.0425 &
  0.10281 &
  0.15094 &
  0.24813 &
  0.35938 &
  0.0425 &
  0.06786 &
  0.07886 &
  0.09179 &
  0.09949 \\
\textbf{CSRM} &
  0.03948 &
  0.10016 &
  0.14617 &
  0.24274 &
  0.35628 &
  0.03948 &
  0.06471 &
  0.07515 &
  0.08791 &
  0.09561 \\ \hline
\cellcolor[HTML]{333333}{\color[HTML]{FFFFFF} } &
  \multicolumn{5}{c|}{\textbf{HR@}} &
  \multicolumn{5}{c|}{\textbf{MRR@}} \\ \cline{2-11} 
\multirow{-2}{*}{\cellcolor[HTML]{333333}{\color[HTML]{FFFFFF} \textbf{TMALL}}} &
  \textbf{1} &
  \textbf{3} &
  \textbf{5} &
  \textbf{10} &
  \textbf{20} &
  \textbf{1} &
  \textbf{3} &
  \textbf{5} &
  \textbf{10} &
  \textbf{20} \\ \hline
\textbf{S-POP} &
  0.05096 &
  0.11438 &
  0.15166 &
  0.19137 &
  0.21527 &
  0.05096 &
  0.05096 &
  0.05096 &
  0.05096 &
  0.05096 \\
\textbf{AR} &
  0.0088 &
  0.01936 &
  0.02613 &
  0.03679 &
  0.03732 &
  0.0088 &
  0.01332 &
  0.01485 &
  0.01632 &
  0.01636 \\
\textbf{SR} &
  0.00793 &
  0.0161 &
  0.02145 &
  0.03004 &
  0.03951 &
  0.00793 &
  0.0114 &
  0.01263 &
  0.01375 &
  0.01441 \\
\textbf{VSKNN} &
  0.02861 & 0.05038 & 0.06213 & 0.08140 & 0.10225 & 0.04902 & 0.04353 & 0.04496 & 0.03607 & 0.05283 \\
\textbf{SMF} &
  0.01275 &
  0.03361 &
  0.04912 &
  0.0745 &
  0.10797 &
  0.01275 &
  0.0216 &
  0.02514 &
  0.02848 &
  0.03077 \\
\textbf{Item2Vec} &
  0.00168 &
  0.00418 &
  0.00604 &
  0.01001 &
  0.01532 &
  0.00168 &
  0.00274 &
  0.00316 &
  0.00367 &
  0.00403 \\
\textbf{GRU4Rec+} &
  0.01344 &
  0.03275 &
  0.04445 &
  0.06461 &
  0.08464 &
  0.01344 &
  0.02159 &
  0.02423 &
  0.02692 &
  0.02829 \\
\textbf{NARM} &
  0.02161 &
  0.04695 &
  0.06368 &
  0.09147 &
  0.14372 &
  0.02161 &
  0.03247 &
  0.03628 &
  0.03994 &
  0.04295 \\
\textbf{STAMP} &
  0.02536 &
  0.05332 &
  0.07018 &
  0.09731 &
  0.12822 &
  0.02536 &
  0.03741 &
  0.04122 &
  0.04483 &
  0.04698 \\
\textbf{NextItNet} &
  0.00293 &
  0.00944 &
  0.01139 &
  0.0153 &
  0.02181 &
  0.00293 &
  0.00581 &
  0.00624 &
  0.00679 &
  0.00723 \\
\textbf{SRGNN} &
  0.02273 &
  0.04555 &
  0.05887 &
  0.0817 &
  0.1072 &
  0.02273 &
  0.03249 &
  0.03554 &
  0.03857 &
  0.04033 \\
\textbf{CSRM} &
  0.01536 &
  0.03333 &
  0.04497 &
  0.06644 &
  0.09052 &
  0.01536 &
  0.02303 &
  0.02565 &
  0.02849 &
  0.03015 \\ \hline
\cellcolor[HTML]{333333}{\color[HTML]{FFFFFF} } &
  \multicolumn{5}{c|}{\textbf{HR@}} &
  \multicolumn{5}{c|}{\textbf{MRR@}} \\ \cline{2-11} 
\multirow{-2}{*}{\cellcolor[HTML]{333333}{\color[HTML]{FFFFFF} \textbf{ROCKET}}} &
  \textbf{1} &
  \textbf{3} &
  \textbf{5} &
  \textbf{10} &
  \textbf{20} &
  \textbf{1} &
  \textbf{3} &
  \textbf{5} &
  \textbf{10} &
  \textbf{20} \\ \hline
\textbf{S-POP} &
  0.03081 &
  0.11386 &
  0.13865 &
  0.16611 &
  0.1795 &
  0.03081 &
  0.0662 &
  0.07192 &
  0.07568 &
  0.07663 \\
\textbf{AR} &
  0.01808 &
  0.04287 &
  0.05492 &
  0.06631 &
  0.06698 &
  0.01808 &
  0.02858 &
  0.03132 &
  0.03299 &
  0.03304 \\
\textbf{SR} &
  0.0221 &
  0.03818 &
  0.0422 &
  0.0643 &
  0.08038 &
  0.0221 &
  0.02858 &
  0.02945 &
  0.03237 &
  0.03351 \\
\textbf{VSKNN} &
  0.06990 & 0.13795 & 0.16186 & 0.20785 & 0.24954 & 0.06990 & 0.10035 & 0.10590 & 0.11195 & 0.11469 \\
\textbf{SMF} &
  0.02009 &
  0.04622 &
  0.07033 &
  0.11253 &
  0.15673 &
  0.02009 &
  0.0307 &
  0.03639 &
  0.04199 &
  0.04506 \\
\textbf{Item2Vec} &
  0.00955 &
  0.02729 &
  0.03342 &
  0.05866 &
  0.07776 &
  0.00955 &
  0.01705 &
  0.01849 &
  0.02181 &
  0.02314 \\
\textbf{GRU4Rec+} &
  0.01996 &
  0.04391 &
  0.05988 &
  0.08649 &
  0.11244 &
  0.01996 &
  0.03027 &
  0.03383 &
  0.03726 &
  0.03909 \\
\textbf{NARM} &
  0.03345 &
  0.07126 &
  0.09484 &
  0.13916 &
  0.23255 &
  0.03345 &
  0.05204 &
  0.0572 &
  0.06303 &
  0.06863 \\
\textbf{STAMP} &
  0.02143 &
  0.04555 &
  0.06162 &
  0.09779 &
  0.13664 &
  0.02143 &
  0.03204 &
  0.03569 &
  0.04061 &
  0.04329 \\
\textbf{NextItNet} &
  0.01042 &
  0.03125 &
  0.05208 &
  0.07292 &
  0.09375 &
  0.01042 &
  0.0191 &
  0.02378 &
  0.02624 &
  0.02791 \\
\textbf{SRGNN} &
  0.02669 &
  0.05924 &
  0.08203 &
  0.11198 &
  0.14323 &
  0.02669 &
  0.04069 &
  0.0458 &
  0.04972 &
  0.05193 \\
\textbf{CSRM} &
  0.03562 &
  0.06452 &
  0.08871 &
  0.12567 &
  0.17675 &
  0.03562 &
  0.04805 &
  0.05343 &
  0.05815 &
  0.06169 \\ \hline
\end{tabular}}
\label{tab:test-long}
\end{table*}
