# Supplementary material for: Comprehensive Empirical Evaluation of Deep Learning Approaches for Session-based Recommendation in E-Commerce
Source: arXiv:2010.12540 source file (2020-10-17)
Supplement: Supplementary file 19 [file tab7.tex]

% Please add the following required packages to your document preamble:
% \usepackage{multirow}
% \usepackage[table,xcdraw]{xcolor}
% If you use beamer only pass "xcolor=table" option, i.e. \documentclass[xcolor=table]{beamer}
\begin{table*}[!h]
\centering
\caption{RQ4: training using the most recent 5(10) days in the training set for RECSYS, CIKMCUP, TMall, and (ROCKET) datasets.}
\resizebox{0.9\textwidth}{!}{\begin{tabular}{|c|ccccc|ccccc|}
\hline
\cellcolor[HTML]{333333}{\color[HTML]{FFFFFF} } &
  \multicolumn{5}{c|}{\textbf{HR@}} &
  \multicolumn{5}{c|}{\textbf{MRR@}} \\ \cline{2-11} 
\multirow{-2}{*}{\cellcolor[HTML]{333333}{\color[HTML]{FFFFFF} \textbf{RECSYS}}} &
  \textbf{1} &
  \textbf{3} &
  \textbf{5} &
  \textbf{10} &
  \textbf{20} &
  \textbf{1} &
  \textbf{3} &
  \textbf{5} &
  \textbf{10} &
  \textbf{20} \\ \hline
\textbf{S-POP} &
  0.0366 &
  0.10092 &
  0.12481 &
  0.14821 &
  0.16091 &
  0.0366 &
  0.06483 &
  0.07032 &
  0.07356 &
  0.07446 \\
\textbf{AR} &
  0.11837 &
  0.22948 &
  0.29245 &
  0.36044 &
  0.36239 &
  0.11837 &
  0.16629 &
  0.1806 &
  0.19033 &
  0.19045 \\
\textbf{SR} &
  0.1201 &
  0.23139 &
  0.29712 &
  0.38944 &
  0.48072 &
  0.1201 &
  0.16816 &
  0.18315 &
  0.19548 &
  0.20189 \\
\textbf{VSKNN} &
  0.10597 & 0.18932 & 0.25384 & 0.31684 & 0.39317 & 0.09974 & 0.14418 & 0.15025 & 0.16697 & 0.16280 \\
\textbf{SMF} &
  0.06946 &
  0.20252 &
  0.28946 &
  0.42745 &
  0.55893 &
  0.06946 &
  0.12603 &
  0.14583 &
  0.16431 &
  0.1735 \\
\textbf{Item2Vec} &
  0.07512 &
  0.14356 &
  0.18745 &
  0.26069 &
  0.34475 &
  0.07512 &
  0.10469 &
  0.11464 &
  0.12429 &
  0.13008 \\
\textbf{GRU4Rec+} &
  0.08493 &
  0.19279 &
  0.26846 &
  0.39479 &
  0.52594 &
  0.08493 &
  0.13108 &
  0.14821 &
  0.16503 &
  0.17418 \\
\textbf{NARM} &
  0.11457 &
  0.28118 &
  0.37792 &
  0.52823 &
  0.70543 &
  0.11457 &
  0.18665 &
  0.20859 &
  0.22869 &
  0.23957 \\
\textbf{STAMP} &
  0.13265 &
  0.2726 &
  0.35214 &
  0.47471 &
  0.60039 &
  0.13265 &
  0.19287 &
  0.21096 &
  0.22715 &
  0.23595 \\
\textbf{NextItNet} &
  0.18508 &
  0.34337 &
  0.4224 &
  0.53057 &
  0.62764 &
  0.18508 &
  0.2537 &
  0.27186 &
  0.28633 &
  0.29313 \\
\textbf{SRGNN} &
  0.1381 &
  0.28465 &
  0.36947 &
  0.49148 &
  0.61673 &
  0.1381 &
  0.20088 &
  0.22015 &
  0.2364 &
  0.24514 \\
\textbf{CSRM} &
  0.16837 &
  0.32844 &
  0.41451 &
  0.54903 &
  0.67152 &
  0.16837 &
  0.23758 &
  0.25714 &
  0.27505 &
  0.28364 \\ \hline
\cellcolor[HTML]{333333}{\color[HTML]{FFFFFF} } &
  \multicolumn{5}{c|}{\textbf{HR@}} &
  \multicolumn{5}{c|}{\textbf{MRR@}} \\ \cline{2-11} 
\multirow{-2}{*}{\cellcolor[HTML]{333333}{\color[HTML]{FFFFFF} \textbf{CIKMCUP}}} &
  \textbf{1} &
  \textbf{3} &
  \textbf{5} &
  \textbf{10} &
  \textbf{20} &
  \textbf{1} &
  \textbf{3} &
  \textbf{5} &
  \textbf{10} &
  \textbf{20} \\ \hline
\textbf{S-POP} &
  0.04027 &
  0.10372 &
  0.12274 &
  0.13718 &
  0.14385 &
  0.04027 &
  0.06836 &
  0.07284 &
  0.07496 &
  0.07543 \\
\textbf{AR} &
  0.04388 &
  0.09761 &
  0.13427 &
  0.18273 &
  0.1855 &
  0.04388 &
  0.06711 &
  0.07544 &
  0.08226 &
  0.08244 \\
\textbf{SR} &
  0.03791 &
  0.08067 &
  0.10969 &
  0.15996 &
  0.20619 &
  0.03791 &
  0.05651 &
  0.06309 &
  0.06988 &
  0.07315 \\
\textbf{VSKNN} &
  0.05962 & 0.12075 & 0.15665 & 0.20823 & 0.26070 & 0.05962 & 0.08619 & 0.09448 & 0.10134 & 0.10505 \\
\textbf{SMF} &
  0.03564 &
  0.09552 &
  0.14018 &
  0.21992 &
  0.33207 &
  0.03564 &
  0.061 &
  0.0712 &
  0.08176 &
  0.08947 \\
\textbf{Item2Vec} &
  0.02132 &
  0.04928 &
  0.07201 &
  0.1172 &
  0.17862 &
  0.02132 &
  0.03316 &
  0.03823 &
  0.0442 &
  0.04835 \\
\textbf{GRU4Rec+} &
  0.02354 &
  0.05782 &
  0.08287 &
  0.13326 &
  0.19287 &
  0.02354 &
  0.03816 &
  0.04384 &
  0.05047 &
  0.05458 \\
\textbf{NARM} &
  0.0461 &
  0.1118 &
  0.15625 &
  0.2394 &
  0.39249 &
  0.0461 &
  0.07413 &
  0.08421 &
  0.09539 &
  0.10442 \\
\textbf{STAMP} &
  0.02958 &
  0.0736 &
  0.10582 &
  0.16387 &
  0.23788 &
  0.02958 &
  0.04793 &
  0.05519 &
  0.06285 &
  0.06794 \\
\textbf{NextItNet} &
  0.01736 &
  0.03522 &
  0.04861 &
  0.0744 &
  0.10466 &
  0.01736 &
  0.02472 &
  0.02762 &
  0.03091 &
  0.03288 \\
\textbf{SRGNN} &
  0.04304 &
  0.10855 &
  0.15666 &
  0.23643 &
  0.33703 &
  0.04304 &
  0.07063 &
  0.08158 &
  0.09226 &
  0.09922 \\
\textbf{CSRM} &
  0.04271 &
  0.10351 &
  0.14608 &
  0.22371 &
  0.31706 &
  0.04271 &
  0.06817 &
  0.07785 &
  0.0882 &
  0.09458 \\ \hline
\cellcolor[HTML]{333333}{\color[HTML]{FFFFFF} } &
  \multicolumn{5}{c|}{\textbf{HR@}} &
  \multicolumn{5}{c|}{\textbf{MRR@}} \\ \cline{2-11} 
\multirow{-2}{*}{\cellcolor[HTML]{333333}{\color[HTML]{FFFFFF} \textbf{TMALL}}} &
  \textbf{1} &
  \textbf{3} &
  \textbf{5} &
  \textbf{10} &
  \textbf{20} &
  \textbf{1} &
  \textbf{3} &
  \textbf{5} &
  \textbf{10} &
  \textbf{20} \\ \hline
\textbf{S-POP} &
  0.04542 &
  0.1047 &
  0.13305 &
  0.1655 &
  0.18606 &
  0.04542 &
  0.07108 &
  0.07756 &
  0.08198 &
  0.08345 \\
\textbf{AR} &
  0.0141 &
  0.02999 &
  0.03989 &
  0.05402 &
  0.05476 &
  0.0141 &
  0.02092 &
  0.02317 &
  0.02512 &
  0.02517 \\
\textbf{SR} &
  0.01357 &
  0.02859 &
  0.03784 &
  0.05104 &
  0.06524 &
  0.01357 &
  0.02004 &
  0.02214 &
  0.02391 &
  0.02489 \\
\textbf{VSKNN} &
  0.02901 & 0.04266 & 0.06215 & 0.06208 & 0.08511 & 0.02256 & 0.03568 & 0.03237 & 0.04793 & 0.04223 \\
\textbf{SMF} &
  0.0157 &
  0.04112 &
  0.05925 &
  0.08783 &
  0.12225 &
  0.0157 &
  0.02652 &
  0.03063 &
  0.0344 &
  0.03675 \\
\textbf{Item2Vec} &
  0.0022 &
  0.00485 &
  0.00675 &
  0.01161 &
  0.01818 &
  0.0022 &
  0.00329 &
  0.00372 &
  0.00436 &
  0.00481 \\
\textbf{GRU4Rec+} &
  0.02411 &
  0.0549 &
  0.07389 &
  0.10368 &
  0.13622 &
  0.02411 &
  0.03737 &
  0.0417 &
  0.04568 &
  0.04794 \\
\textbf{NARM} &
  0.04043 &
  0.08946 &
  0.11755 &
  0.16023 &
  0.24241 &
  0.04043 &
  0.06174 &
  0.06809 &
  0.07376 &
  0.0787 \\
\textbf{STAMP} &
  0.03542 &
  0.07169 &
  0.09382 &
  0.12706 &
  0.16389 &
  0.03542 &
  0.05106 &
  0.05612 &
  0.06053 &
  0.06308 \\
\textbf{NextItNet} &
  0.02441 &
  0.04742 &
  0.05903 &
  0.0778 &
  0.09907 &
  0.02441 &
  0.03456 &
  0.03717 &
  0.03962 &
  0.04109 \\
\textbf{SRGNN} &
  0.03734 &
  0.07508 &
  0.09736 &
  0.131 &
  0.16891 &
  0.03734 &
  0.05356 &
  0.05864 &
  0.0631 &
  0.06571 \\
\textbf{CSRM} &
  0.03117 &
  0.06737 &
  0.08954 &
  0.1254 &
  0.16772 &
  0.03117 &
  0.04679 &
  0.05184 &
  0.05657 &
  0.0595 \\ \hline
\cellcolor[HTML]{333333}{\color[HTML]{FFFFFF} } &
  \multicolumn{5}{c|}{\textbf{HR@}} &
  \multicolumn{5}{c|}{\textbf{MRR@}} \\ \cline{2-11} 
\multirow{-2}{*}{\cellcolor[HTML]{333333}{\color[HTML]{FFFFFF} \textbf{ROCKET}}} &
  \textbf{1} &
  \textbf{3} &
  \textbf{5} &
  \textbf{10} &
  \textbf{20} &
  \textbf{1} &
  \textbf{3} &
  \textbf{5} &
  \textbf{10} &
  \textbf{20} \\ \hline
\textbf{S-POP} &
  0.03795 &
  0.11177 &
  0.12907 &
  0.14223 &
  0.15256 &
  0.03795 &
  0.07094 &
  0.07498 &
  0.07673 &
  0.07743 \\
\textbf{AR} &
  0.05498 &
  0.10867 &
  0.13345 &
  0.16314 &
  0.1634 &
  0.05498 &
  0.0783 &
  0.0839 &
  0.08802 &
  0.08803 \\
\textbf{SR} &
  0.04595 &
  0.09732 &
  0.12158 &
  0.14481 &
  0.16701 &
  0.04595 &
  0.06789 &
  0.07349 &
  0.07679 &
  0.07837 \\
\textbf{VSKNN} &
  0.12808 & 0.20525 & 0.22910 & 0.26238 & 0.28863 & 0.12808 & 0.16249 & 0.16797 & 0.17249 & 0.17432 \\
\textbf{SMF} &
  0.04337 &
  0.10945 &
  0.14972 &
  0.20547 &
  0.27336 &
  0.04337 &
  0.07124 &
  0.08041 &
  0.08772 &
  0.09249 \\
\textbf{Item2Vec} &
  0.02535 &
  0.05572 &
  0.07314 &
  0.09929 &
  0.12965 &
  0.02535 &
  0.03829 &
  0.04217 &
  0.04563 &
  0.04766 \\
\textbf{GRU4Rec+} &
  0.03957 &
  0.07991 &
  0.10509 &
  0.14106 &
  0.17009 &
  0.03957 &
  0.05695 &
  0.06275 &
  0.06752 &
  0.06952 \\
\textbf{NARM} &
  0.07335 &
  0.14935 &
  0.17745 &
  0.23272 &
  0.30072 &
  0.07335 &
  0.10652 &
  0.11323 &
  0.1205 &
  0.12432 \\
\textbf{STAMP} &
  0.04675 &
  0.09481 &
  0.13195 &
  0.17143 &
  0.21351 &
  0.04675 &
  0.0671 &
  0.07561 &
  0.08091 &
  0.08383 \\
\textbf{NextItNet} &
  0.03338 &
  0.05114 &
  0.06747 &
  0.08381 &
  0.11151 &
  0.03338 &
  0.04096 &
  0.0444 &
  0.04663 &
  0.04858 \\
\textbf{SRGNN} &
  0.04965 &
  0.10988 &
  0.14138 &
  0.1812 &
  0.22077 &
  0.04965 &
  0.07548 &
  0.08261 &
  0.08796 &
  0.09074 \\
\textbf{CSRM} &
  0.06492 &
  0.1319 &
  0.16782 &
  0.2253 &
  0.27123 &
  0.06492 &
  0.09375 &
  0.10206 &
  0.10963 &
  0.11282 \\ \hline
\end{tabular}}
\label{tab:recency-recent}
\end{table*}
