# Supplementary material for: Comprehensive Empirical Evaluation of Deep Learning Approaches for Session-based Recommendation in E-Commerce
Source: arXiv:2010.12540 source file (2020-10-17)
Supplement: Supplementary file 20 [file tab8.tex]

% Please add the following required packages to your document preamble:
% \usepackage{multirow}
% \usepackage[table,xcdraw]{xcolor}
% If you use beamer only pass "xcolor=table" option, i.e. \documentclass[xcolor=table]{beamer}
\begin{table*}[!h]
\centering
\caption{RQ4: training using eldest 5(10) days in the training set for RECSYS, CIKMCUP, TMall, and (ROCKET) datasets.}
\resizebox{0.9\textwidth}{!}{\begin{tabular}{|c|ccccc|ccccc|}
\hline
\cellcolor[HTML]{333333}{\color[HTML]{FFFFFF} } &
  \multicolumn{5}{c|}{\textbf{HR@}} &
  \multicolumn{5}{c|}{\textbf{MRR@}} \\ \cline{2-11} 
\multirow{-2}{*}{\cellcolor[HTML]{333333}{\color[HTML]{FFFFFF} \textbf{RECSYS}}} &
  \textbf{1} &
  \textbf{3} &
  \textbf{5} &
  \textbf{10} &
  \textbf{20} &
  \textbf{1} &
  \textbf{3} &
  \textbf{5} &
  \textbf{10} &
  \textbf{20} \\ \hline
\textbf{S-POP} &
  0.0505 &
  0.1199 &
  0.13773 &
  0.14682 &
  0.14988 &
  0.0505 &
  0.08192 &
  0.08607 &
  0.08737 &
  0.0876 \\
\textbf{AR} &
  0.064 &
  0.13746 &
  0.1776 &
  0.21946 &
  0.21964 &
  0.064 &
  0.09534 &
  0.10443 &
  0.11026 &
  0.11027 \\
\textbf{SR} &
  0.06148 &
  0.13989 &
  0.18192 &
  0.22972 &
  0.29382 &
  0.06148 &
  0.09501 &
  0.10445 &
  0.11088 &
  0.11546 \\
\textbf{VSKNN} &
  0.11214 & 0.15943 & 0.18167 & 0.21227 & 0.23055 & 0.11485 & 0.12550 & 0.13974 & 0.14178 & 0.13535 \\
\textbf{SMF} &
  0.03556 &
  0.1399 &
  0.21291 &
  0.31662 &
  0.40763 &
  0.03556 &
  0.07916 &
  0.0957 &
  0.10959 &
  0.11595 \\
\textbf{Item2Vec} &
  0.02606 &
  0.06934 &
  0.09194 &
  0.14861 &
  0.21932 &
  0.02606 &
  0.045 &
  0.05003 &
  0.0576 &
  0.06254 \\
\textbf{GRU4Rec+} &
  0.05481 &
  0.1434 &
  0.21387 &
  0.31362 &
  0.39957 &
  0.05481 &
  0.092 &
  0.10796 &
  0.12141 &
  0.12738 \\
\textbf{NARM} &
  0.07121 &
  0.1895 &
  0.25972 &
  0.34935 &
  0.50721 &
  0.07121 &
  0.12244 &
  0.14024 &
  0.1533 &
  0.1628 \\
\textbf{STAMP} &
  0.0827 &
  0.17982 &
  0.23059 &
  0.32164 &
  0.41821 &
  0.0827 &
  0.1235 &
  0.135 &
  0.14688 &
  0.15358 \\
\textbf{NextItNet} &
  0.08304 &
  0.17634 &
  0.24509 &
  0.31942 &
  0.39621 &
  0.08304 &
  0.12374 &
  0.13956 &
  0.14944 &
  0.15468 \\
\textbf{SRGNN} &
  0.08648 &
  0.19352 &
  0.25332 &
  0.33037 &
  0.4296 &
  0.08648 &
  0.13199 &
  0.14564 &
  0.1559 &
  0.16272 \\
\textbf{CSRM} &
  0.09126 &
  0.19937 &
  0.2589 &
  0.36004 &
  0.46153 &
  0.09126 &
  0.13706 &
  0.15053 &
  0.16381 &
  0.17083 \\ \hline
\cellcolor[HTML]{333333}{\color[HTML]{FFFFFF} } &
  \multicolumn{5}{c|}{\textbf{HR@}} &
  \multicolumn{5}{c|}{\textbf{MRR@}} \\ \cline{2-11} 
\multirow{-2}{*}{\cellcolor[HTML]{333333}{\color[HTML]{FFFFFF} \textbf{CIKMCUP}}} &
  \textbf{1} &
  \textbf{3} &
  \textbf{5} &
  \textbf{10} &
  \textbf{20} &
  \textbf{1} &
  \textbf{3} &
  \textbf{5} &
  \textbf{10} &
  \textbf{20} \\ \hline
\textbf{S-POP} &
  0.03899 &
  0.10664 &
  0.12135 &
  0.1291 &
  0.13375 &
  0.03899 &
  0.06877 &
  0.07215 &
  0.07328 &
  0.07361 \\
\textbf{AR} &
  0.03847 &
  0.08572 &
  0.11955 &
  0.16266 &
  0.16266 &
  0.03847 &
  0.05908 &
  0.06687 &
  0.0729 &
  0.0729 \\
\textbf{SR} &
  0.03227 &
  0.06997 &
  0.09605 &
  0.13168 &
  0.1606 &
  0.03227 &
  0.04798 &
  0.05371 &
  0.05858 &
  0.06065 \\
\textbf{VSKNN} &
  0.08275 & 0.14899 & 0.19082 & 0.25096 & 0.29279 & 0.08275 & 0.11135 & 0.12078 & 0.12888 & 0.13179 \\
\textbf{SMF} &
  0.03894 &
  0.09096 &
  0.12912 &
  0.20125 &
  0.28698 &
  0.03894 &
  0.0602 &
  0.06884 &
  0.07839 &
  0.08434 \\
\textbf{Item2Vec} &
  0.0202 &
  0.04853 &
  0.07004 &
  0.10913 &
  0.15923 &
  0.0202 &
  0.03231 &
  0.03716 &
  0.0423 &
  0.04578 \\
\textbf{GRU4Rec+} &
  0.0244 &
  0.05403 &
  0.07644 &
  0.11753 &
  0.17007 &
  0.0244 &
  0.03714 &
  0.04222 &
  0.04761 &
  0.05114 \\
\textbf{NARM} &
  0.03617 &
  0.09168 &
  0.13568 &
  0.20776 &
  0.34333 &
  0.03617 &
  0.06008 &
  0.07001 &
  0.07935 &
  0.08721 \\
\textbf{STAMP} &
  0.02608 &
  0.06507 &
  0.09011 &
  0.14278 &
  0.20475 &
  0.02608 &
  0.04247 &
  0.04826 &
  0.05513 &
  0.05942 \\
\textbf{NextItNet} &
  0.01116 &
  0.01339 &
  0.02009 &
  0.03199 &
  0.05357 &
  0.01116 &
  0.01203 &
  0.01363 &
  0.01528 &
  0.01678 \\
\textbf{SRGNN} &
  0.03478 &
  0.0935 &
  0.14037 &
  0.2001 &
  0.27646 &
  0.03478 &
  0.05994 &
  0.07055 &
  0.07844 &
  0.08378 \\
\textbf{CSRM} &
  0.0321 &
  0.07766 &
  0.11261 &
  0.18379 &
  0.26171 &
  0.0321 &
  0.05156 &
  0.05953 &
  0.06893 &
  0.07435 \\ \hline
\cellcolor[HTML]{333333}{\color[HTML]{FFFFFF} } &
  \multicolumn{5}{c|}{\textbf{HR@}} &
  \multicolumn{5}{c|}{\textbf{MRR@}} \\ \cline{2-11} 
\multirow{-2}{*}{\cellcolor[HTML]{333333}{\color[HTML]{FFFFFF} \textbf{TMALL}}} &
  \textbf{1} &
  \textbf{3} &
  \textbf{5} &
  \textbf{10} &
  \textbf{20} &
  \textbf{1} &
  \textbf{3} &
  \textbf{5} &
  \textbf{10} &
  \textbf{20} \\ \hline
\textbf{S-POP} &
  0.04944 &
  0.11934 &
  0.14922 &
  0.17604 &
  0.18762 &
  0.04944 &
  0.07971 &
  0.08661 &
  0.0903 &
  0.09115 \\
\textbf{AR} &
  0.0137 &
  0.03007 &
  0.03953 &
  0.0523 &
  0.05236 &
  0.0137 &
  0.02075 &
  0.0229 &
  0.02467 &
  0.02468 \\
\textbf{SR} &
  0.01354 &
  0.02732 &
  0.03508 &
  0.0479 &
  0.06099 &
  0.01354 &
  0.01936 &
  0.02112 &
  0.02282 &
  0.02373 \\
\textbf{VSKNN} &
  0.04108 & 0.05073 & 0.05379 & 0.07906 & 0.08772 & 0.03872 & 0.04251 & 0.04978 & 0.05184 & 0.04779 \\
\textbf{SMF} &
  0.01158 &
  0.03058 &
  0.04245 &
  0.06187 &
  0.08346 &
  0.01158 &
  0.01966 &
  0.02233 &
  0.02491 &
  0.0264 \\
\textbf{Item2Vec} &
  0.00271 &
  0.00611 &
  0.00888 &
  0.01411 &
  0.02235 &
  0.00271 &
  0.00413 &
  0.00476 &
  0.00546 &
  0.00601 \\
\textbf{GRU4Rec+} &
  0.02142 &
  0.05197 &
  0.07113 &
  0.09992 &
  0.12914 &
  0.02142 &
  0.03463 &
  0.039 &
  0.04283 &
  0.04485 \\
\textbf{NARM} &
  0.03018 &
  0.07757 &
  0.10832 &
  0.14692 &
  0.21896 &
  0.03018 &
  0.05063 &
  0.05763 &
  0.06265 &
  0.06697 \\
\textbf{STAMP} &
  0.03028 &
  0.06364 &
  0.08182 &
  0.10863 &
  0.1373 &
  0.03028 &
  0.04474 &
  0.04888 &
  0.05243 &
  0.0544 \\
\textbf{NextItNet} &
  0.0135 &
  0.02656 &
  0.03492 &
  0.04842 &
  0.06529 &
  0.0135 &
  0.019 &
  0.02088 &
  0.0227 &
  0.02384 \\
\textbf{SRGNN} &
  0.03824 &
  0.07338 &
  0.09248 &
  0.12116 &
  0.15297 &
  0.03824 &
  0.05339 &
  0.05774 &
  0.06157 &
  0.06376 \\
\textbf{CSRM} &
  0.02538 &
  0.05672 &
  0.07502 &
  0.10369 &
  0.13509 &
  0.02538 &
  0.03883 &
  0.04301 &
  0.04683 &
  0.04899 \\ \hline
\cellcolor[HTML]{333333}{\color[HTML]{FFFFFF} } &
  \multicolumn{5}{c|}{\textbf{HR@}} &
  \multicolumn{5}{c|}{\textbf{MRR@}} \\ \cline{2-11} 
\multirow{-2}{*}{\cellcolor[HTML]{333333}{\color[HTML]{FFFFFF} \textbf{ROCKET}}} &
  \textbf{1} &
  \textbf{3} &
  \textbf{5} &
  \textbf{10} &
  \textbf{20} &
  \textbf{1} &
  \textbf{3} &
  \textbf{5} &
  \textbf{10} &
  \textbf{20} \\ \hline
\textbf{S-POP} &
  0.05125 &
  0.12874 &
  0.14063 &
  0.14719 &
  0.15539 &
  0.05125 &
  0.08747 &
  0.09026 &
  0.0912 &
  0.09182 \\
\textbf{AR} &
  0.04469 &
  0.08528 &
  0.10742 &
  0.13284 &
  0.13284 &
  0.04469 &
  0.06218 &
  0.06721 &
  0.0707 &
  0.0707 \\
\textbf{SR} &
  0.04182 &
  0.07585 &
  0.09594 &
  0.11972 &
  0.13325 &
  0.04182 &
  0.05617 &
  0.06082 &
  0.06412 &
  0.06504 \\
\textbf{VSKNN} &
  0.16911 & 0.24948 & 0.27547 & 0.30834 & 0.33254 & 0.16911 & 0.20536 & 0.21138 & 0.21585 & 0.21757 \\
\textbf{SMF} &
  0.03772 &
  0.09512 &
  0.13243 &
  0.18901 &
  0.24887 &
  0.03772 &
  0.06225 &
  0.0707 &
  0.07815 &
  0.0824 \\
\textbf{Item2Vec} &
  0.01607 &
  0.04061 &
  0.05499 &
  0.07783 &
  0.11929 &
  0.01607 &
  0.02686 &
  0.03003 &
  0.03304 &
  0.036 \\
\textbf{GRU4Rec+} &
  0.03333 &
  0.07631 &
  0.09799 &
  0.13253 &
  0.16787 &
  0.03333 &
  0.05214 &
  0.05702 &
  0.06145 &
  0.06386 \\
\textbf{NARM} &
  0.06735 &
  0.11318 &
  0.14916 &
  0.19573 &
  0.27188 &
  0.06735 &
  0.08663 &
  0.09476 &
  0.10073 &
  0.10508 \\
\textbf{STAMP} &
  0.04299 &
  0.08433 &
  0.11451 &
  0.1542 &
  0.2038 &
  0.04299 &
  0.06104 &
  0.06793 &
  0.07307 &
  0.07652 \\
\textbf{NextItNet} &
  0.02832 &
  0.04297 &
  0.05273 &
  0.07129 &
  0.09375 &
  0.02832 &
  0.03516 &
  0.0375 &
  0.03987 &
  0.0413 \\
\textbf{SRGNN} &
  0.06094 &
  0.11016 &
  0.13945 &
  0.18164 &
  0.22344 &
  0.06094 &
  0.08197 &
  0.0888 &
  0.09464 &
  0.09747 \\
\textbf{CSRM} &
  0.05628 &
  0.11378 &
  0.14886 &
  0.19902 &
  0.24674 &
  0.05628 &
  0.08109 &
  0.08908 &
  0.09573 &
  0.09894 \\ \hline
\end{tabular}}
\label{tab:recency-old}
\end{table*}
