# Supplementary material for: Comprehensive Empirical Evaluation of Deep Learning Approaches for Session-based Recommendation in E-Commerce
Source: arXiv:2010.12540 source file (2020-10-17)
Supplement: Supplementary file 21 [file tab9.tex]

% Please add the following required packages to your document preamble:
% \usepackage{multirow}
% \usepackage[table,xcdraw]{xcolor}
% If you use beamer only pass "xcolor=table" option, i.e. \documentclass[xcolor=table]{beamer}
\begin{table*}[!h]
\centering
\caption{RQ4: Training using a mixture between the most recent 5(10) days and the eldest 5(10) days in the training set for RECSYS, CIKMCUP, TMall, and (ROCKET) datasets.}
\resizebox{0.9\textwidth}{!}{\begin{tabular}{|c|ccccc|ccccc|}
\hline
\cellcolor[HTML]{333333}{\color[HTML]{FFFFFF} } &
  \multicolumn{5}{c|}{\textbf{HR@}} &
  \multicolumn{5}{c|}{\textbf{MRR@}} \\ \cline{2-11} 
\multirow{-2}{*}{\cellcolor[HTML]{333333}{\color[HTML]{FFFFFF} \textbf{RECSYS}}} &
  \textbf{1} &
  \textbf{3} &
  \textbf{5} &
  \textbf{10} &
  \textbf{20} &
  \textbf{1} &
  \textbf{3} &
  \textbf{5} &
  \textbf{10} &
  \textbf{20} \\ \hline
\textbf{S-POP} &
  0.03645 &
  0.0997 &
  0.12352 &
  0.14468 &
  0.15449 &
  0.03645 &
  0.06416 &
  0.06964 &
  0.07256 &
  0.07328 \\
\textbf{AR} &
  0.1142 &
  0.22309 &
  0.28489 &
  0.35159 &
  0.35163 &
  0.1142 &
  0.16122 &
  0.17524 &
  0.18476 &
  0.18476 \\
\textbf{SR} &
  0.1163 &
  0.22639 &
  0.28927 &
  0.38188 &
  0.47596 &
  0.1163 &
  0.16403 &
  0.1783 &
  0.19069 &
  0.19721 \\
\textbf{VSKNN} &
  0.11120 & 0.19876 & 0.24997 & 0.30103 & 0.36255 & 0.09493 & 0.14982 & 0.15719 & 0.15204 & 0.16442 \\
\textbf{SMF} &
  0.06817 &
  0.19971 &
  0.29022 &
  0.43308 &
  0.56207 &
  0.06817 &
  0.12372 &
  0.14433 &
  0.16335 &
  0.17241 \\
\textbf{Item2Vec} &
  0.07749 &
  0.1551 &
  0.2049 &
  0.28104 &
  0.36868 &
  0.07749 &
  0.11131 &
  0.12256 &
  0.13265 &
  0.13862 \\
\textbf{GRU4Rec+} &
  0.09028 &
  0.19609 &
  0.27605 &
  0.40226 &
  0.53275 &
  0.09028 &
  0.13502 &
  0.15316 &
  0.16995 &
  0.17906 \\
\textbf{NARM} &
  0.1125 &
  0.26714 &
  0.36731 &
  0.51003 &
  0.69546 &
  0.1125 &
  0.17921 &
  0.20211 &
  0.22124 &
  0.23269 \\
\textbf{STAMP} &
  0.13102 &
  0.26197 &
  0.3436 &
  0.46573 &
  0.5863 &
  0.13102 &
  0.1872 &
  0.20582 &
  0.22213 &
  0.23055 \\
\textbf{NextItNet} &
  0.17973 &
  0.33756 &
  0.41825 &
  0.52521 &
  0.62326 &
  0.17973 &
  0.24818 &
  0.26655 &
  0.28102 &
  0.28787 \\
\textbf{SRGNN} &
  0.14046 &
  0.28276 &
  0.36916 &
  0.49403 &
  0.61603 &
  0.14046 &
  0.20182 &
  0.22149 &
  0.23828 &
  0.24679 \\
\textbf{CSRM} &
  0.16558 &
  0.32565 &
  0.41225 &
  0.54721 &
  0.66871 &
  0.16558 &
  0.23502 &
  0.25472 &
  0.27273 &
  0.28126 \\ \hline
\cellcolor[HTML]{333333}{\color[HTML]{FFFFFF} } &
  \multicolumn{5}{c|}{\textbf{HR@}} &
  \multicolumn{5}{c|}{\textbf{MRR@}} \\ \cline{2-11} 
\multirow{-2}{*}{\cellcolor[HTML]{333333}{\color[HTML]{FFFFFF} \textbf{CIKMCUP}}} &
  \textbf{1} &
  \textbf{3} &
  \textbf{5} &
  \textbf{10} &
  \textbf{20} &
  \textbf{1} &
  \textbf{3} &
  \textbf{5} &
  \textbf{10} &
  \textbf{20} \\ \hline
\textbf{S-POP} &
  0.03839 &
  0.10434 &
  0.12213 &
  0.13458 &
  0.14006 &
  0.03839 &
  0.06746 &
  0.07153 &
  0.07331 &
  0.07371 \\
\textbf{AR} &
  0.03794 &
  0.09071 &
  0.12539 &
  0.16926 &
  0.16941 &
  0.03794 &
  0.06067 &
  0.0685 &
  0.07456 &
  0.07457 \\
\textbf{SR} &
  0.03705 &
  0.07396 &
  0.09827 &
  0.14125 &
  0.17919 &
  0.03705 &
  0.05284 &
  0.05832 &
  0.06404 &
  0.06669 \\
\textbf{VSKNN} &
  0.06581 & 0.13016 & 0.17319 & 0.22169 & 0.27272 & 0.06581 & 0.09353 & 0.10340 & 0.10984 & 0.11343 \\
\textbf{SMF} &
  0.04027 &
  0.09667 &
  0.13678 &
  0.21867 &
  0.31775 &
  0.04027 &
  0.06382 &
  0.07295 &
  0.08371 &
  0.09051 \\
\textbf{Item2Vec} &
  0.02158 &
  0.04966 &
  0.07049 &
  0.11336 &
  0.1766 &
  0.02158 &
  0.03358 &
  0.03827 &
  0.04397 &
  0.04834 \\
\textbf{GRU4Rec+} &
  0.02326 &
  0.05589 &
  0.08018 &
  0.12231 &
  0.17001 &
  0.02326 &
  0.03706 &
  0.0426 &
  0.04814 &
  0.0514 \\
\textbf{NARM} &
  0.03364 &
  0.1011 &
  0.14965 &
  0.23336 &
  0.38111 &
  0.03364 &
  0.06214 &
  0.07337 &
  0.08436 &
  0.09295 \\
\textbf{STAMP} &
  0.02683 &
  0.06448 &
  0.09635 &
  0.1515 &
  0.22132 &
  0.02683 &
  0.04267 &
  0.04977 &
  0.05702 &
  0.06193 \\
\textbf{NextItNet} &
  0.00469 &
  0.01302 &
  0.01979 &
  0.03698 &
  0.05729 &
  0.00469 &
  0.00816 &
  0.00967 &
  0.01184 &
  0.0133 \\
\textbf{SRGNN} &
  0.03641 &
  0.1023 &
  0.14298 &
  0.21094 &
  0.28641 &
  0.03641 &
  0.06454 &
  0.07383 &
  0.08284 &
  0.08807 \\
\textbf{CSRM} &
  0.03857 &
  0.09657 &
  0.13633 &
  0.20991 &
  0.29491 &
  0.03857 &
  0.06339 &
  0.07246 &
  0.08208 &
  0.08791 \\ \hline
\cellcolor[HTML]{333333}{\color[HTML]{FFFFFF} } &
  \multicolumn{5}{c|}{\textbf{HR@}} &
  \multicolumn{5}{c|}{\textbf{MRR@}} \\ \cline{2-11} 
\multirow{-2}{*}{\cellcolor[HTML]{333333}{\color[HTML]{FFFFFF} \textbf{TMALL}}} &
  \textbf{1} &
  \textbf{3} &
  \textbf{5} &
  \textbf{10} &
  \textbf{20} &
  \textbf{1} &
  \textbf{3} &
  \textbf{5} &
  \textbf{10} &
  \textbf{20} \\ \hline
\textbf{S-POP} &
  0.046 &
  0.10521 &
  0.1345 &
  0.1667 &
  0.18649 &
  0.046 &
  0.07164 &
  0.07834 &
  0.08272 &
  0.08413 \\
\textbf{AR} &
  0.01305 &
  0.02837 &
  0.03737 &
  0.04993 &
  0.05007 &
  0.01305 &
  0.01968 &
  0.02173 &
  0.02349 &
  0.02349 \\
\textbf{SR} &
  0.01248 &
  0.02637 &
  0.03458 &
  0.04692 &
  0.06102 &
  0.01248 &
  0.01847 &
  0.02033 &
  0.02195 &
  0.02293 \\
\textbf{VSKNN} &
  0.02649 & 0.05548 & 0.05775 & 0.06740 & 0.08883 & 0.03116 & 0.03902 & 0.04004 & 0.03935 & 0.04467 \\
\textbf{SMF} &
  0.01387 &
  0.03639 &
  0.05225 &
  0.07809 &
  0.10966 &
  0.01387 &
  0.02342 &
  0.027 &
  0.03044 &
  0.03262 \\
\textbf{Item2Vec} &
  0.00216 &
  0.00512 &
  0.00711 &
  0.01121 &
  0.01781 &
  0.00216 &
  0.00341 &
  0.00386 &
  0.0044 &
  0.00485 \\
\textbf{GRU4Rec+} &
  0.02066 &
  0.04896 &
  0.06656 &
  0.09472 &
  0.12331 &
  0.02066 &
  0.0328 &
  0.03681 &
  0.04061 &
  0.04258 \\
\textbf{NARM} &
  0.02599 &
  0.07346 &
  0.10293 &
  0.1486 &
  0.22854 &
  0.02599 &
  0.04633 &
  0.0533 &
  0.05958 &
  0.06446 \\
\textbf{STAMP} &
  0.03034 &
  0.06202 &
  0.08124 &
  0.11303 &
  0.14747 &
  0.03034 &
  0.04398 &
  0.04835 &
  0.05256 &
  0.05495 \\
\textbf{NextItNet} &
  0.02021 &
  0.03737 &
  0.04622 &
  0.0601 &
  0.07976 &
  0.02021 &
  0.02759 &
  0.02962 &
  0.03145 &
  0.03278 \\
\textbf{SRGNN} &
  0.03545 &
  0.07001 &
  0.09067 &
  0.12145 &
  0.15635 &
  0.03545 &
  0.05039 &
  0.05508 &
  0.05917 &
  0.06158 \\
\textbf{CSRM} &
  0.02535 &
  0.05574 &
  0.07436 &
  0.10477 &
  0.1398 &
  0.02535 &
  0.03843 &
  0.04267 &
  0.0467 &
  0.0491 \\ \hline
\cellcolor[HTML]{333333}{\color[HTML]{FFFFFF} } &
  \multicolumn{5}{c|}{\textbf{HR@}} &
  \multicolumn{5}{c|}{\textbf{MRR@}} \\ \cline{2-11} 
\multirow{-2}{*}{\cellcolor[HTML]{333333}{\color[HTML]{FFFFFF} \textbf{ROCKET}}} &
  \textbf{1} &
  \textbf{3} &
  \textbf{5} &
  \textbf{10} &
  \textbf{20} &
  \textbf{1} &
  \textbf{3} &
  \textbf{5} &
  \textbf{10} &
  \textbf{20} \\ \hline
\textbf{S-POP} &
  0.03984 &
  0.11554 &
  0.13015 &
  0.1421 &
  0.15193 &
  0.03984 &
  0.0741 &
  0.07752 &
  0.07921 &
  0.0799 \\
\textbf{AR} &
  0.05232 &
  0.09987 &
  0.12696 &
  0.15697 &
  0.15777 &
  0.05232 &
  0.07291 &
  0.07907 &
  0.08337 &
  0.08343 \\
\textbf{SR} &
  0.05046 &
  0.09163 &
  0.11262 &
  0.14343 &
  0.16016 &
  0.05046 &
  0.06826 &
  0.07304 &
  0.07729 &
  0.0785 \\
\textbf{VSKNN} &
  0.13399 & 0.21085 & 0.23572 & 0.26921 & 0.29203 & 0.13399 & 0.16814 & 0.17384 & 0.17841 & 0.17996 \\
\textbf{SMF} &
  0.04648 &
  0.10757 &
  0.14927 &
  0.20478 &
  0.26614 &
  0.04648 &
  0.0722 &
  0.08176 &
  0.08919 &
  0.09337 \\
\textbf{Item2Vec} &
  0.02744 &
  0.0546 &
  0.06764 &
  0.09264 &
  0.12171 &
  0.02744 &
  0.03903 &
  0.04191 &
  0.04529 &
  0.04733 \\
\textbf{GRU4Rec+} &
  0.0386 &
  0.07694 &
  0.10153 &
  0.13221 &
  0.16499 &
  0.0386 &
  0.05531 &
  0.06085 &
  0.06506 &
  0.06727 \\
\textbf{NARM} &
  0.07582 &
  0.15037 &
  0.19233 &
  0.24099 &
  0.31707 &
  0.07582 &
  0.10837 &
  0.11792 &
  0.12464 &
  0.1291 \\
\textbf{STAMP} &
  0.04218 &
  0.07982 &
  0.11052 &
  0.15109 &
  0.19301 &
  0.04218 &
  0.05833 &
  0.06546 &
  0.07081 &
  0.07373 \\
\textbf{NextItNet} &
  0.0277 &
  0.05327 &
  0.07173 &
  0.09517 &
  0.12145 &
  0.0277 &
  0.03918 &
  0.04319 &
  0.0465 &
  0.04818 \\
\textbf{SRGNN} &
  0.05286 &
  0.1138 &
  0.14271 &
  0.18307 &
  0.21927 &
  0.05286 &
  0.07938 &
  0.0861 &
  0.0915 &
  0.09406 \\
\textbf{CSRM} &
  0.05896 &
  0.12797 &
  0.16869 &
  0.2192 &
  0.27287 &
  0.05896 &
  0.08761 &
  0.09692 &
  0.10365 &
  0.10733 \\ \hline
\end{tabular}}
\label{tab:recency-mix}
\end{table*}
